# Supplementary material for: Understanding out-of-distribution accuracies through quantifying difficulty of test samples
Source: arXiv:2203.15100 source file (2022-03-28)
Supplement: Supplementary file 1 [file appendix.tex]

% \documentclass{article}
% \usepackage[top=1in, bottom=1in, left=1in, right=1in]{geometry}
% \usepackage{graphicx, subfig}
% \usepackage{wrapfig}
% \usepackage{booktabs}
% \usepackage{amsmath, amsthm, amssymb}
% \usepackage{array}
% \usepackage{nicefrac}
% \usepackage{bbm}
% \usepackage{wrapfig}

% \usepackage[dvipsnames]{xcolor}

% \usepackage{hyperref}
% \usepackage{appendix}

% \usepackage{natbib}
% %\addbibresource{references.bib}

% \input{preamble.tex}

% \title{What make the OOD accuracies drop? An entropy-based image difficulty analysis} %[ICLR 2021] OOD-OP
% \author{Berfin \c{S}im\c{s}ek, St\'ephane D'Ascoli, Levent Sagun}
% %\author{Berfin \c{S}im\c{s}ek*, St\'ephane D'Ascoli*, Levent Sagun}
% \date{}

% \begin{document}

\appendix

\section{The prediction performance of alternative entropy scores}

\subsection{Resnet101s with different complexity (with early stopping)}

We use the entropy scores calculated from 10 resnet101s but by controlling the network complexity by choosing the epoch from which to collect class conditional probabilities. In our experiments resnet101s achieve the best test accuracy on the CIFAR10 test data in between epochs 150-200. 

\begin{figure}[ht!]
   \begin{center}
    \includegraphics[width=0.9\textwidth]{figs/01OOD-acc-preds-epoch10.png} 
    \includegraphics[width=0.9\textwidth]{figs/01OOD-acc-preds-epoch50.png} 
    \includegraphics[width=0.9\textwidth]{figs/01OOD-acc-preds-epoch200.png} 
   \end{center}
  \vspace{-0.3cm}
  \caption{\label{fig:appendix-OOD-acc-pred} Predicting the OOD accuracies using entropy partions of the probabilities predicted from resnet101 at epoch 10, epoch 50, and epoch 200 respectively. We observe that the epoch 10 resnet101's are good at predicting the performance of small feedforward networks but the predictions are pessimistic for high-performing models whereas epoch 50 or epoch 200 probabilities are poor at predicting the performance of small networks. We obtain the best performance in predicting OOD accuracies by averaging the entropies of all epochs as described in the main text.}
 \end{figure}

We calculated the entropy scores using the network predictions of the first 10 epochs with 40 resnets of (10 seeds of resnet18, resnet34, resnet50, and resnet101). We show that entopy scores obtained by averaging over 200 epochs gives the similar results. TO-DO: decide on what is the best averaging stratgey i.e. how many epochs?

We show that the entopy scores obtained by converged lenets with optimal stopping (by peeking at the accuracy of the test data), and feedforward networks with optimal stopping are correlated with high scores suggesting that the entropy scores are a property of the datasets alone and shows limited dependence on the inductive biases of the chosen architecture. 

\subsection{Single Resnet101s without ensembling}

Why can't we rely on the predictions/dynamics of a single network to study image difficulty?

\section{Learning dynamics}

In literature, cite[...] explores a large variety of models to study image difficulty. In this section we will discuss these methods and the behavior of confusion groups during training.

\begin{figure}[ht!]
   \begin{center}
    \includegraphics[width=1\textwidth]{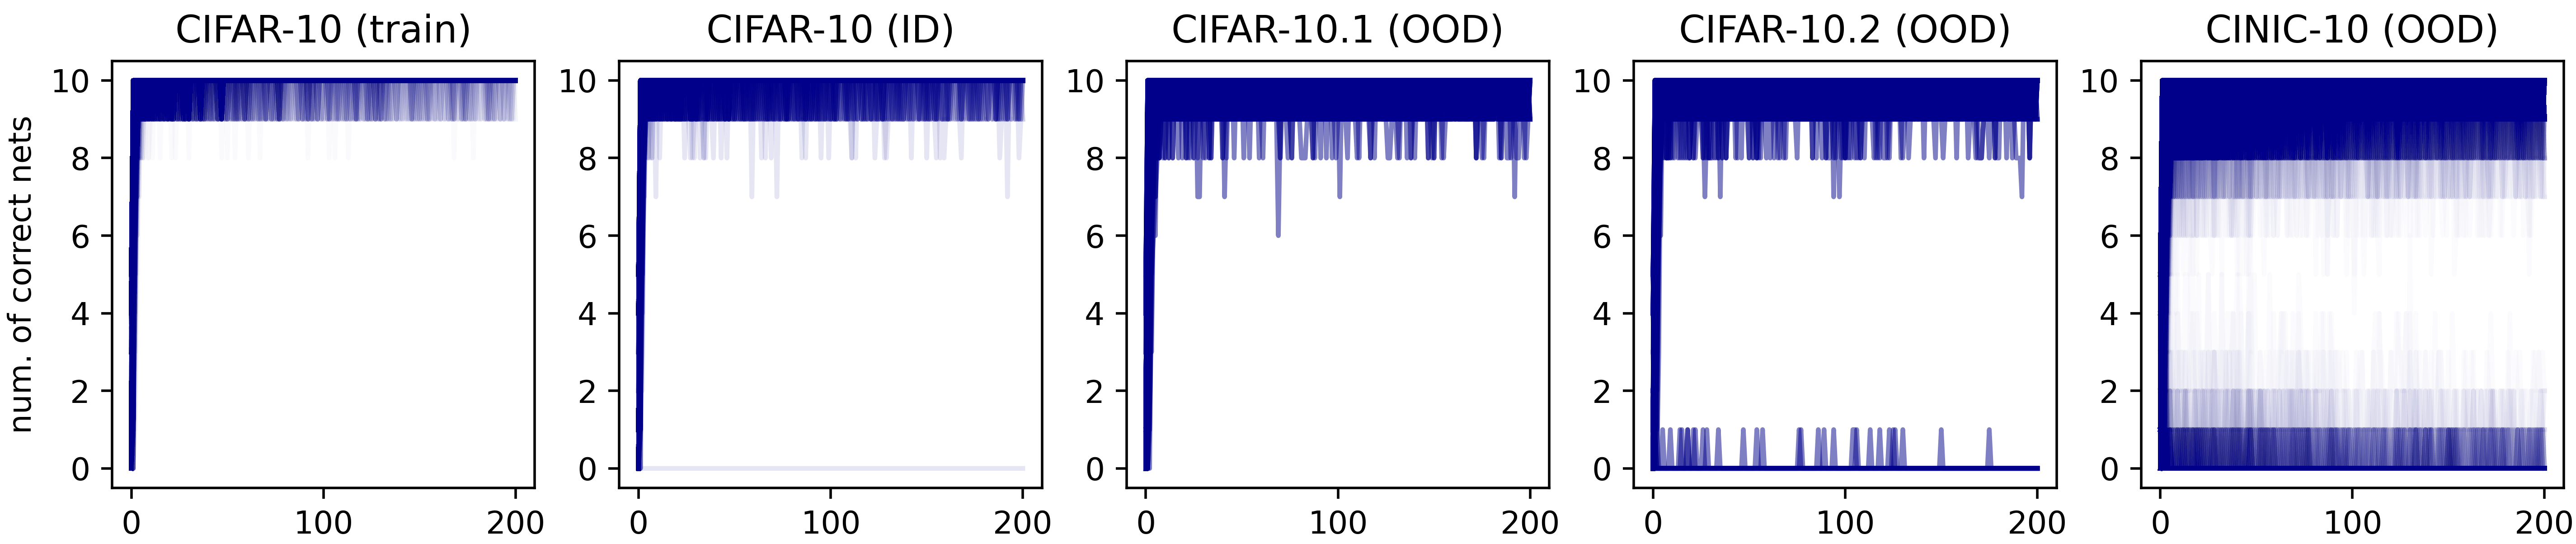} 
    \includegraphics[width=1\textwidth]{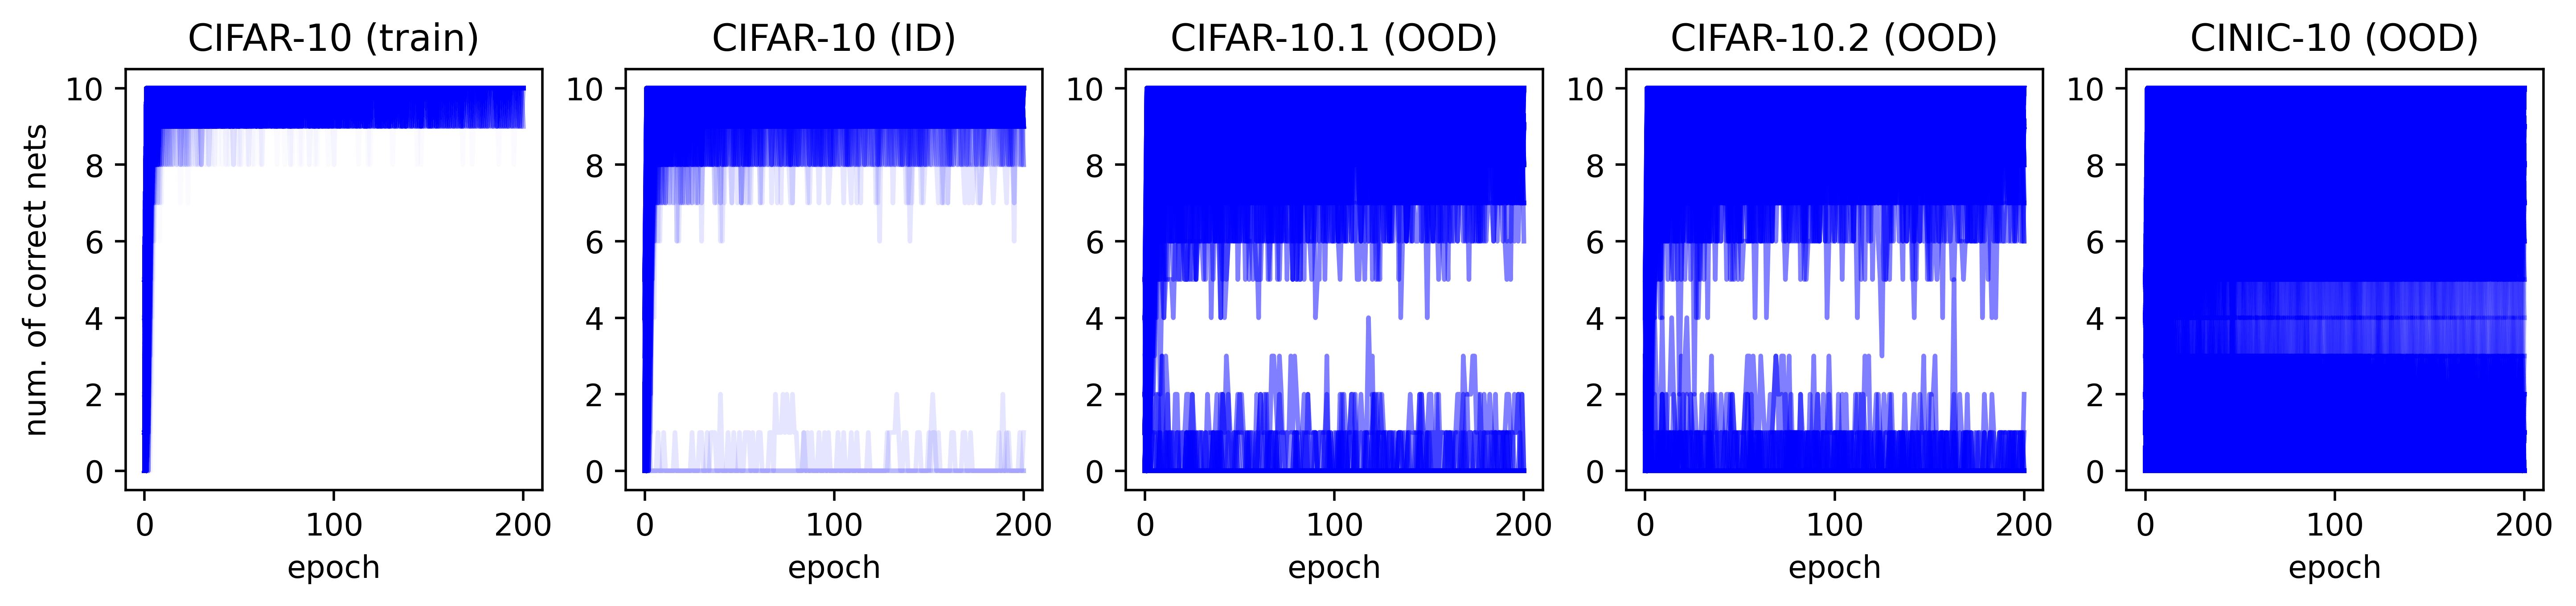} 
   \end{center}
  \vspace{-0.3cm}
  \caption{\label{fig:dynamics-per-group-app} We observe that the easy samples in the low entropy group are rarely forgotten and hard samples are rarely classified correctly. First row represents first fifth of the samples in the lowest entropy group, the second row represents the second fifth. In the other groups we do not see a separation between easy and hard examples which suggests that the networks keep learn and forget these samples in a cyclic fashion (except for the training data where we observe all the samples are learnt/memorized similar to the first two rows. But there are accidental mistakes (in easy samples) and accidental learning (in hard samples) due to the randomness coming from the initialization and learning algorithm (probably the order of which the samples are learnt matters the most).}
 \end{figure}

\section{Accuracy across confusion groups for various model families}

\begin{figure}[ht!]
   \begin{center}
    \includegraphics[width=1\textwidth]{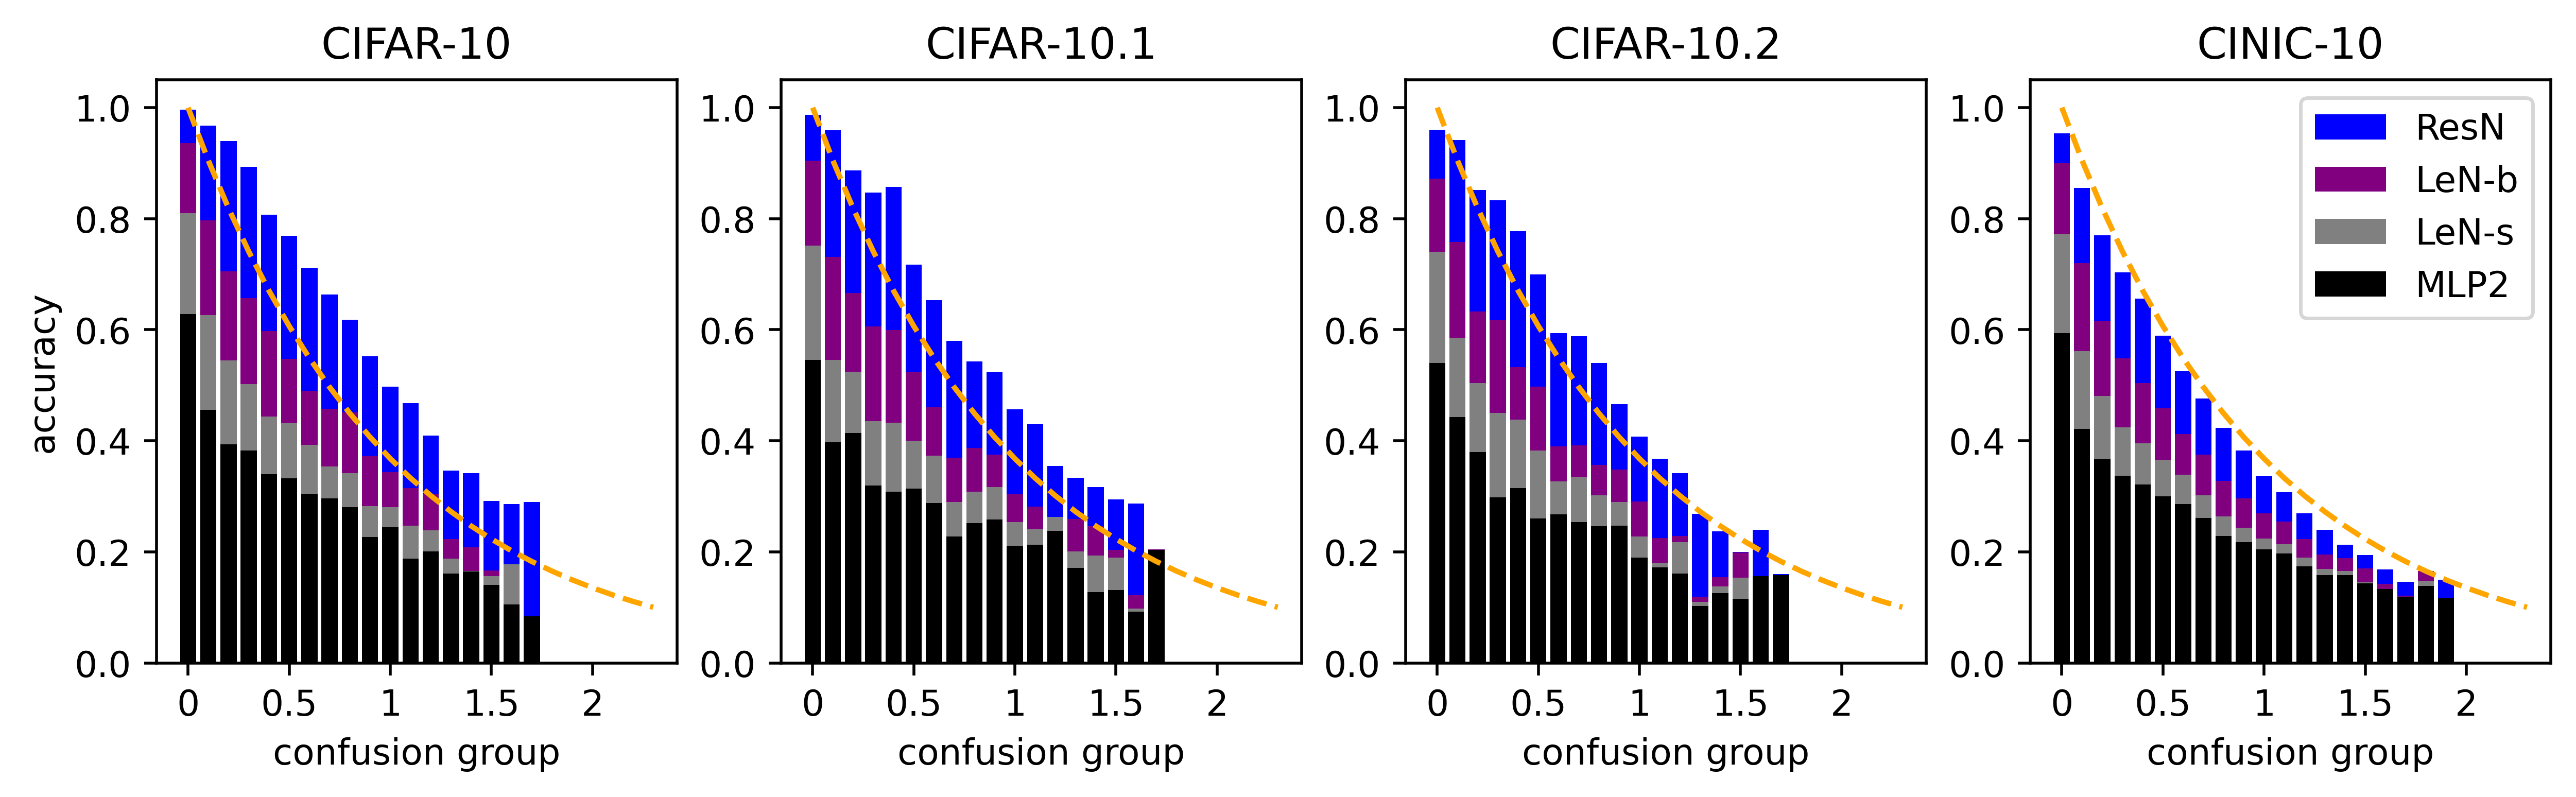} 
   \end{center}
  \vspace{-0.3cm}
  \caption{\label{fig:appendix-acc-per-group} We plot the average accuracies of (i) ResNets (10 resnet18s, 10 resnet34s, 10 resnet50s, and 10 resnet101s), (ii) big LeNets with the number of filters $(16, 32, 64, 128)$ in the first layer and our scaling scheme, (iii) small LeNets with the number of filters $(2, 4, 8)$ in the first layer and our scaling scheme, and (iv) two-layers networks with widths $(2,4,8,\ldots, 2014)$. We find that decreasing the model complexity hurts accuracies across subgroups in a structured way, i.e. drop in accuracy in each subgroup is homogenous. The orange line represents $ e^{-x}$  where $ x $ is the confusion score. Our preliminary observations suggest that the accuracy levels per group can be modeled with $ C^{(\alpha -1)} e^{-\alpha x}$ where $\alpha\in [0,1]$ represents the model complexity ($C$ is the number of classes): for $\alpha=1$ we have the orange line and where for $\alpha = 0$ we have the random model which is guessing randomly the correct class for each subgroup.}
 \end{figure}

\subsection{The effect of ensembling on confusion groups}

\begin{figure}[ht!]
   \begin{center}
    \includegraphics[width=1\textwidth]{figs/01acc-per-group-ens.png} 
   \end{center}
  \vspace{-0.3cm}
  \caption{\label{fig:appendix-acc-per-grou-ensp} We plot the average accuracies of (blue) ResNets (10 resnet18s, 10 resnet34s, 10 resnet50s, and 10 resnet101s)  and (green) is the gain in accuracy in their ensembles (the average accuracy of 4 ensembled networks).}
 \end{figure}

\section{The Representation Geometry}

\begin{figure}[t!]
   \begin{center}
   \includegraphics[width=0.995\textwidth]{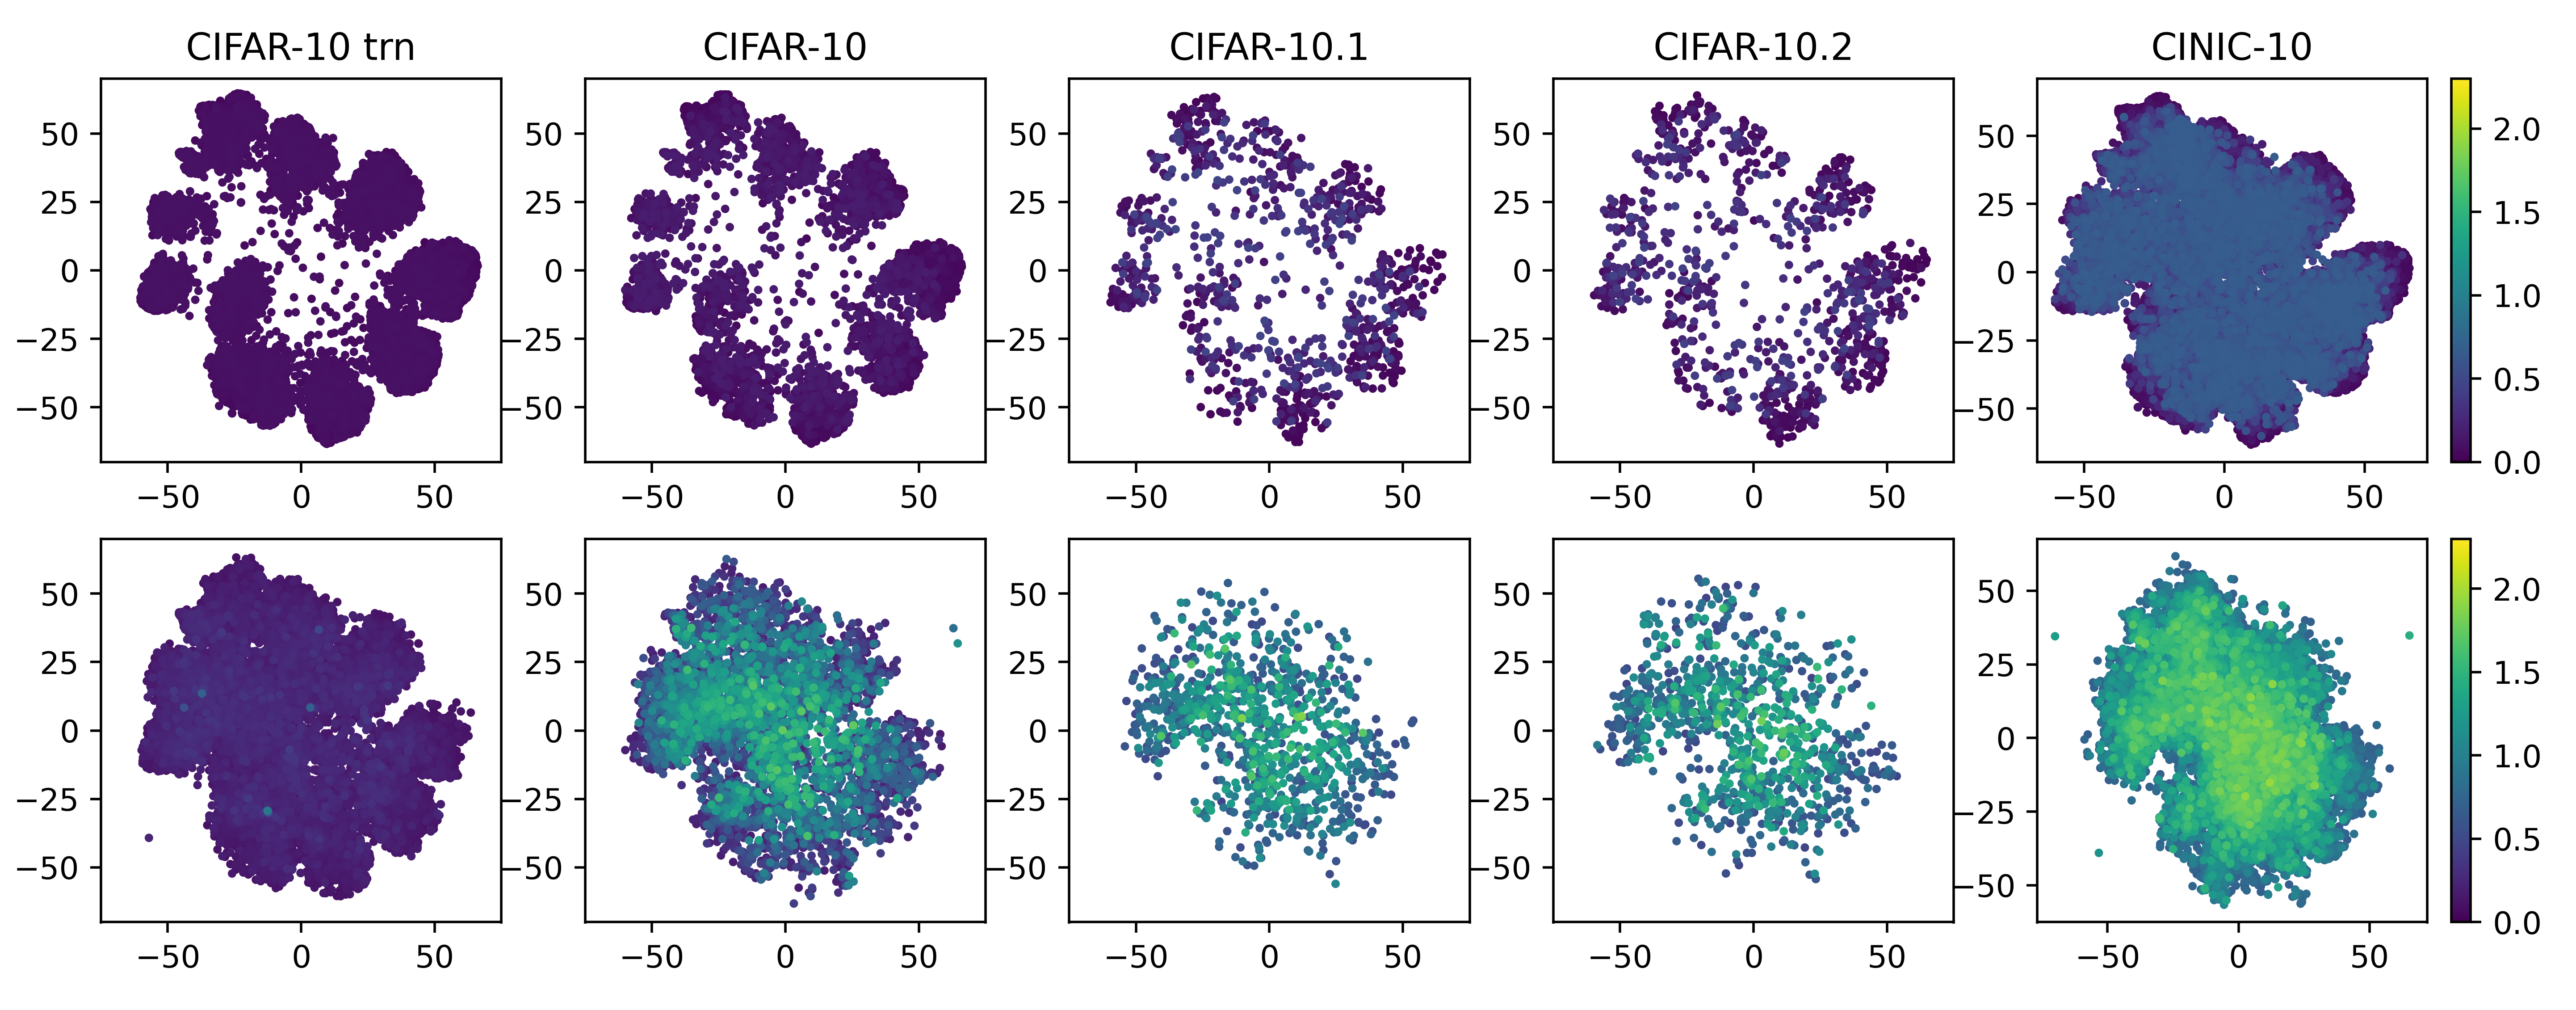} 
   \end{center}
  \vspace{-0.3cm}
  \caption{\label{fig:rep-geo-app} \textbf{TSNE visualizations of the data points in the representation space of a ResNet18: confusing (high entropy samples) are found 'in-between' low entropy clusters}. Low entropy ID and OOD samples are represented in the similar regions of the representation space. In the training data, we only have a few high entropy samples since (almost) all the data points are memorized during training in order to predict the class label. In the CINIC-10 dataset, we see a large amount of very high entropy samples (yellow points in the middle) that do not form clusters which indicates that they are farther apart from each other in the representation space.} 
\end{figure}

\begin{figure}[t!]
   \begin{center}
   \includegraphics[width=0.9\textwidth]{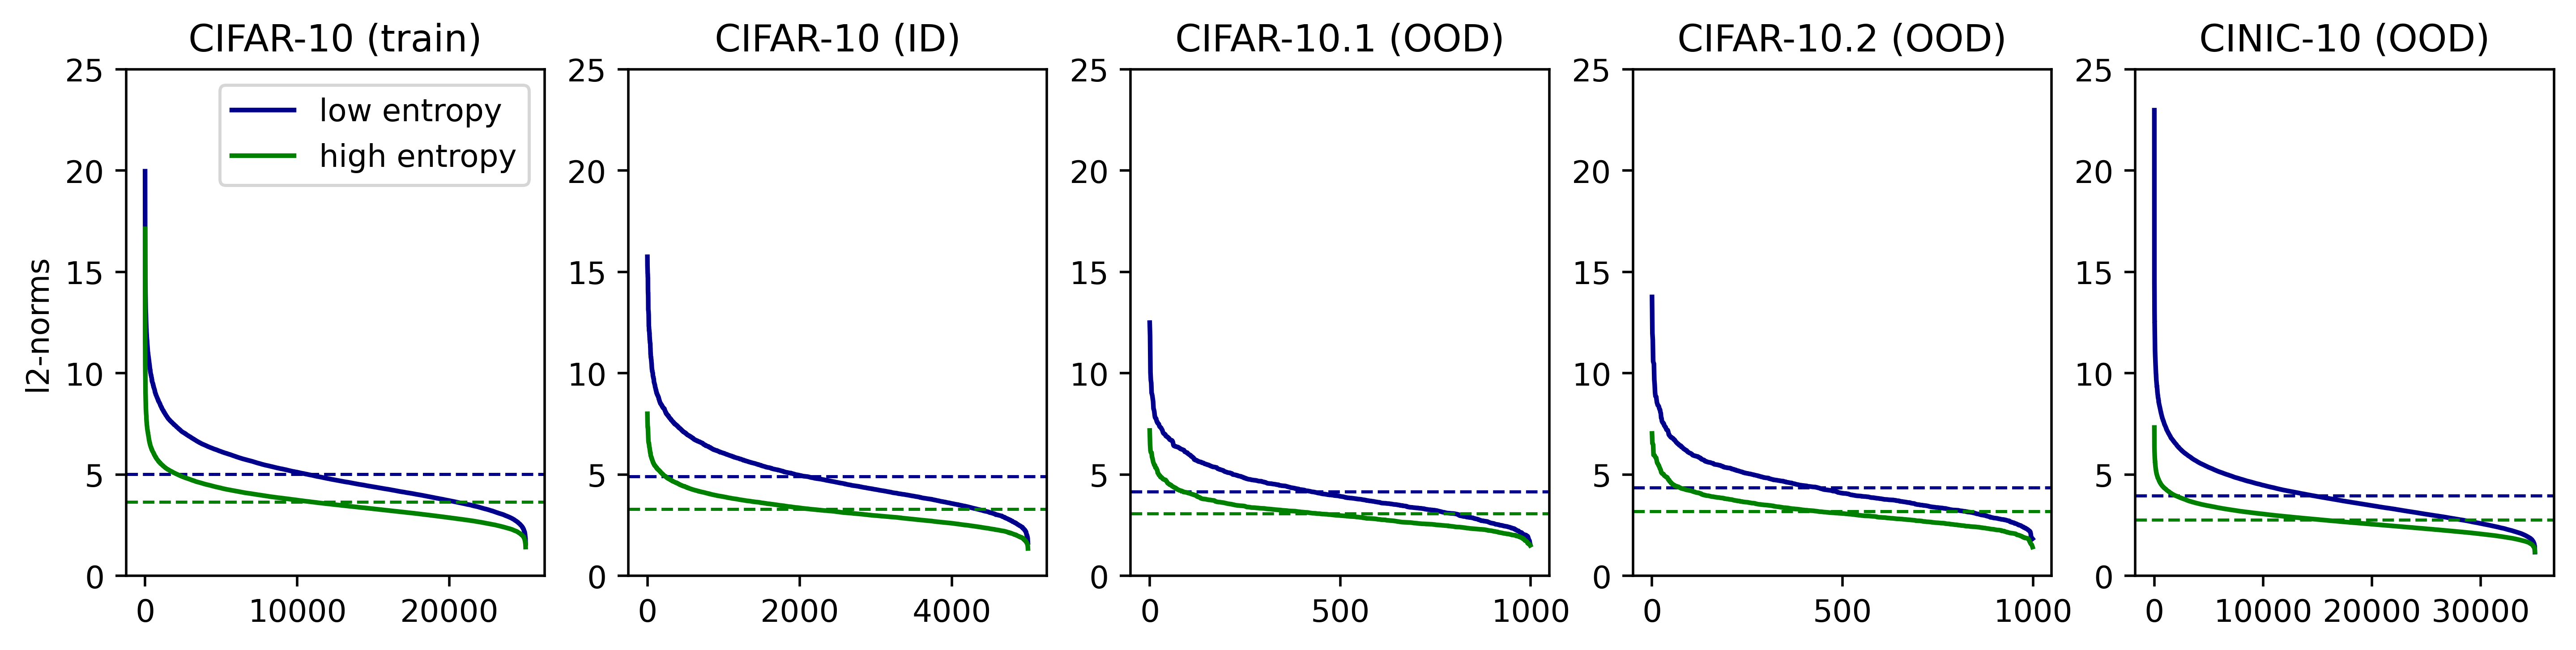} 
   \includegraphics[width=0.9\textwidth]{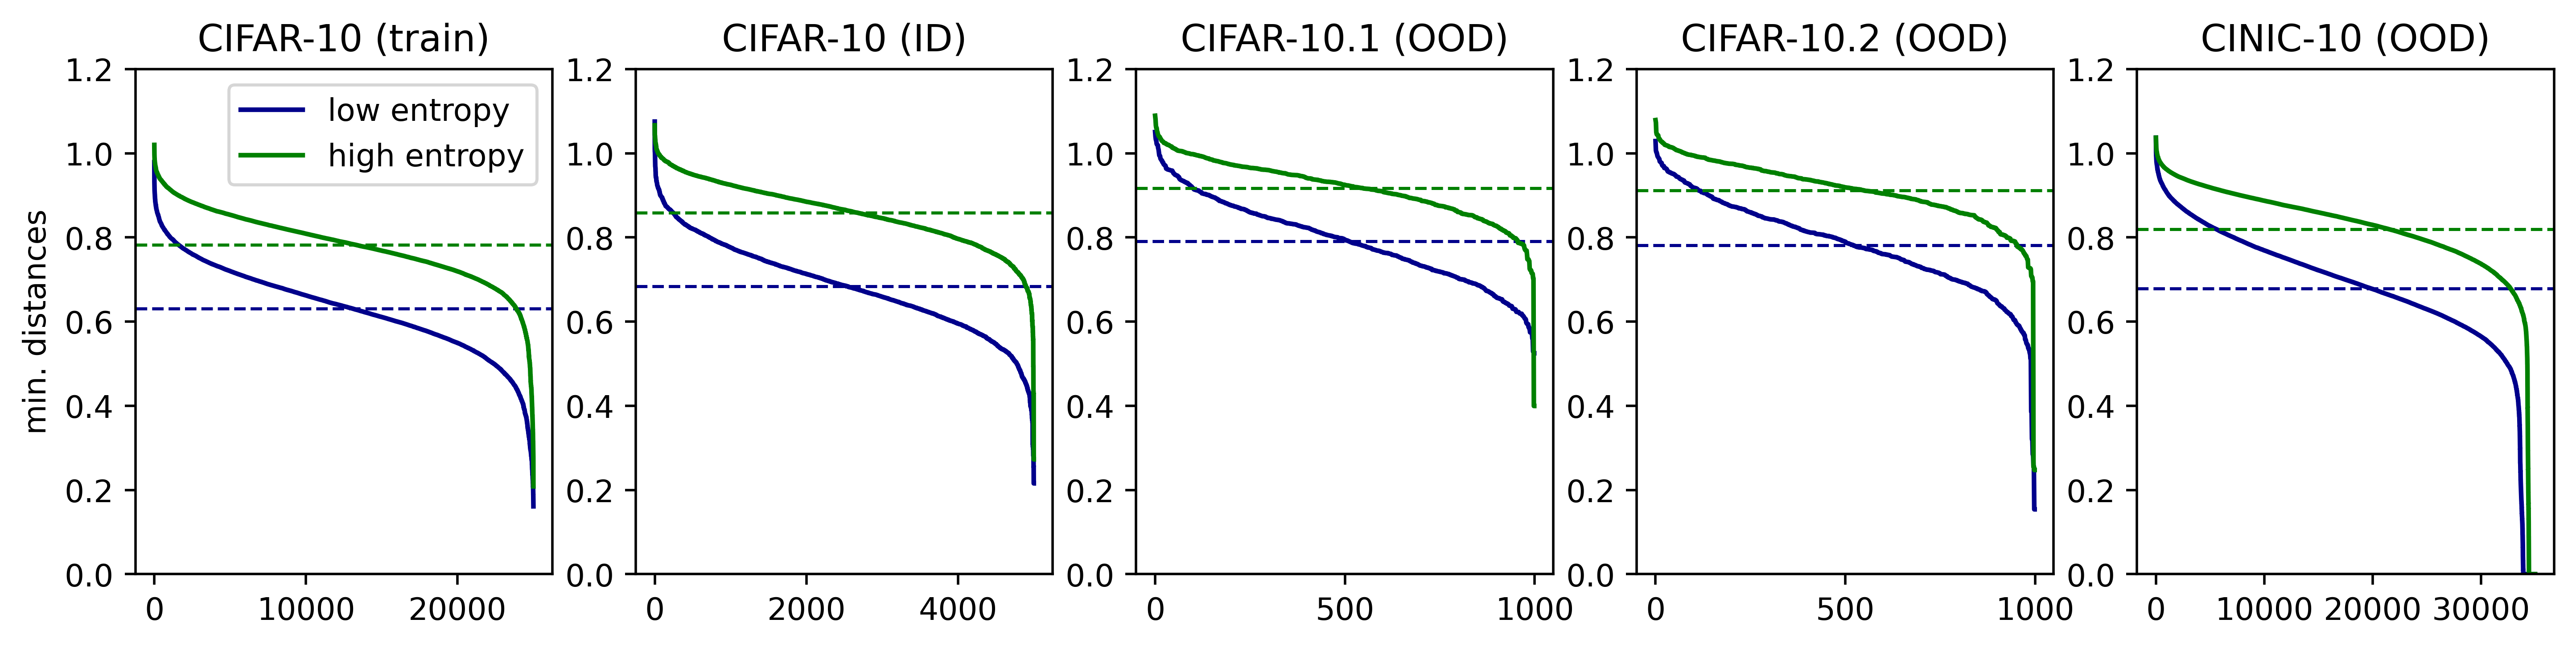} 
   \end{center}
  \vspace{-0.3cm}
  \caption{\label{fig:rep-geo-euc-app} \textbf{(Top) L2-norm of the data points in the representation space Bottom: }. Color represents the confusion score: dark colors represent low entropy samples whereas light color/yellow samples represent high entropy samples. ID and OOD samples are also represented in similar regions in the representation space.} 
\end{figure}

\begin{figure}[t!]
   \begin{center}
      \includegraphics[width=0.9\textwidth]{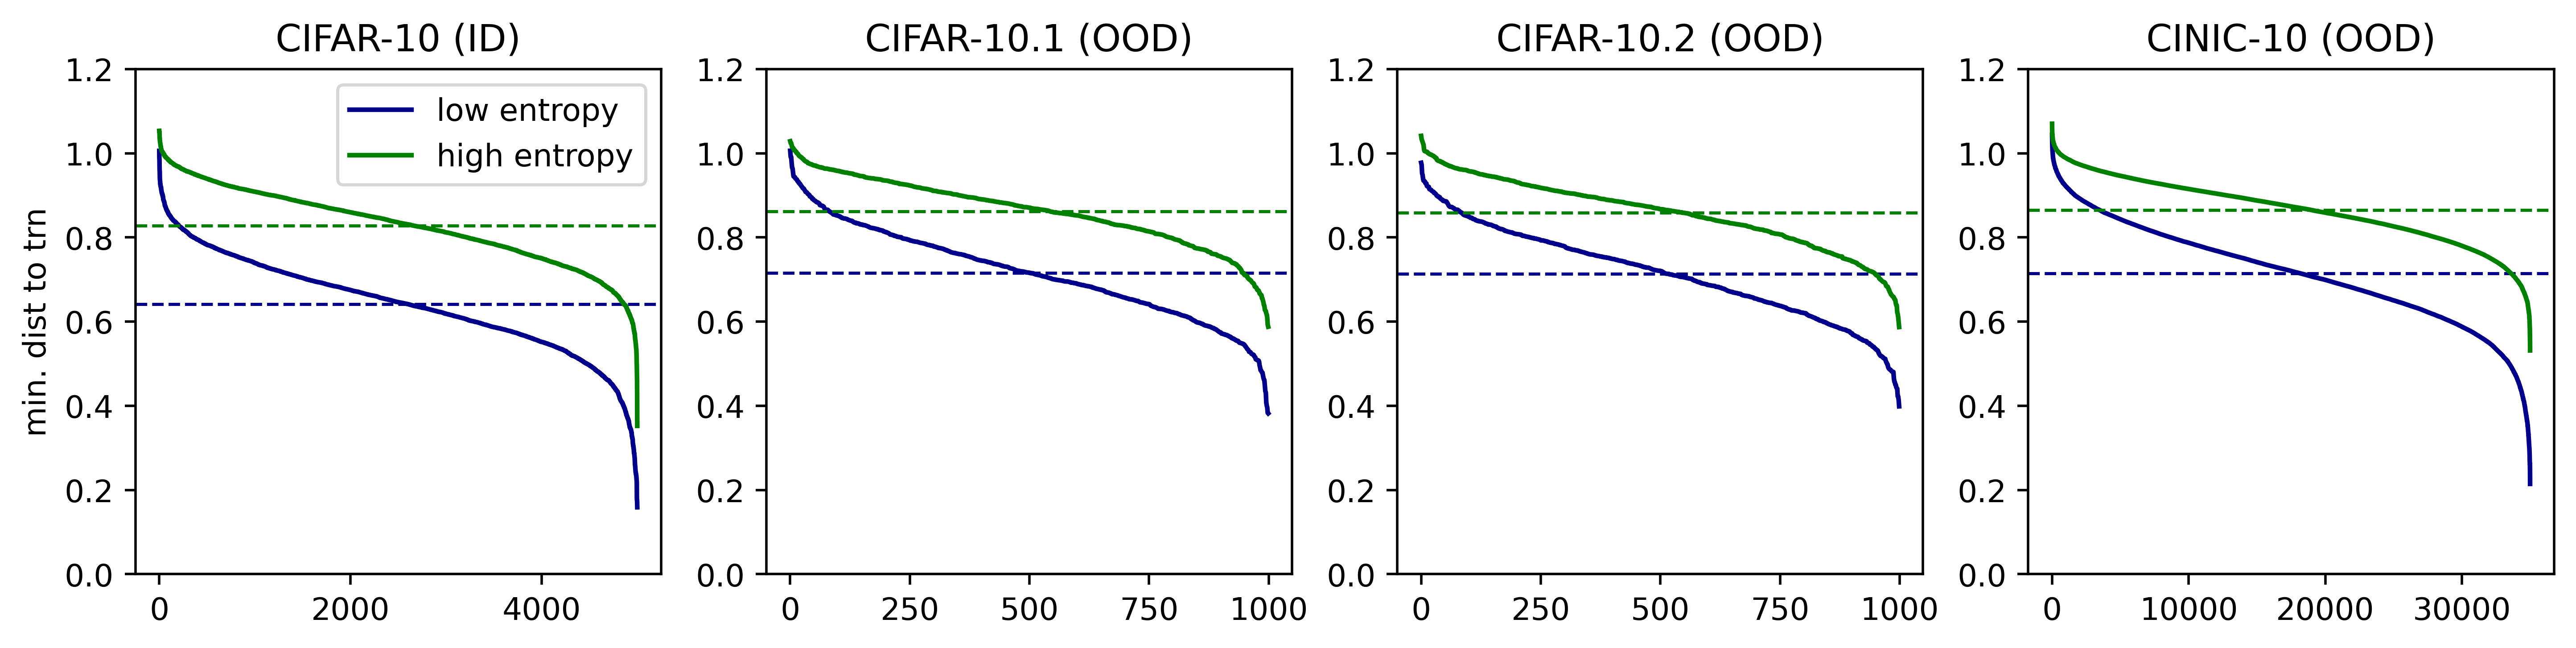} 
   \end{center}
  \vspace{-0.3cm}
  \caption{\label{fig:rep-geo-euc-app2} \textbf{Distance of the test samples to the low entropy population of the training dataset}. Color represents the confusion score: dark colors represent low entropy samples whereas light color/yellow samples represent high entropy samples. ID and OOD samples are also represented in similar regions in the representation space. See appendix for the visualization of all the datasets we considered.} 
\end{figure}

\section{Lowest \& Highest entropy images from each class}

\begin{figure}[t!]
   \begin{center}
   \includegraphics[width=0.48\textwidth]{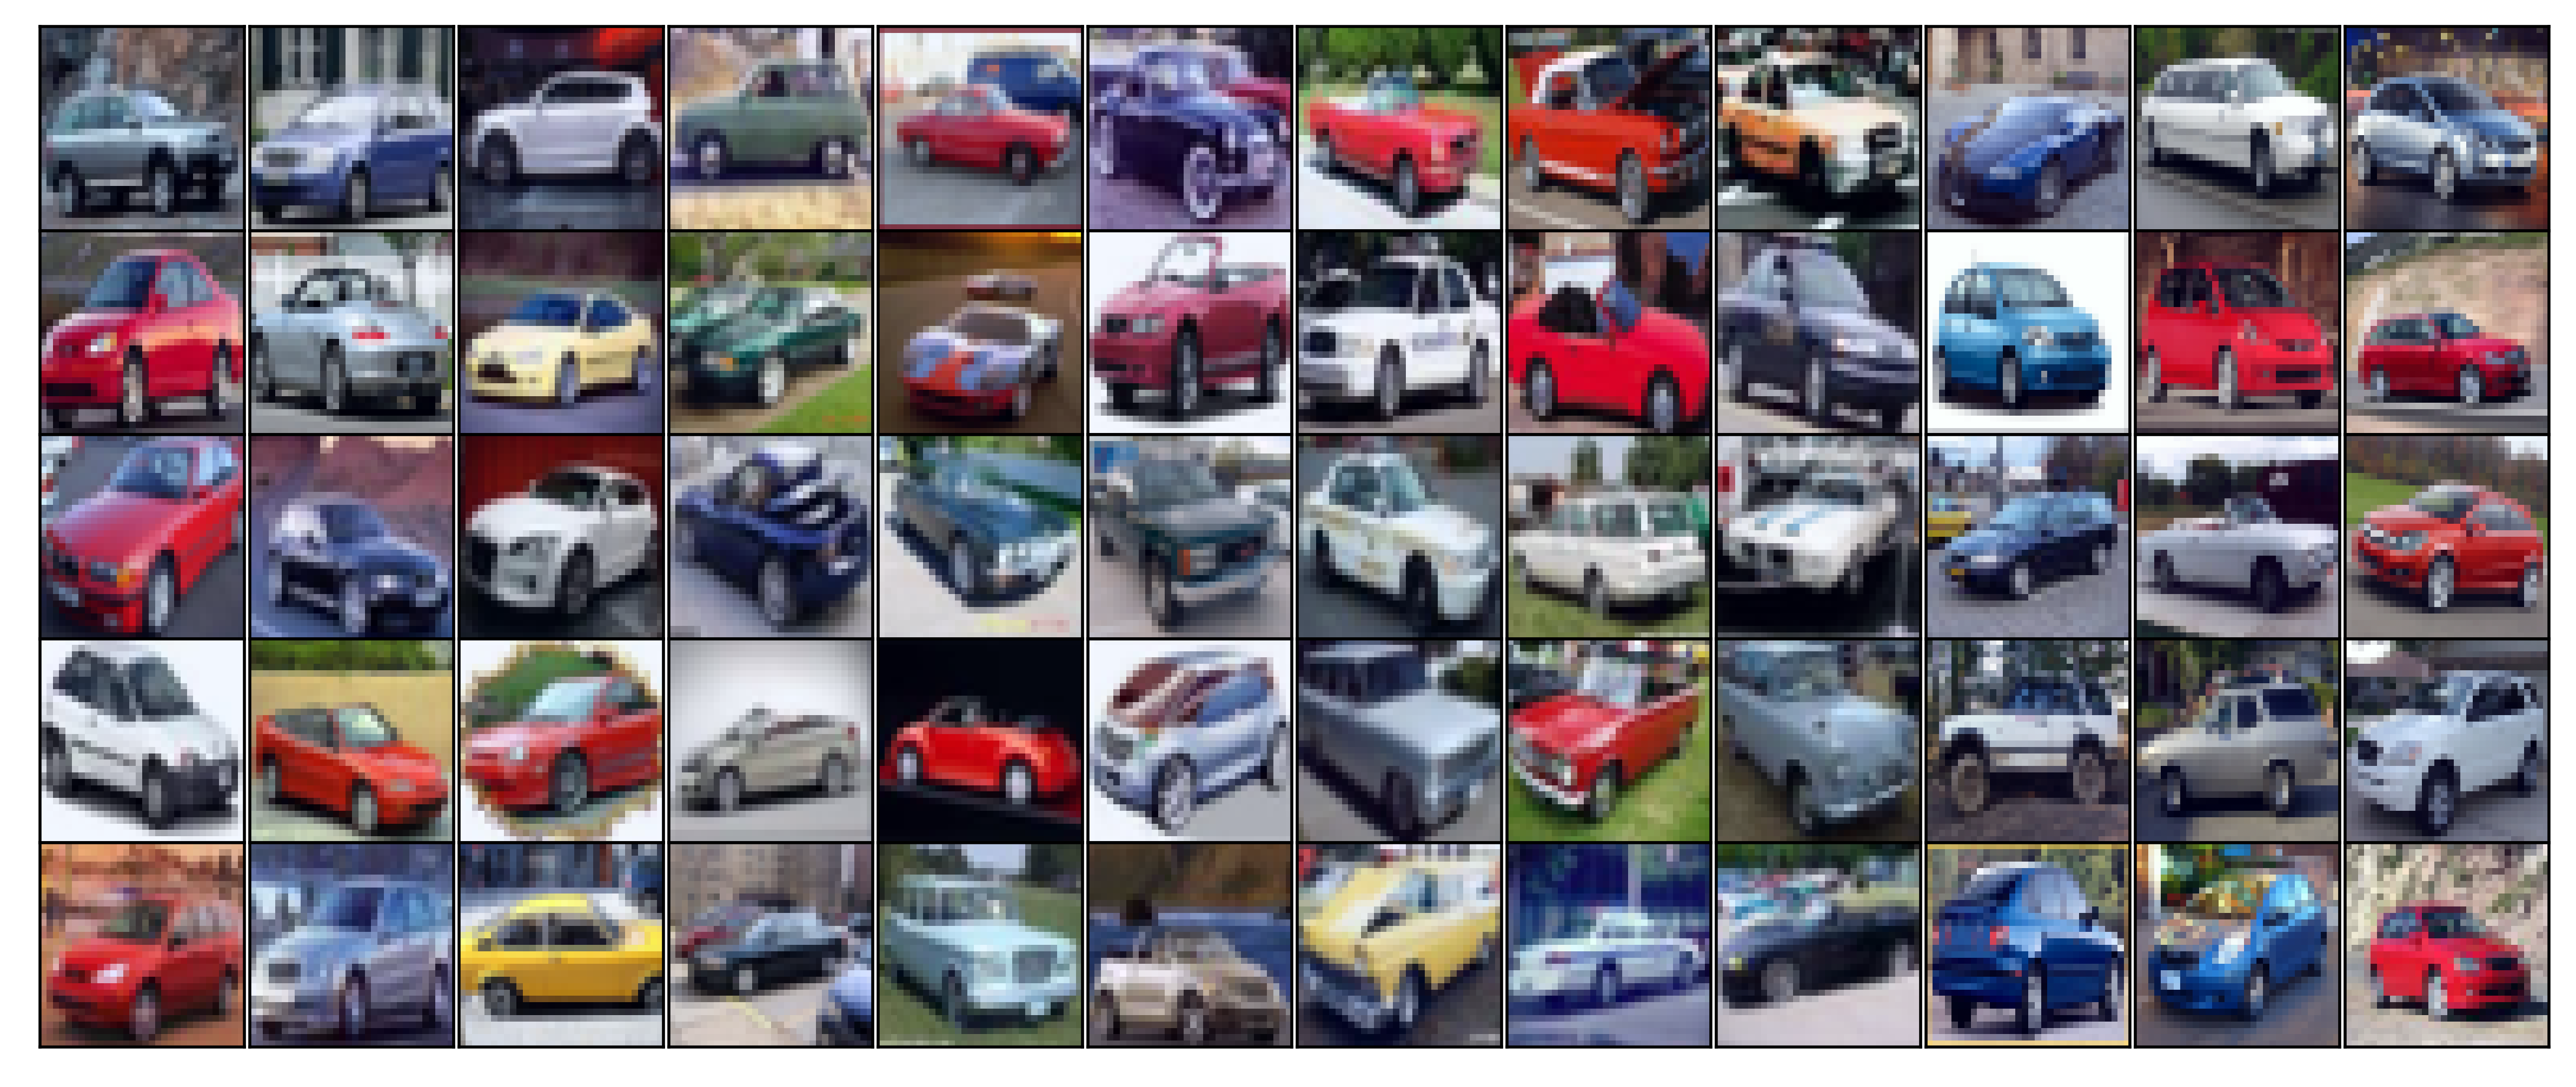} \hspace{3mm}
    \includegraphics[width=0.48\textwidth]{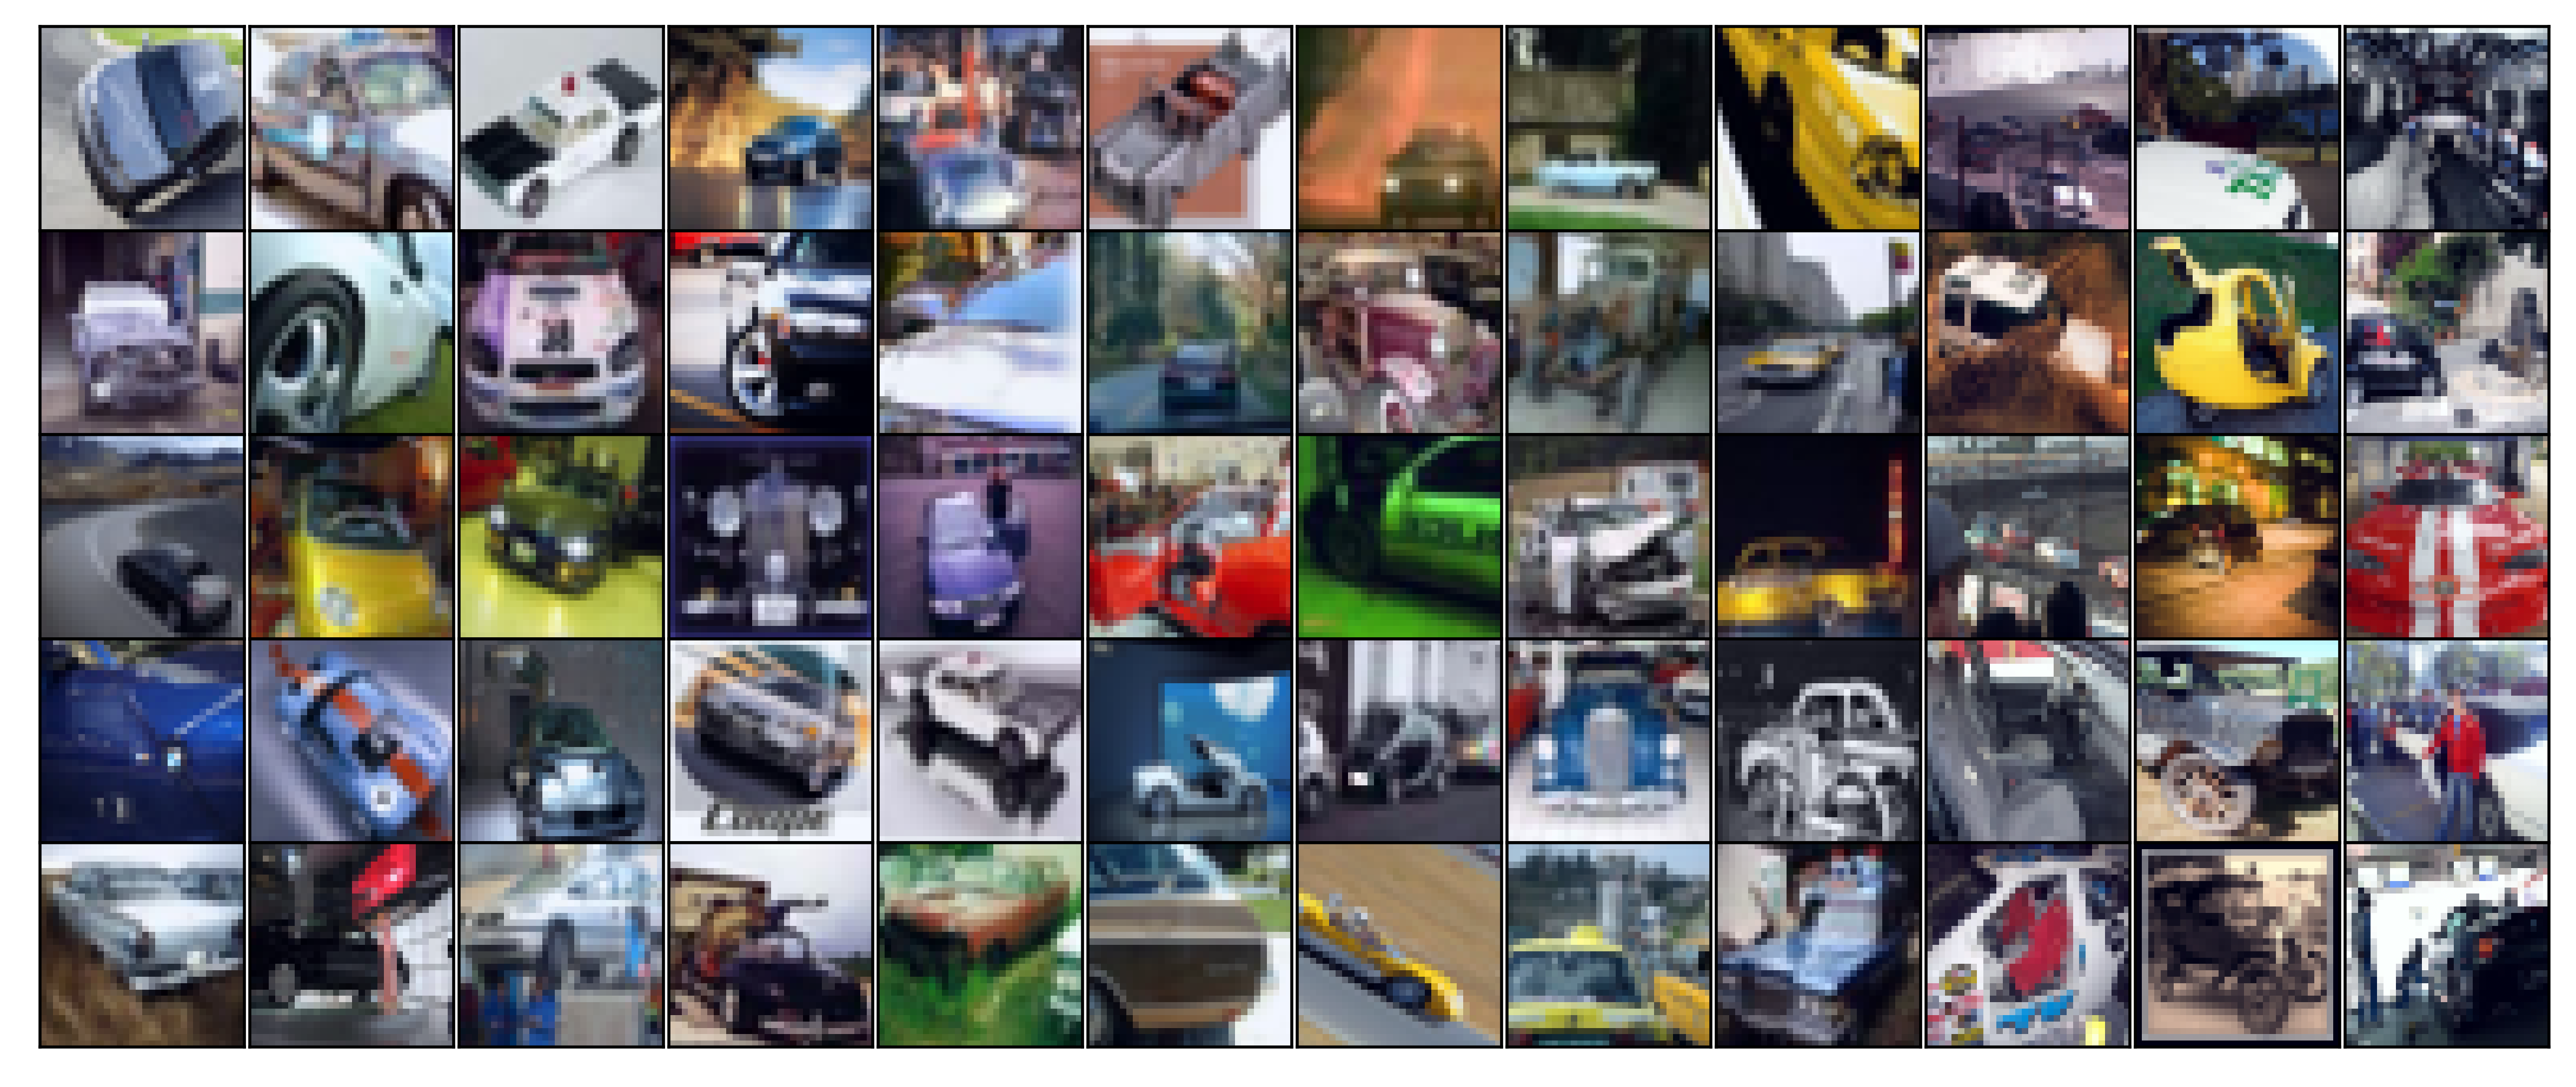}
    \includegraphics[width=0.48\textwidth]{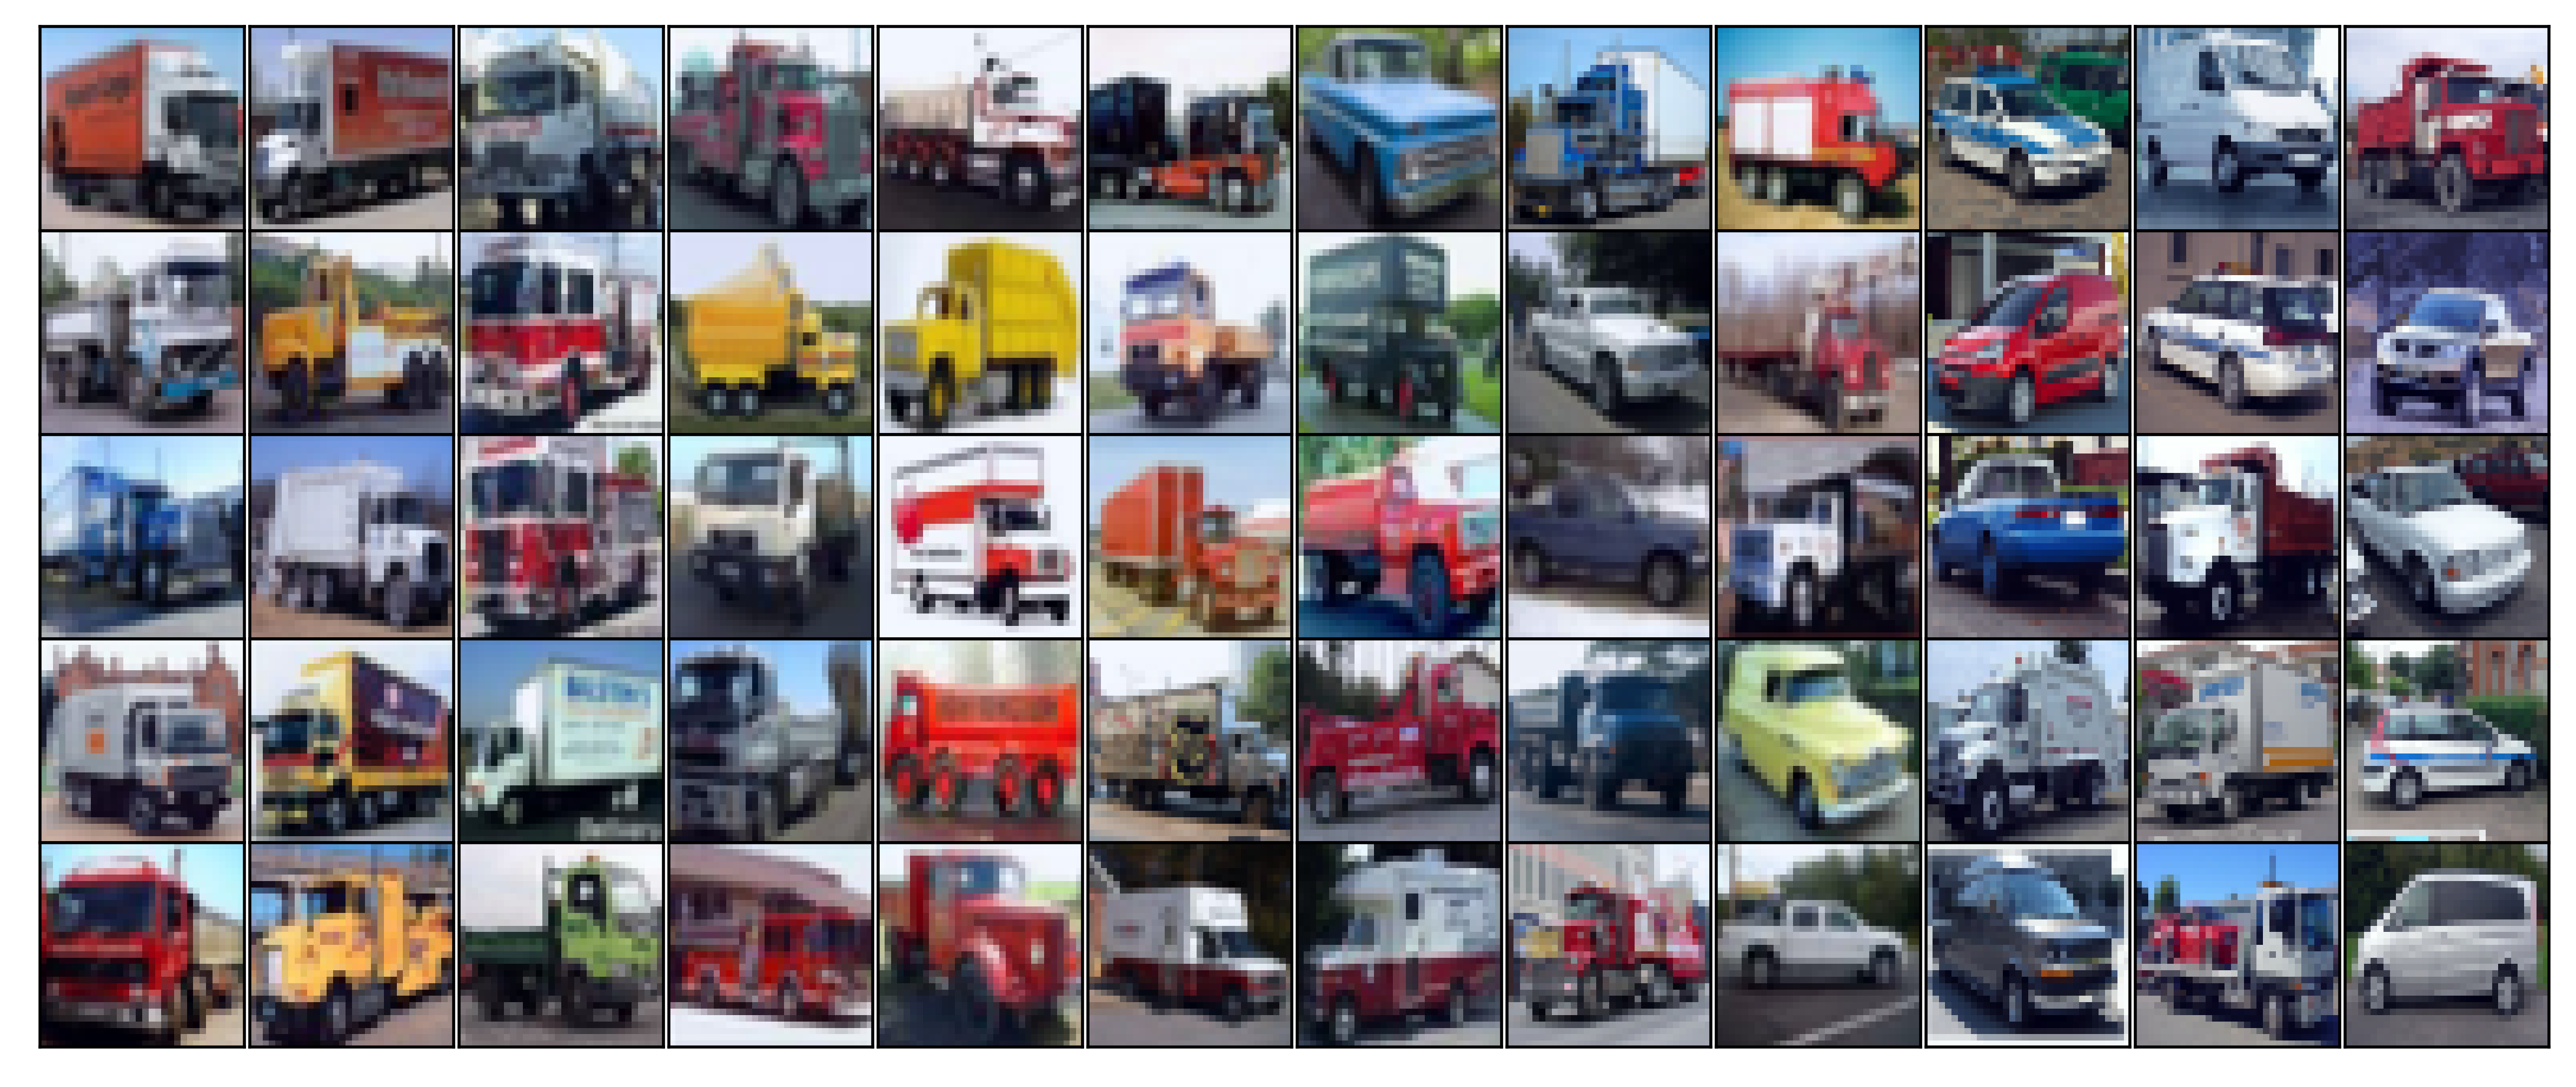} \hspace{3mm}
    \includegraphics[width=0.48\textwidth]{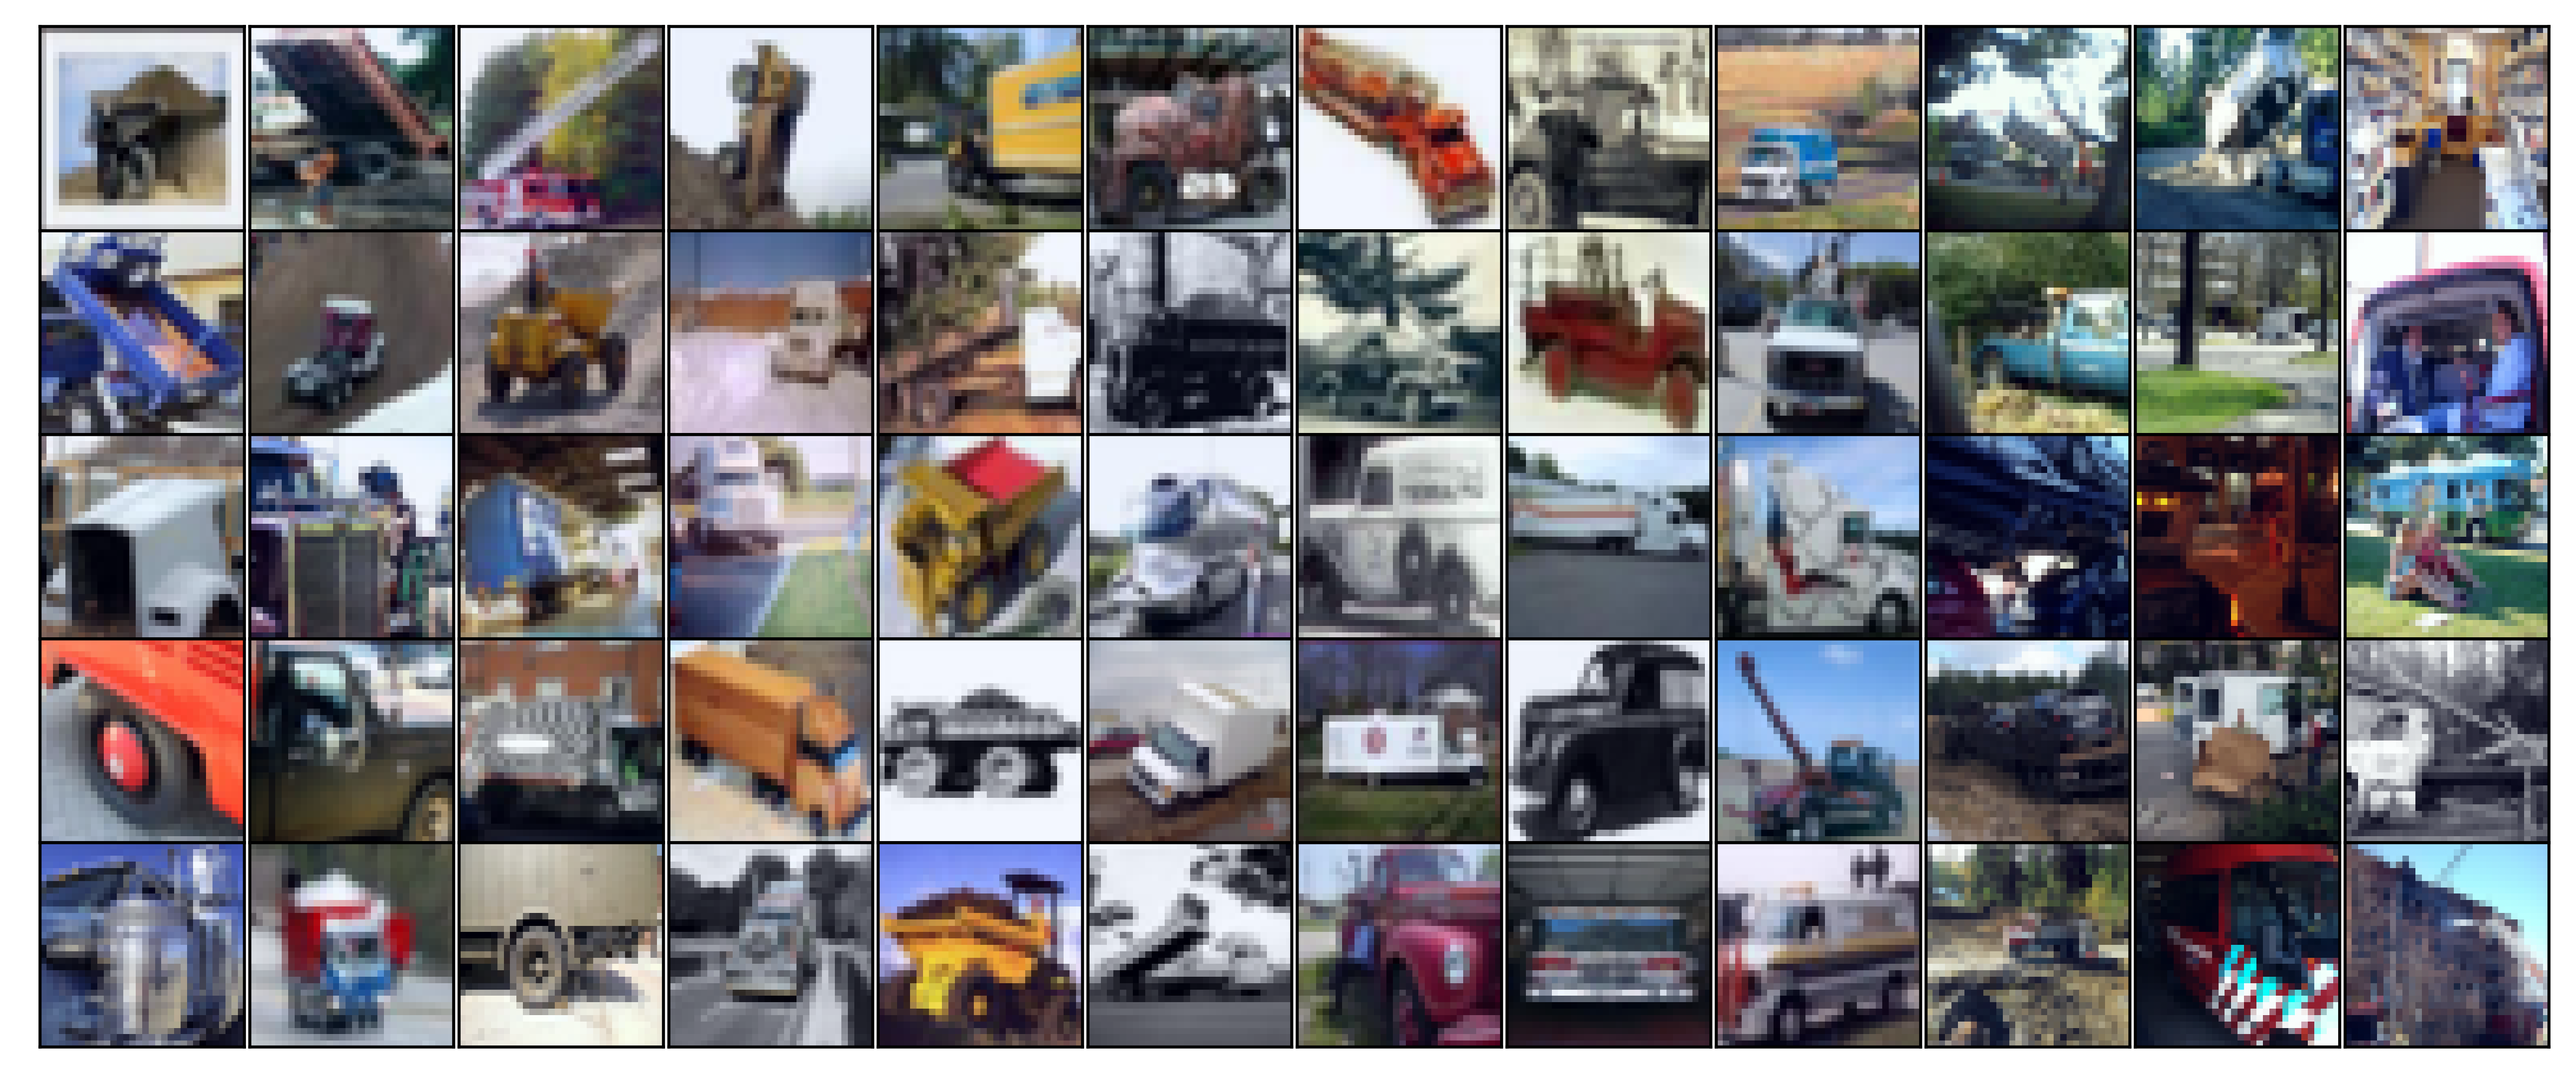}
      \includegraphics[width=0.48\textwidth]{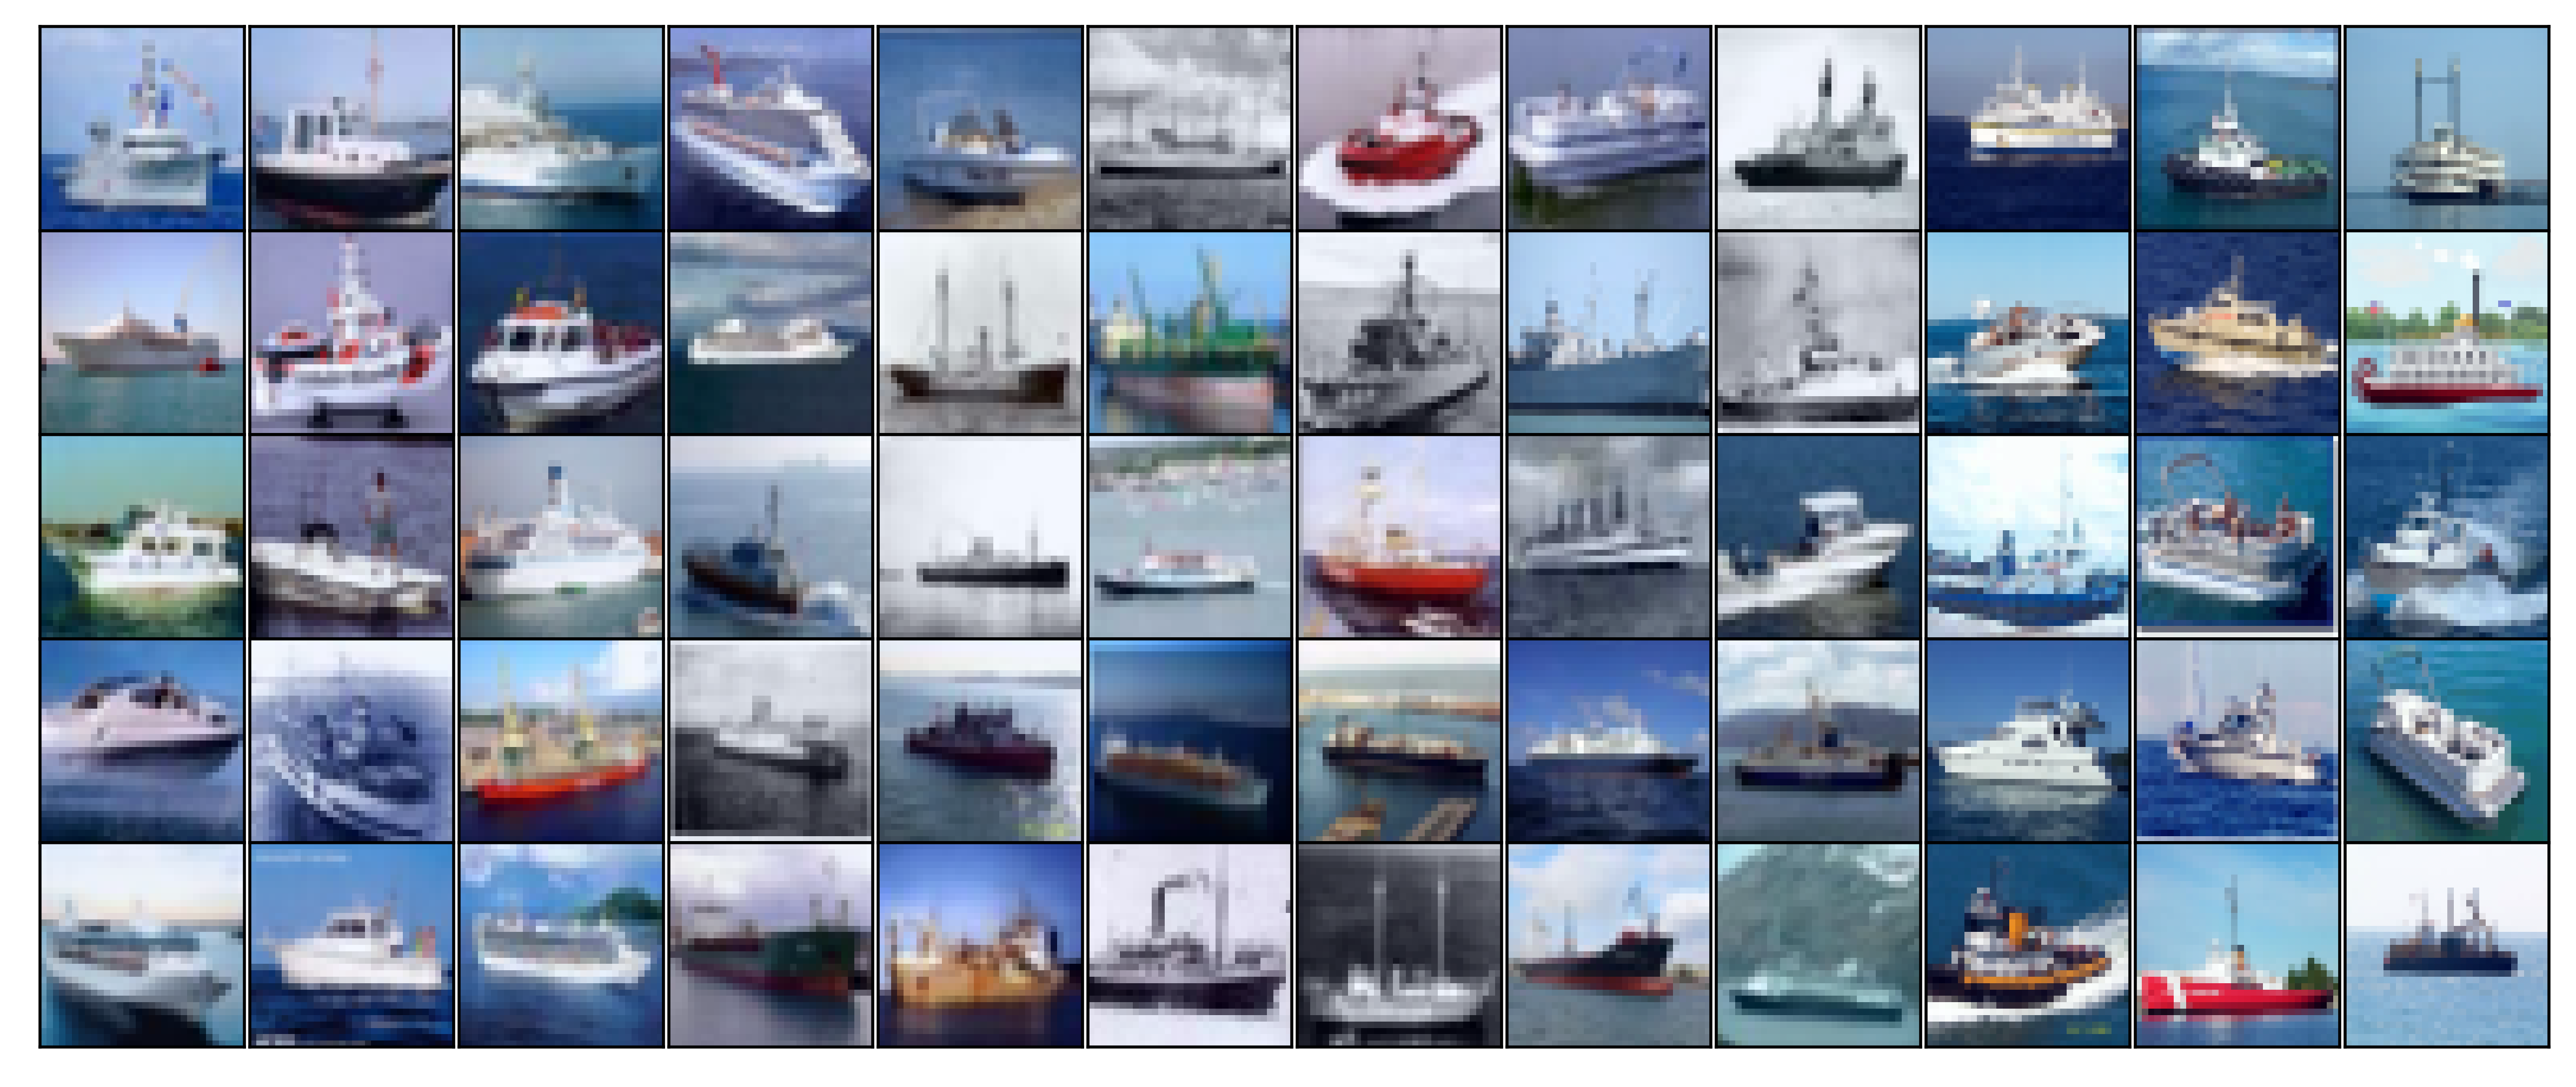} \hspace{3mm}
    \includegraphics[width=0.48\textwidth]{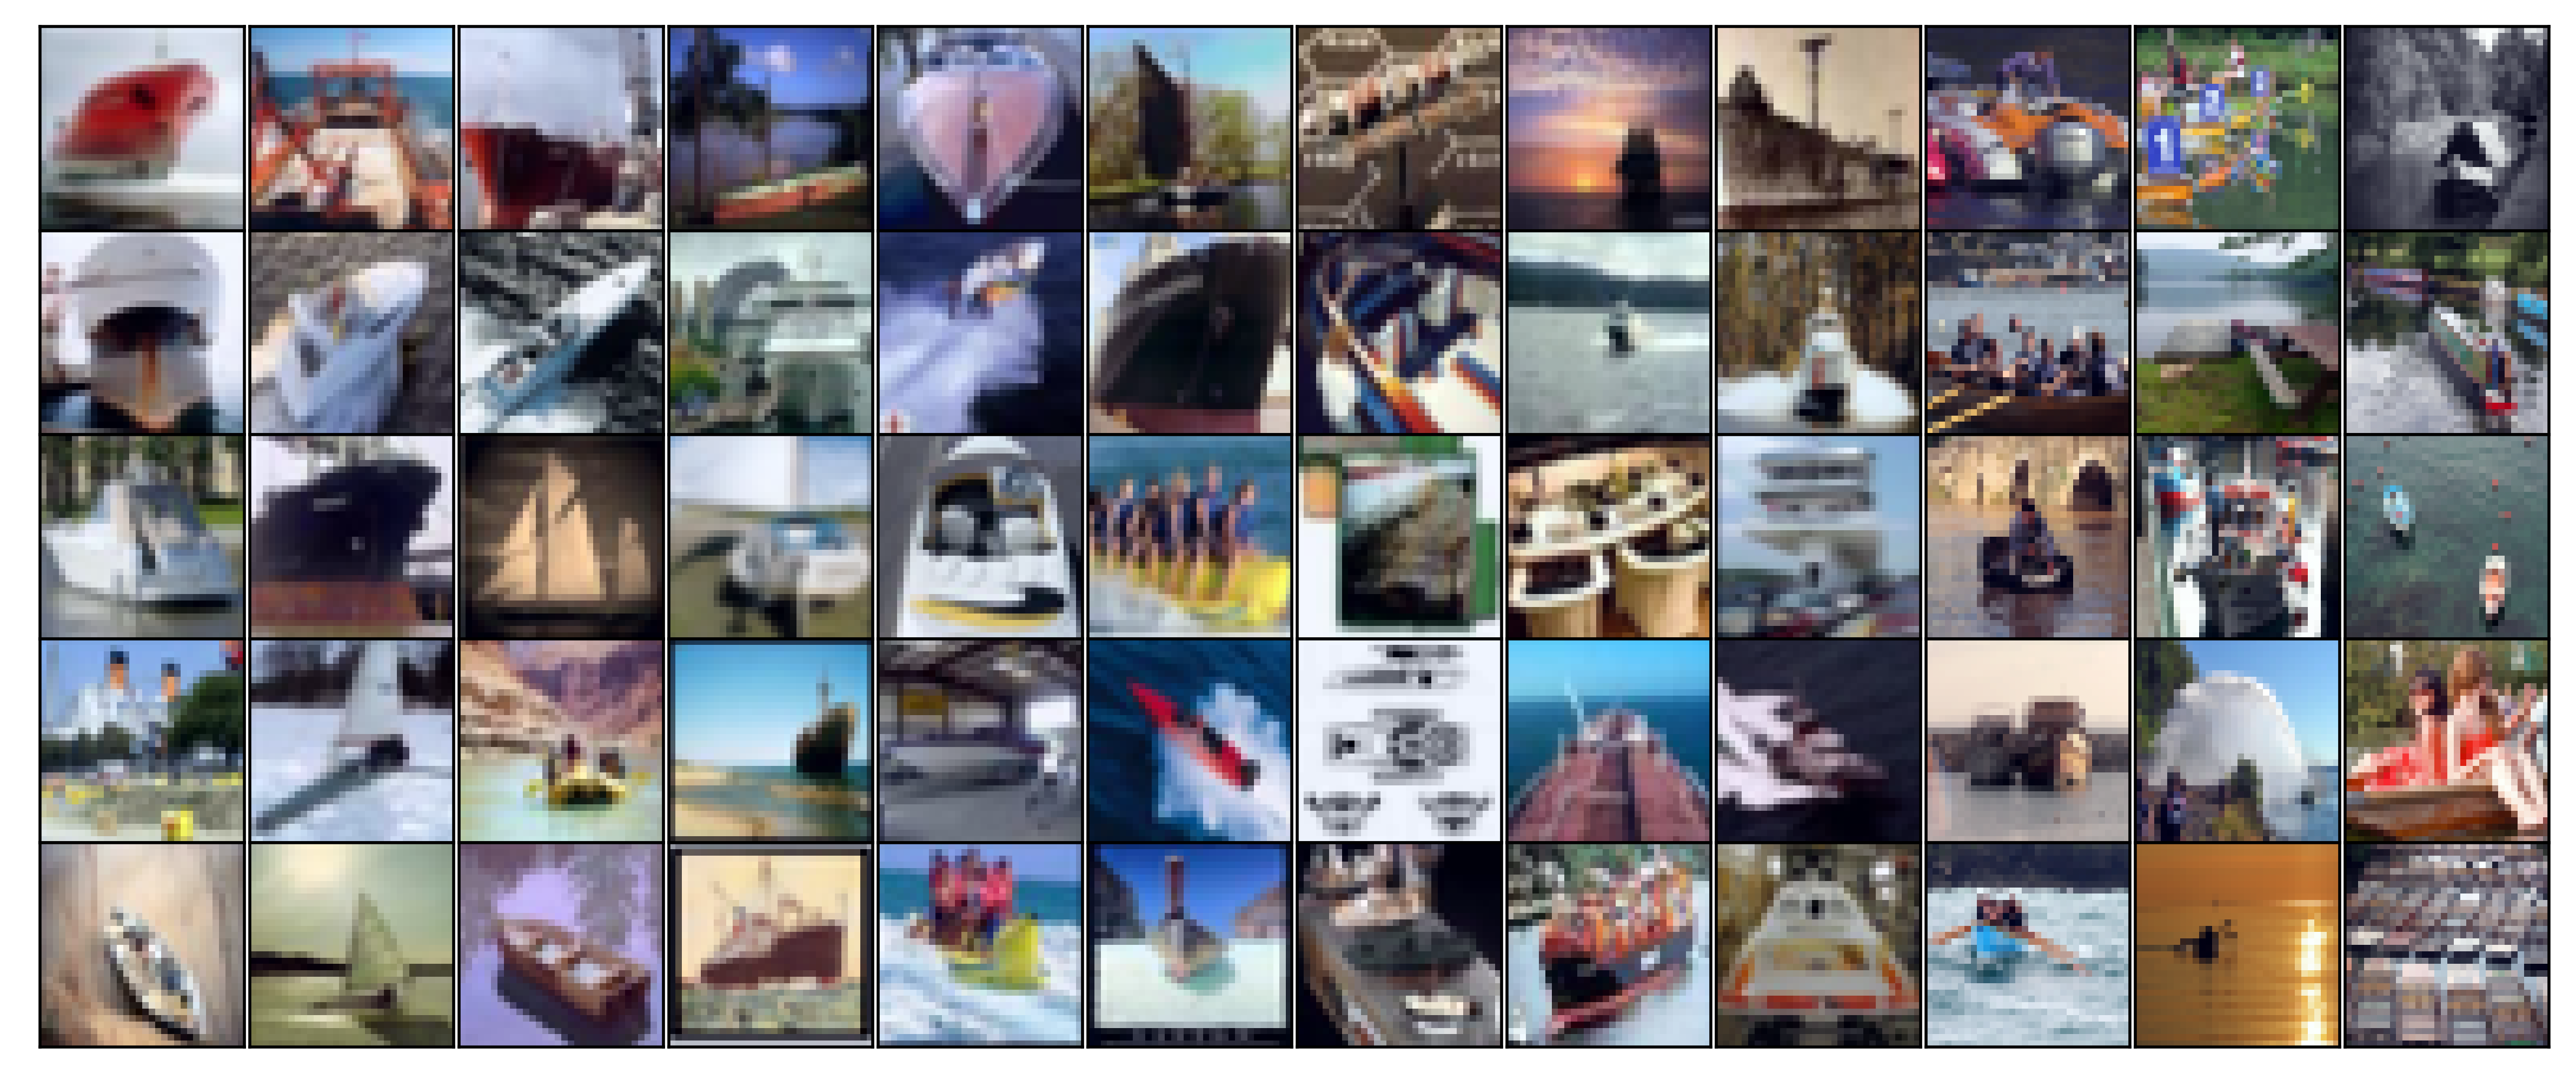}
   \includegraphics[width=0.48\textwidth]{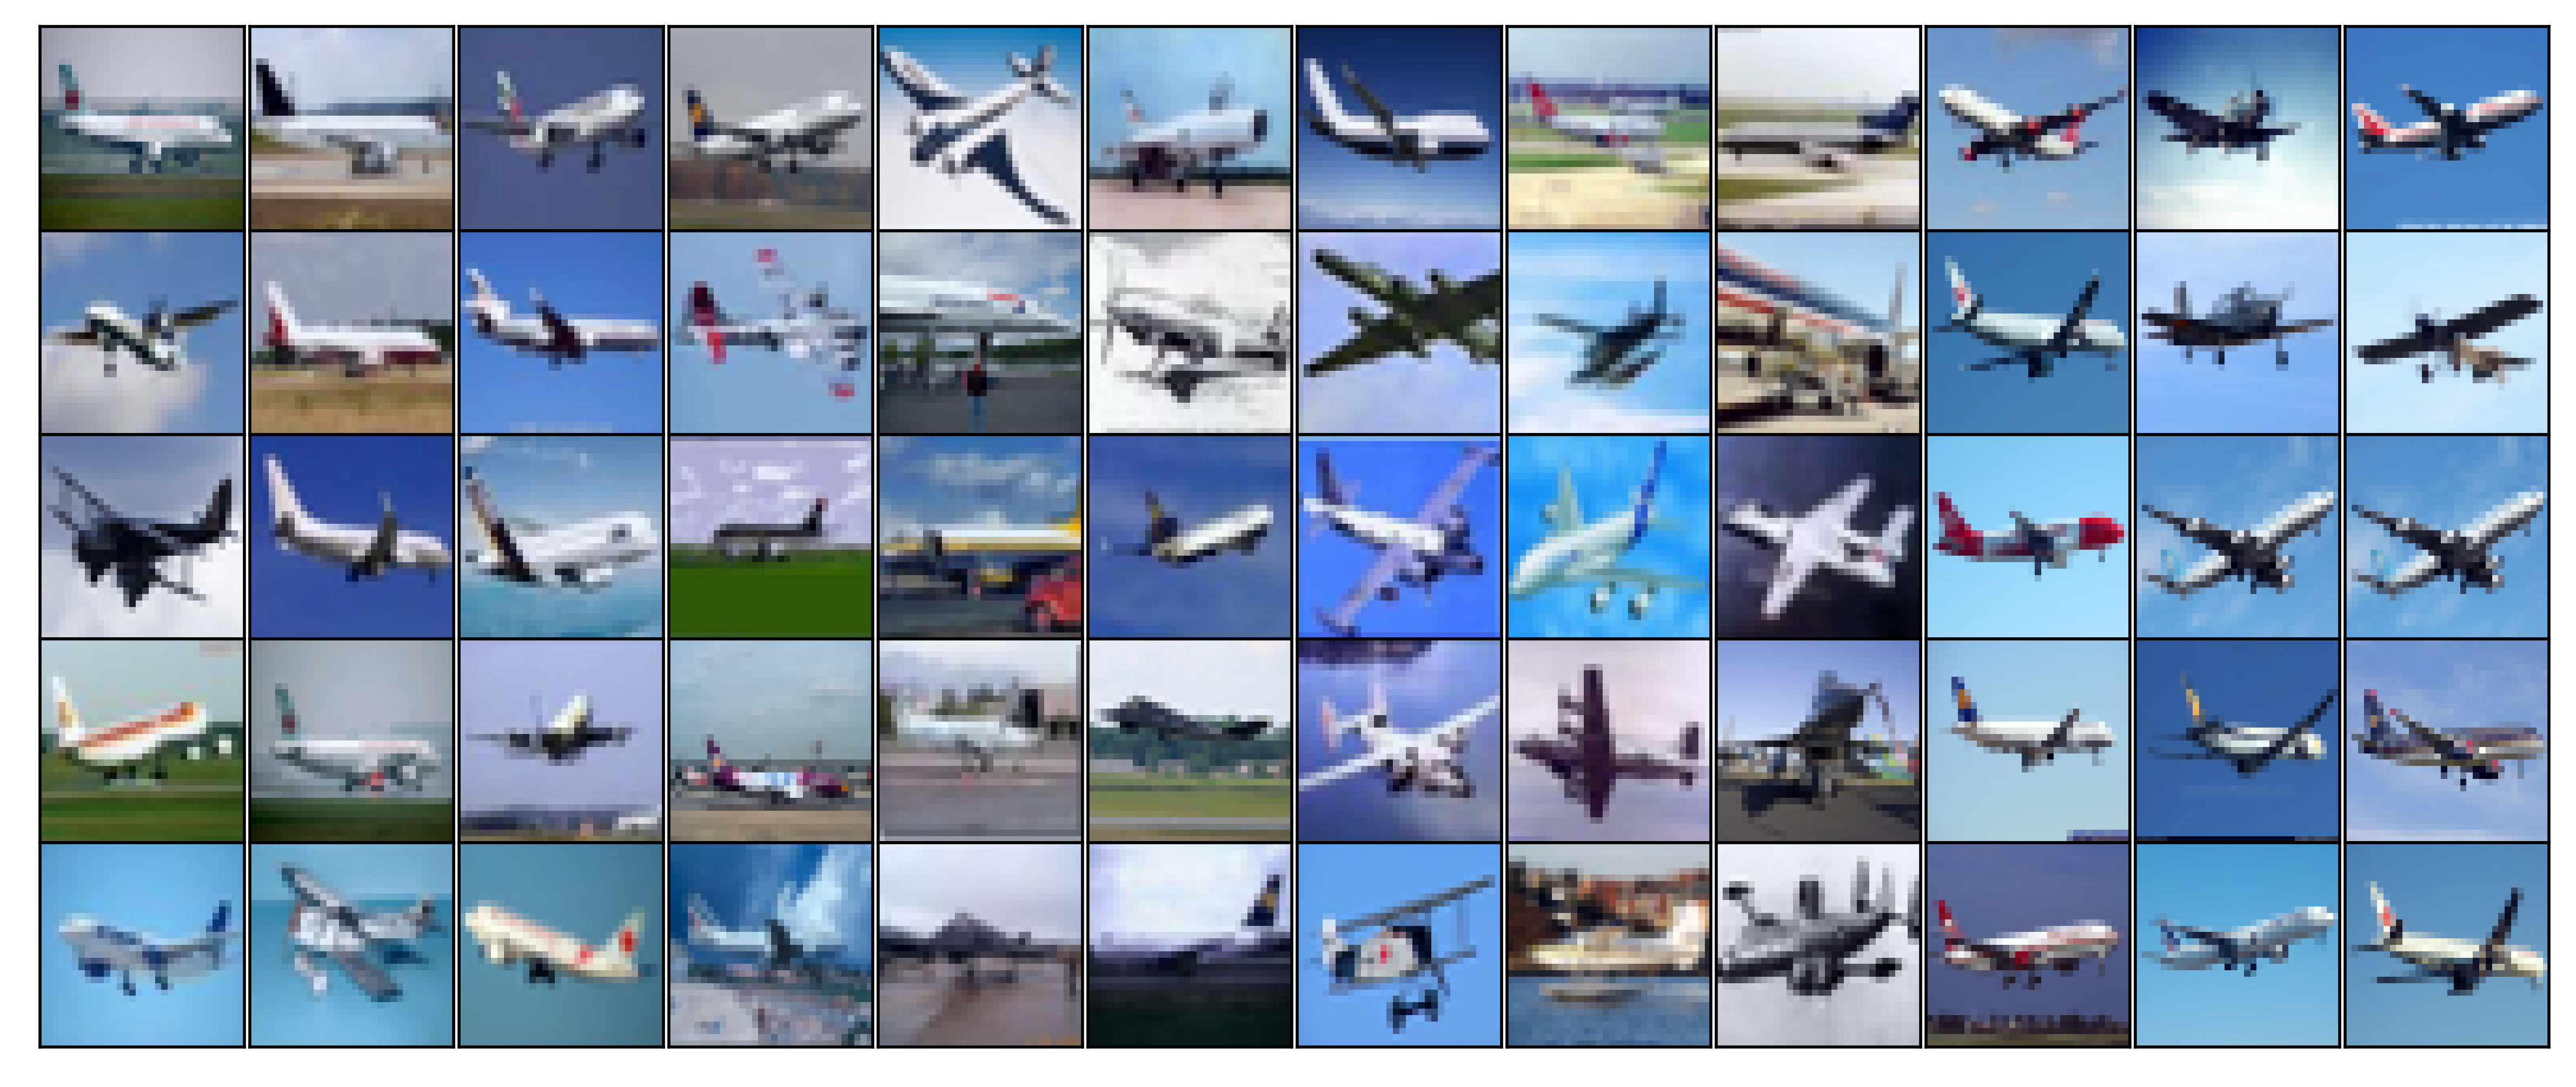} \hspace{3mm}
    \includegraphics[width=0.48\textwidth]{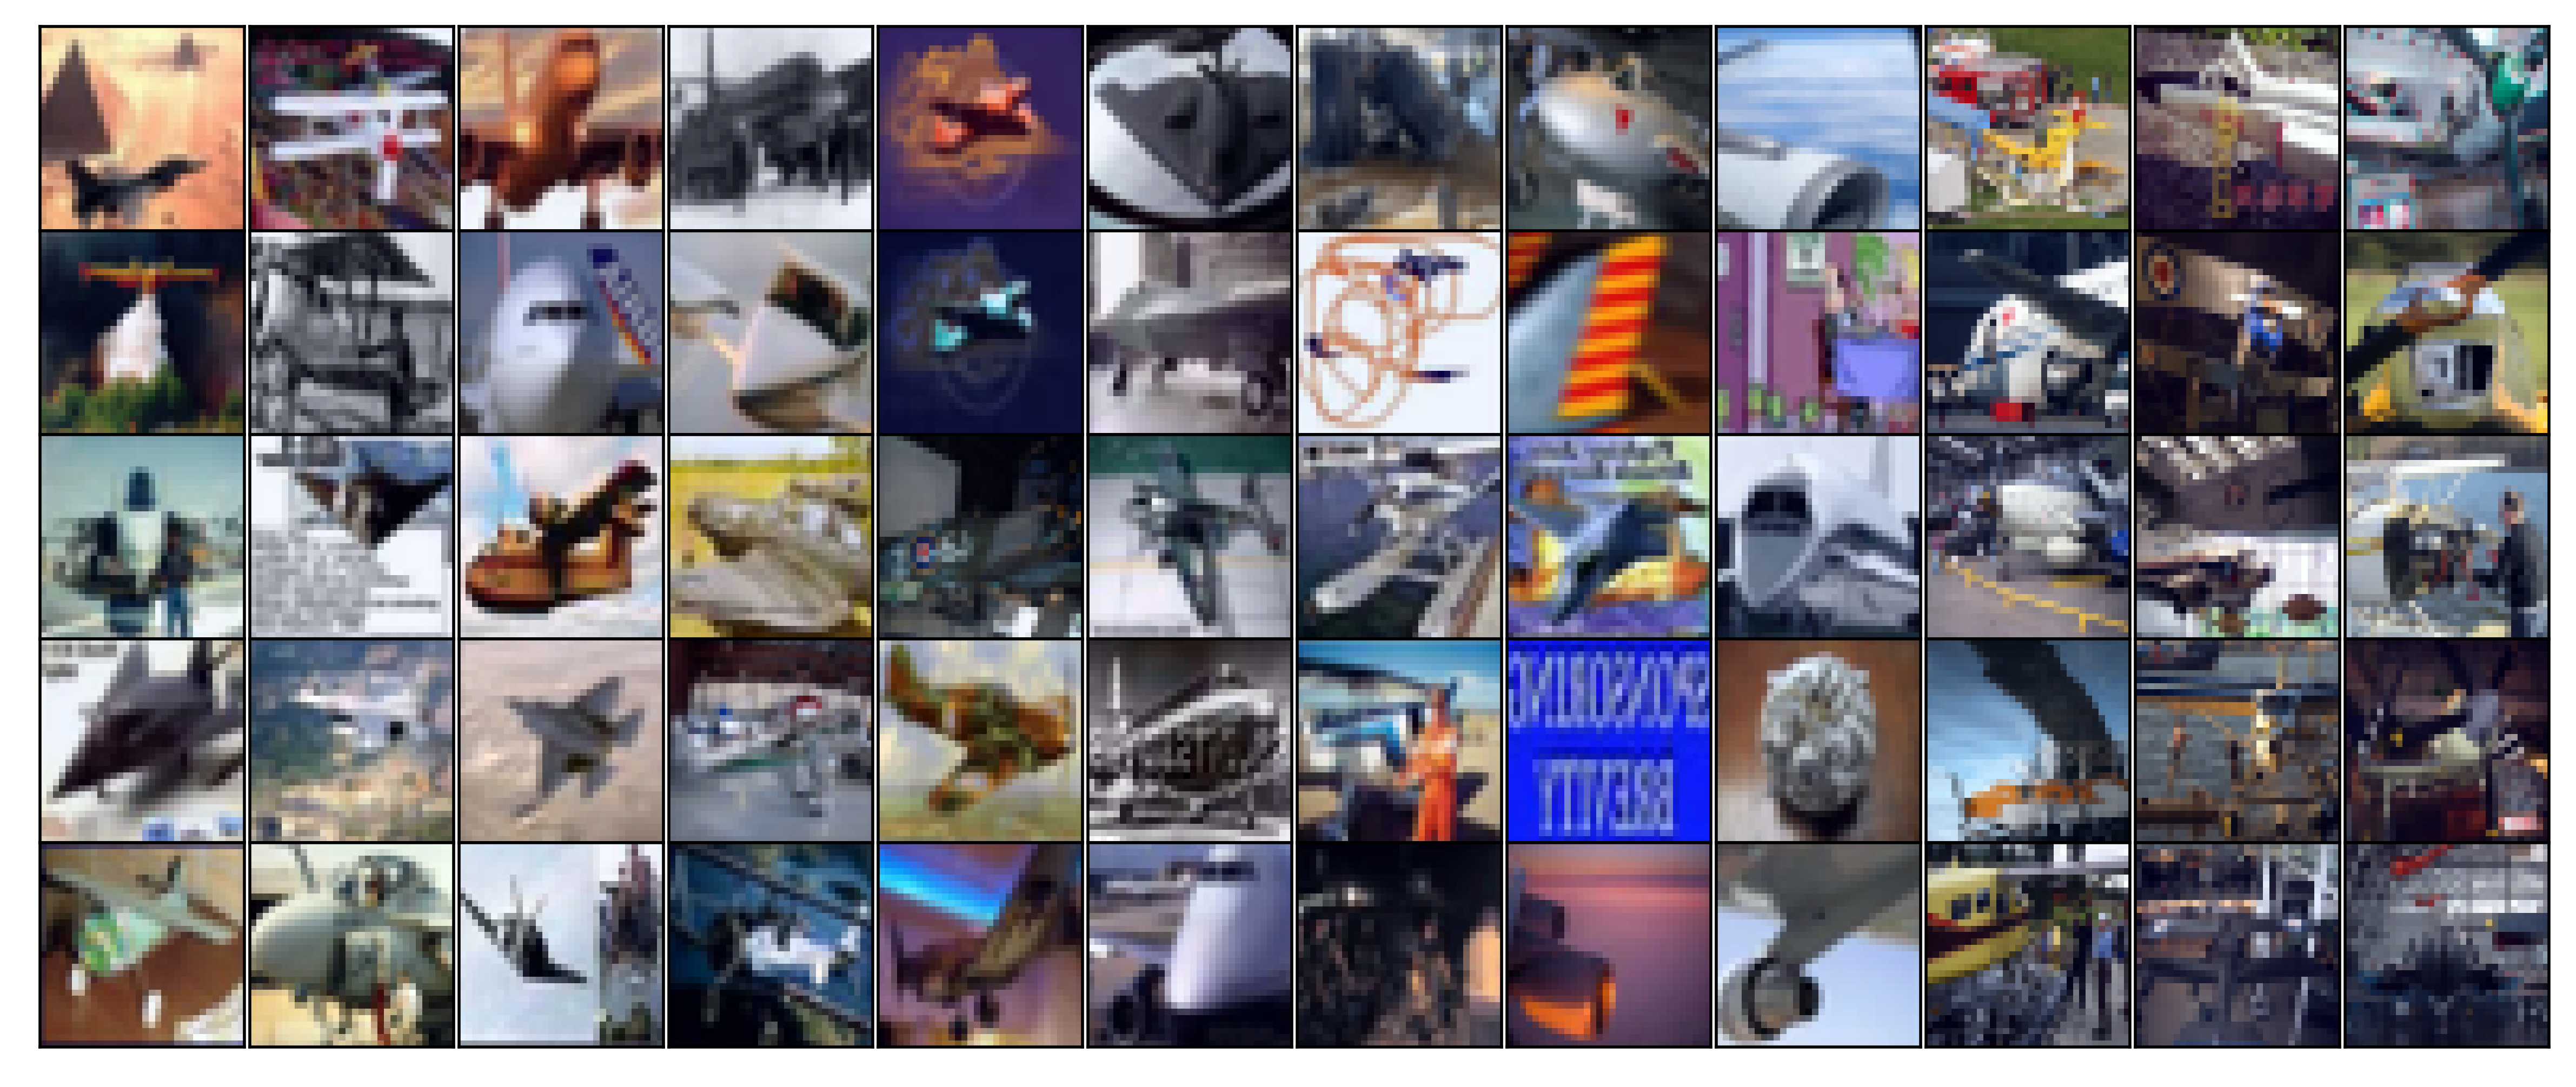} 
      \includegraphics[width=0.48\textwidth]{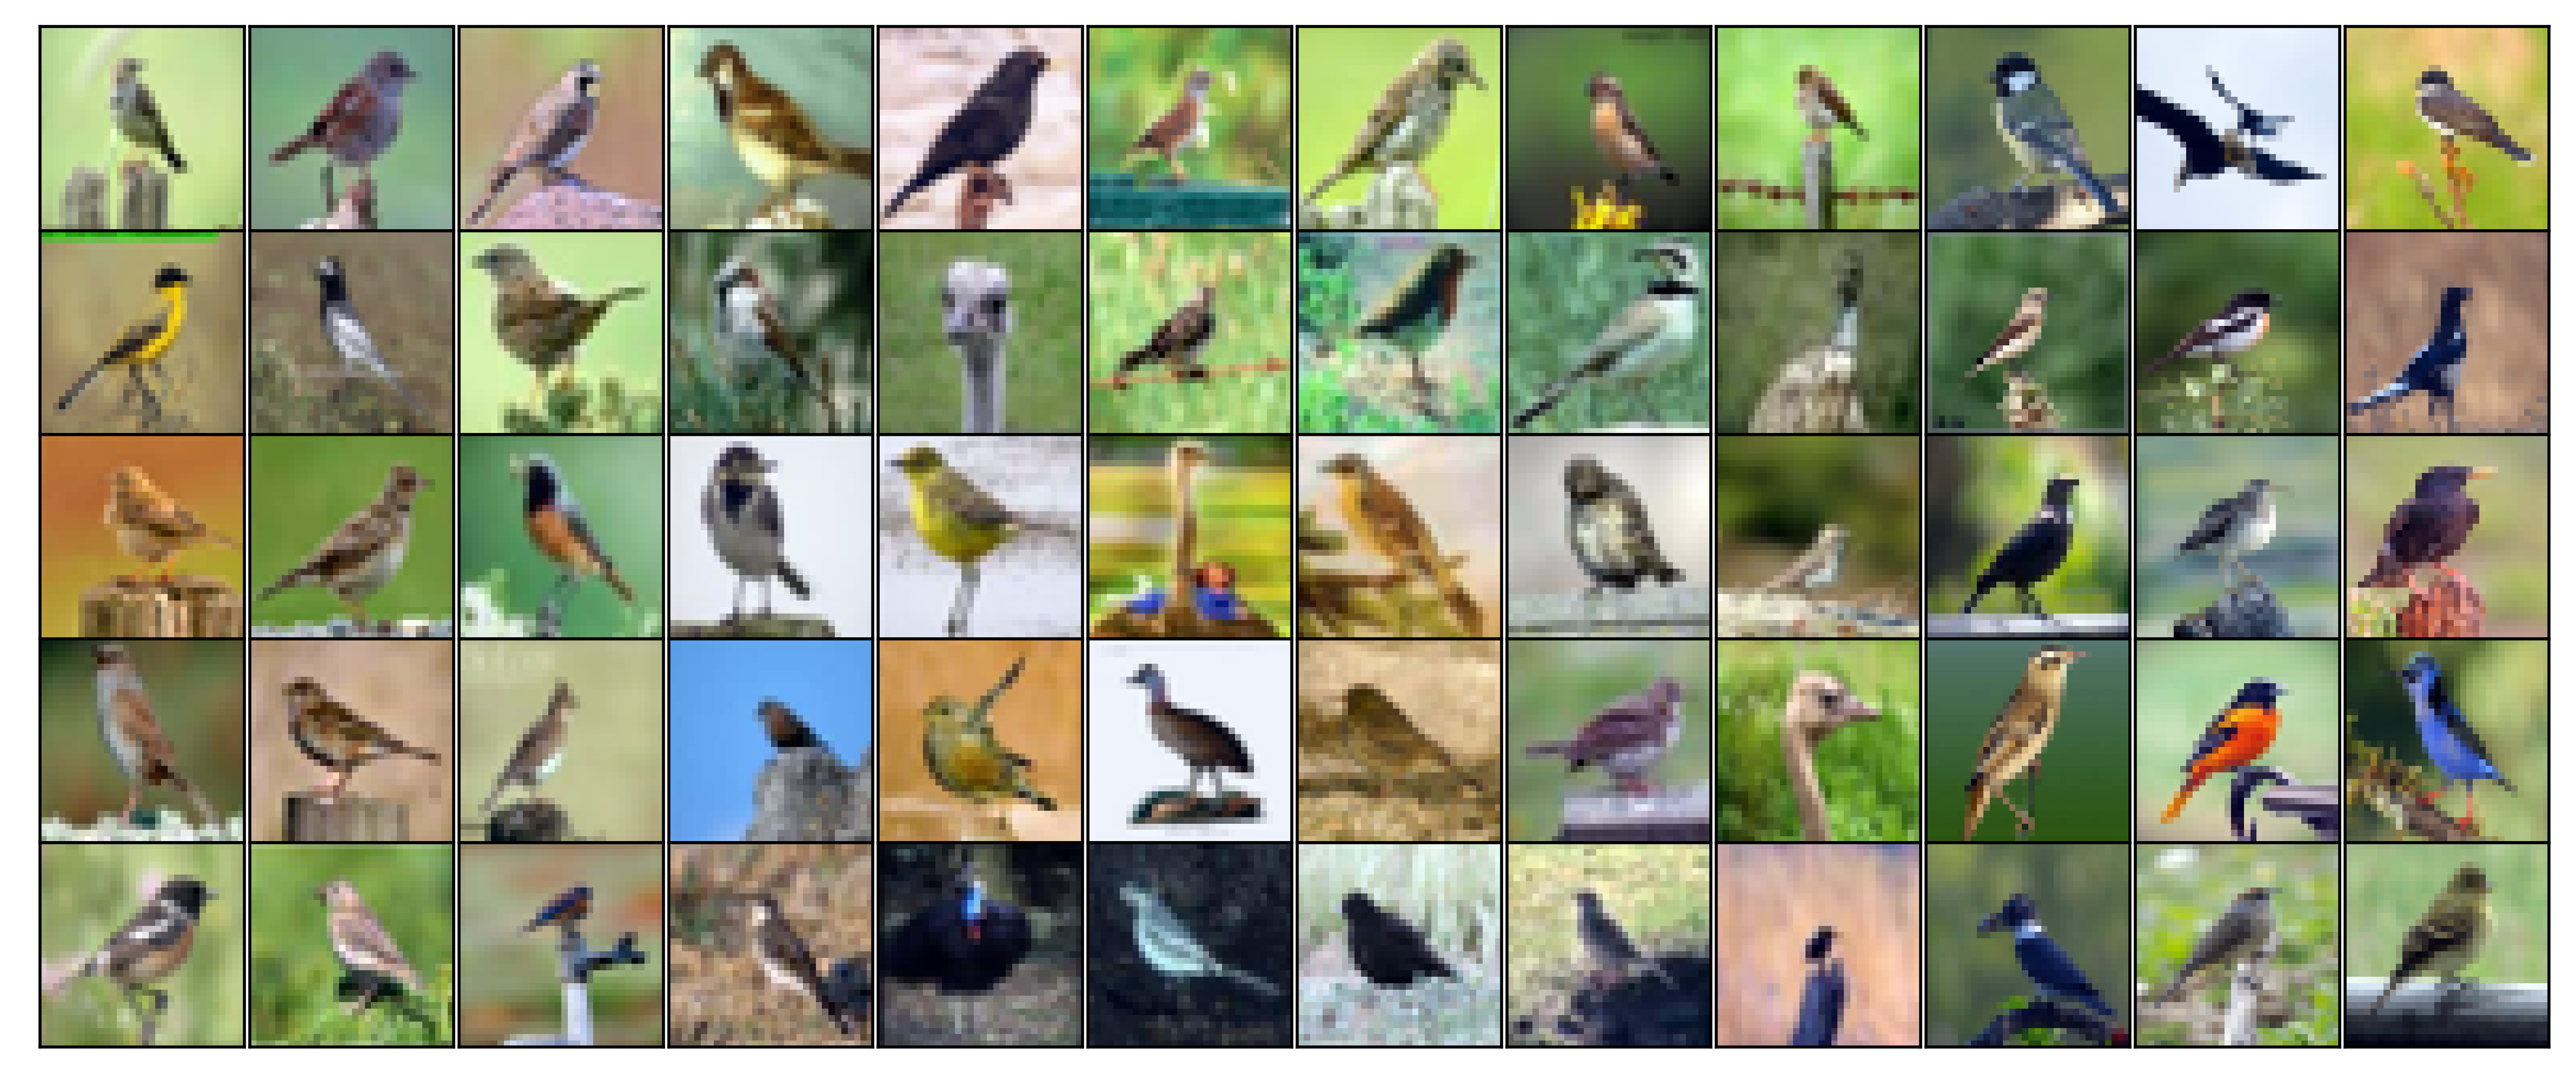} \hspace{3mm}
    \includegraphics[width=0.48\textwidth]{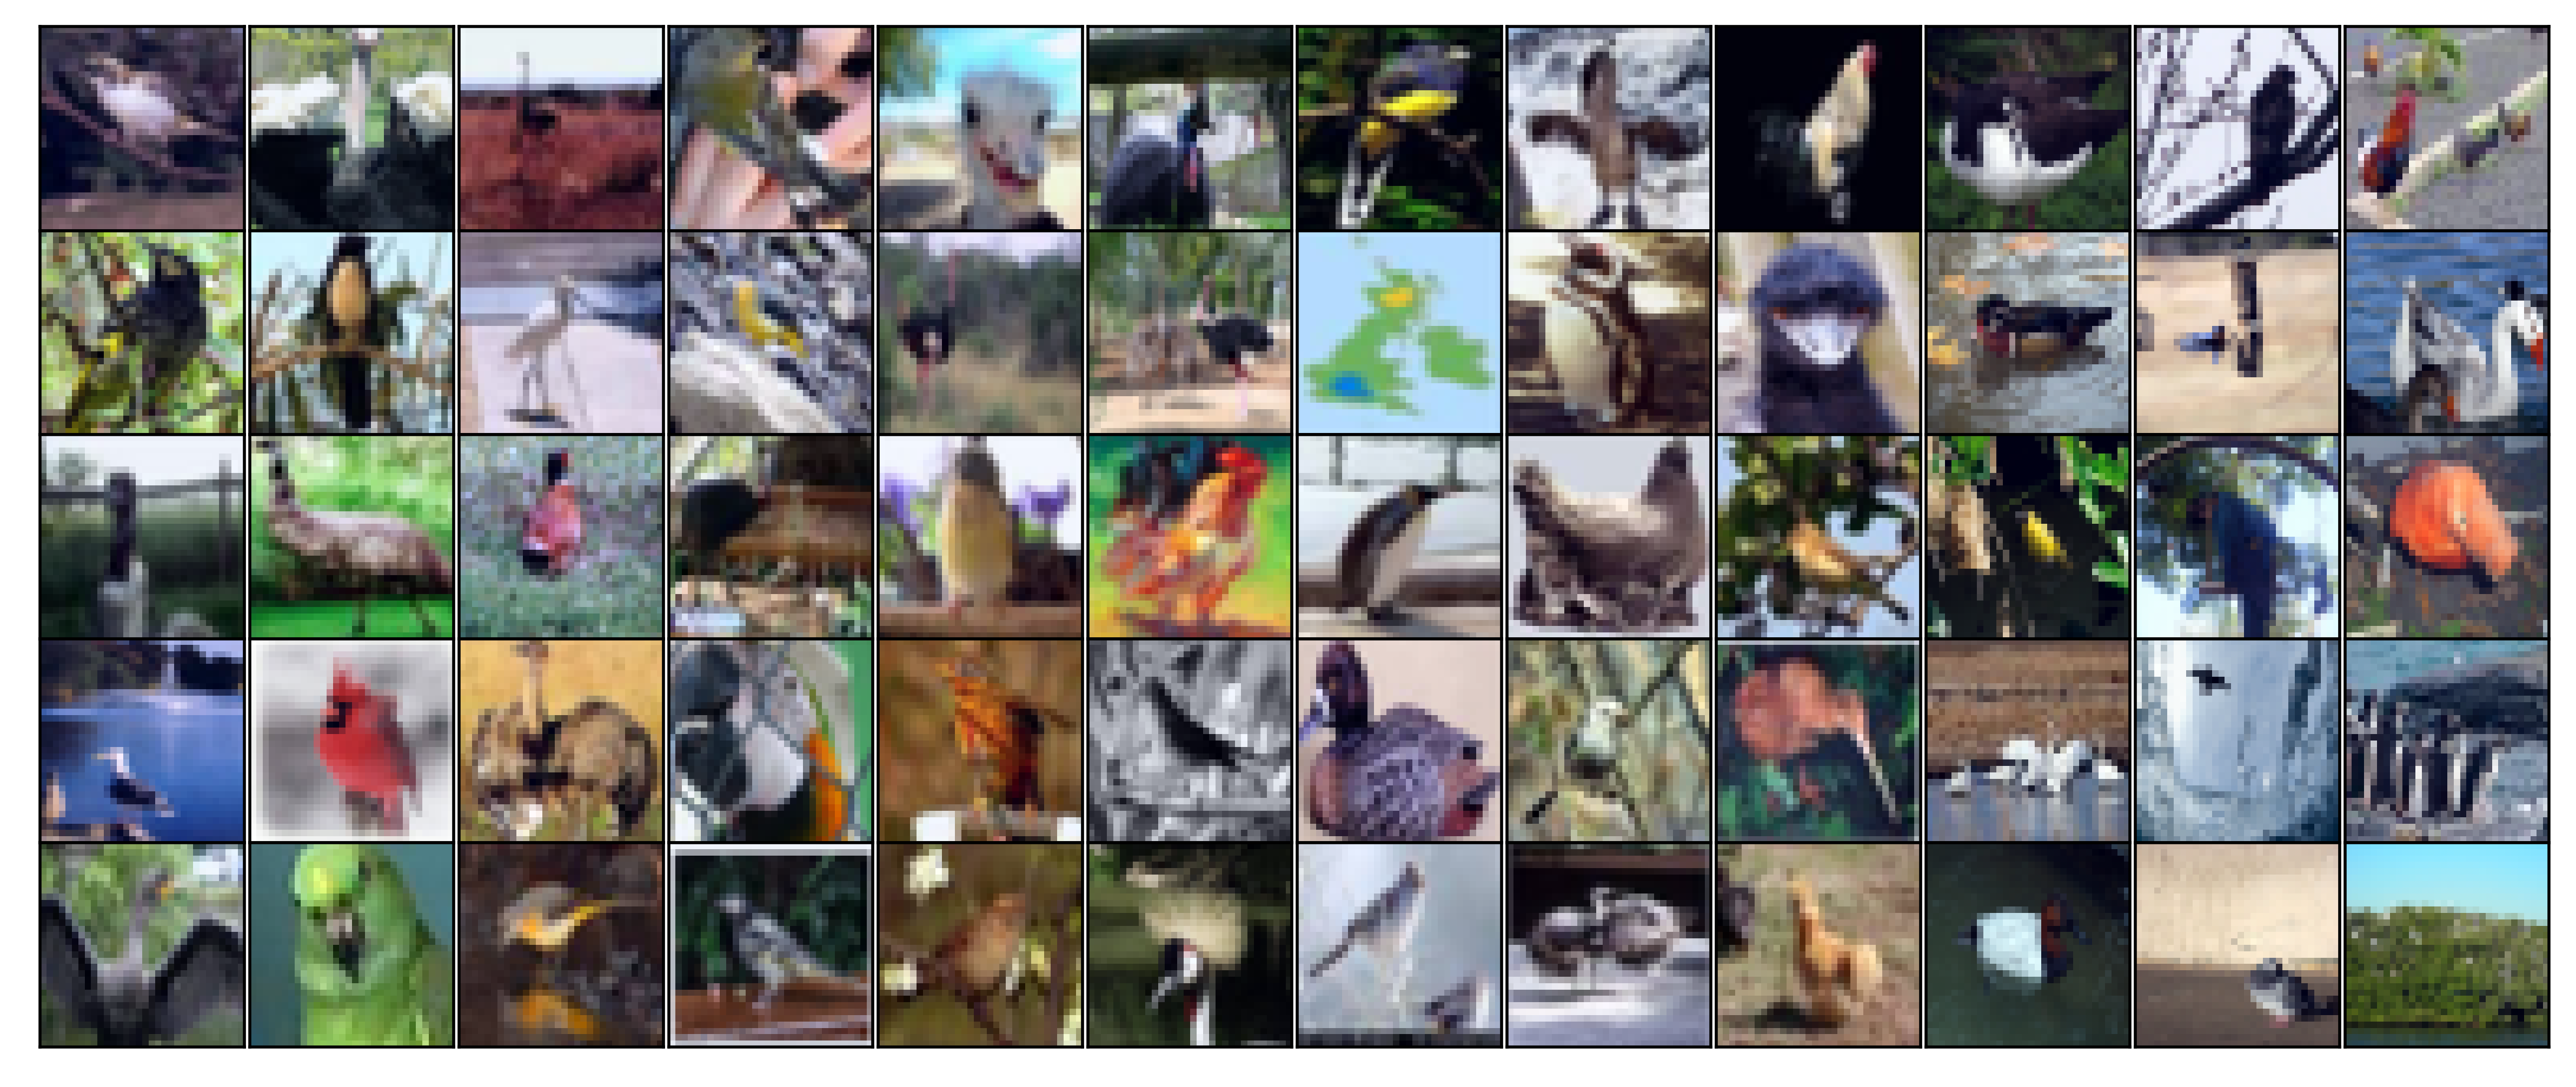}
   \end{center}
  \vspace{-0.3cm}
  \caption{\label{fig:low-high-entropy-app1} \textbf{Left: lowest entropy images; Right: highest entropy images from the CIFAR-10 test dataset (ID) and three OOD datasets (CIFAR-10.1, CIFAR-10.2, and CINIC-10)}} 
\end{figure}

\begin{figure}[t!]
   \begin{center}
   \includegraphics[width=0.48\textwidth]{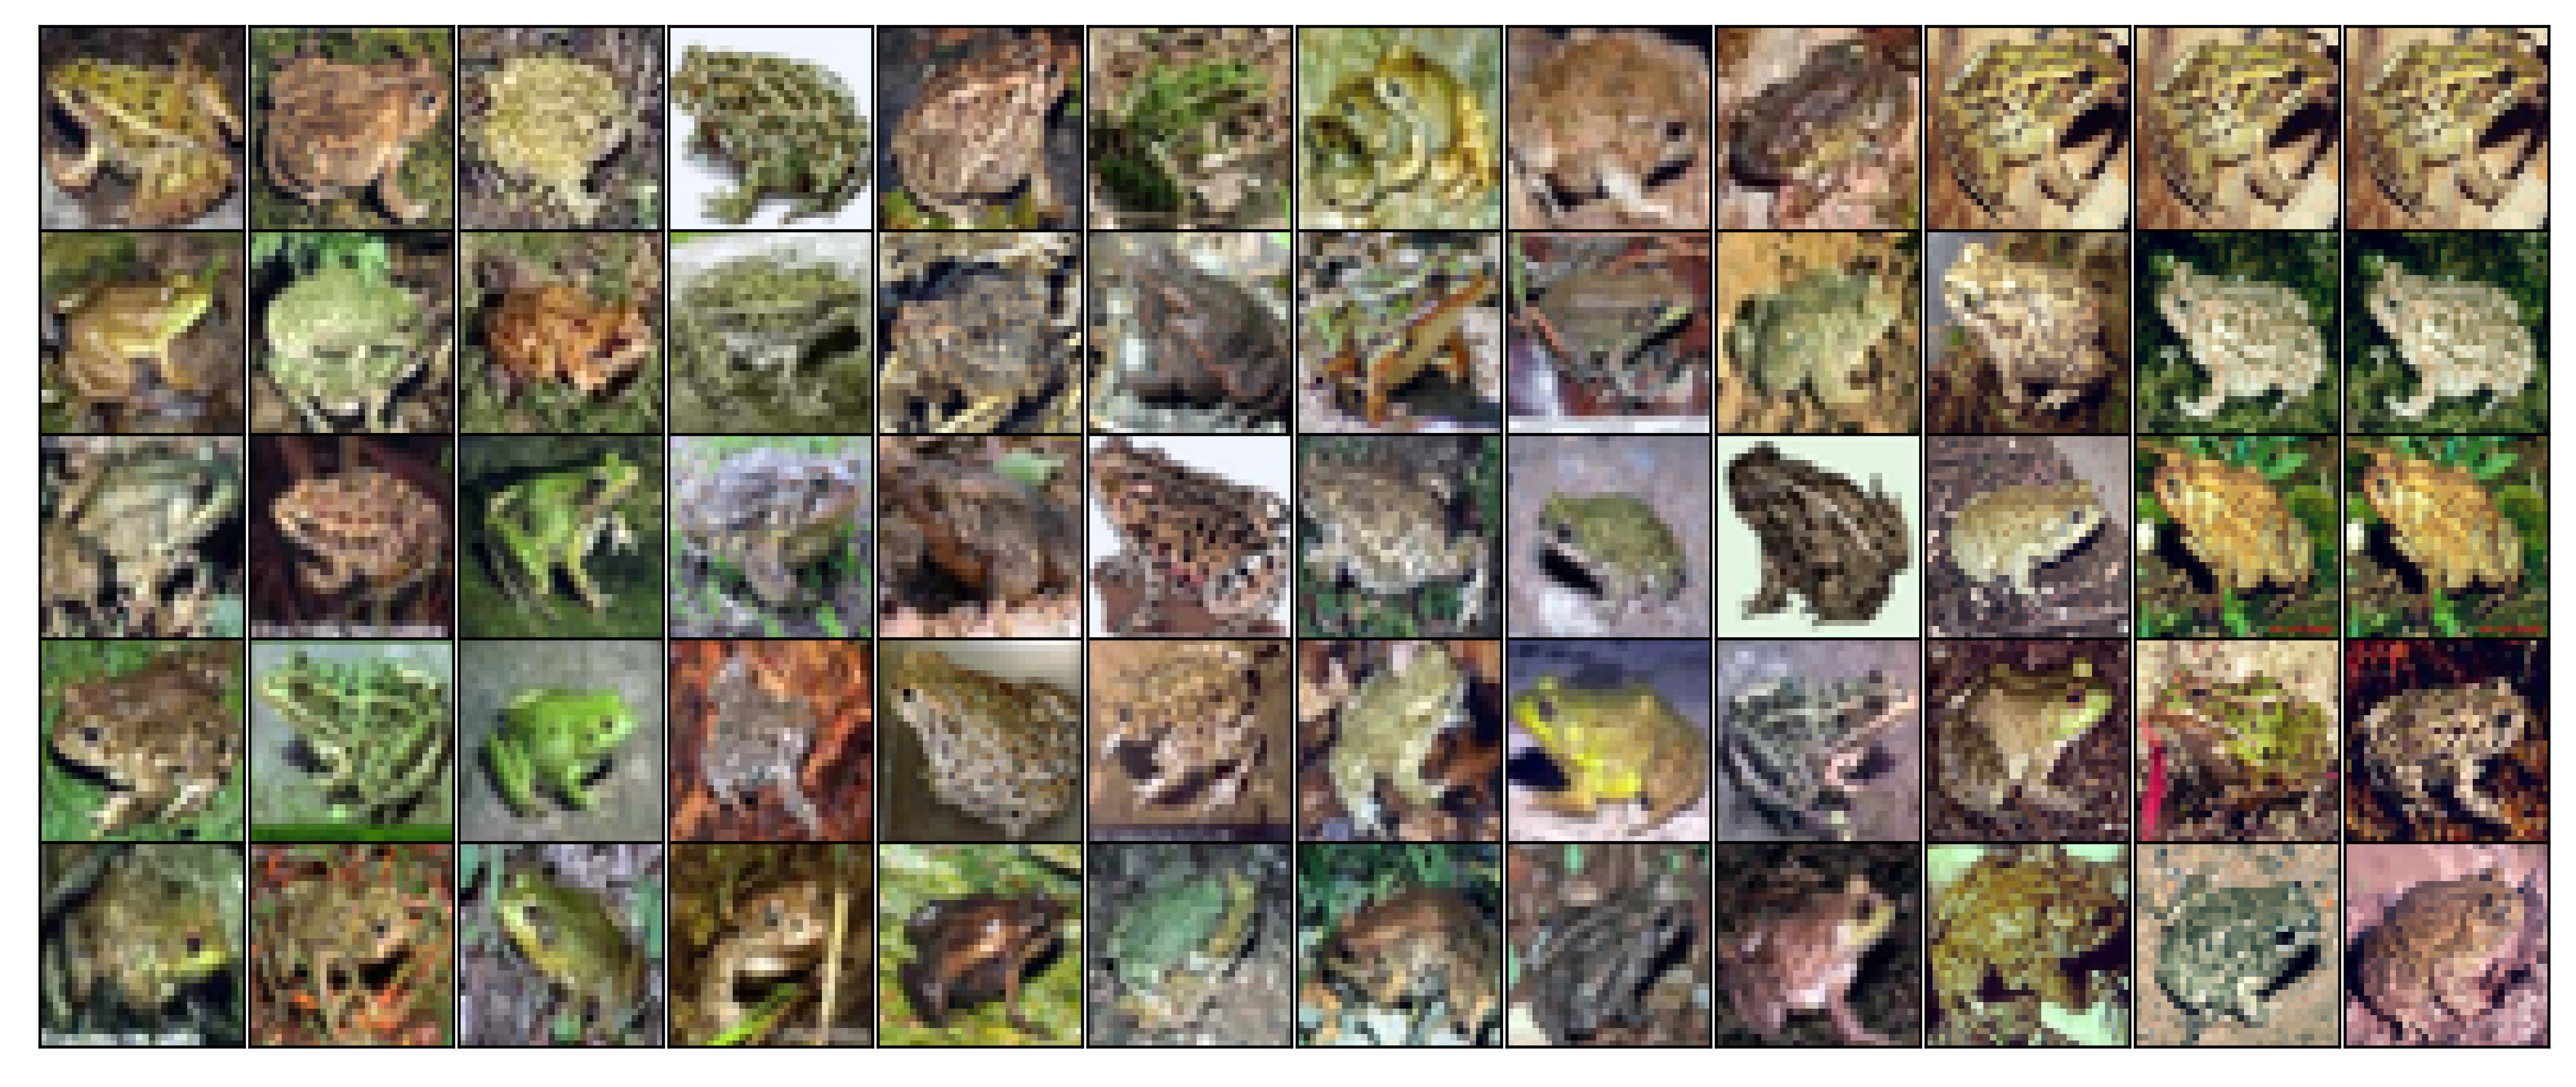} \hspace{3mm}
    \includegraphics[width=0.48\textwidth]{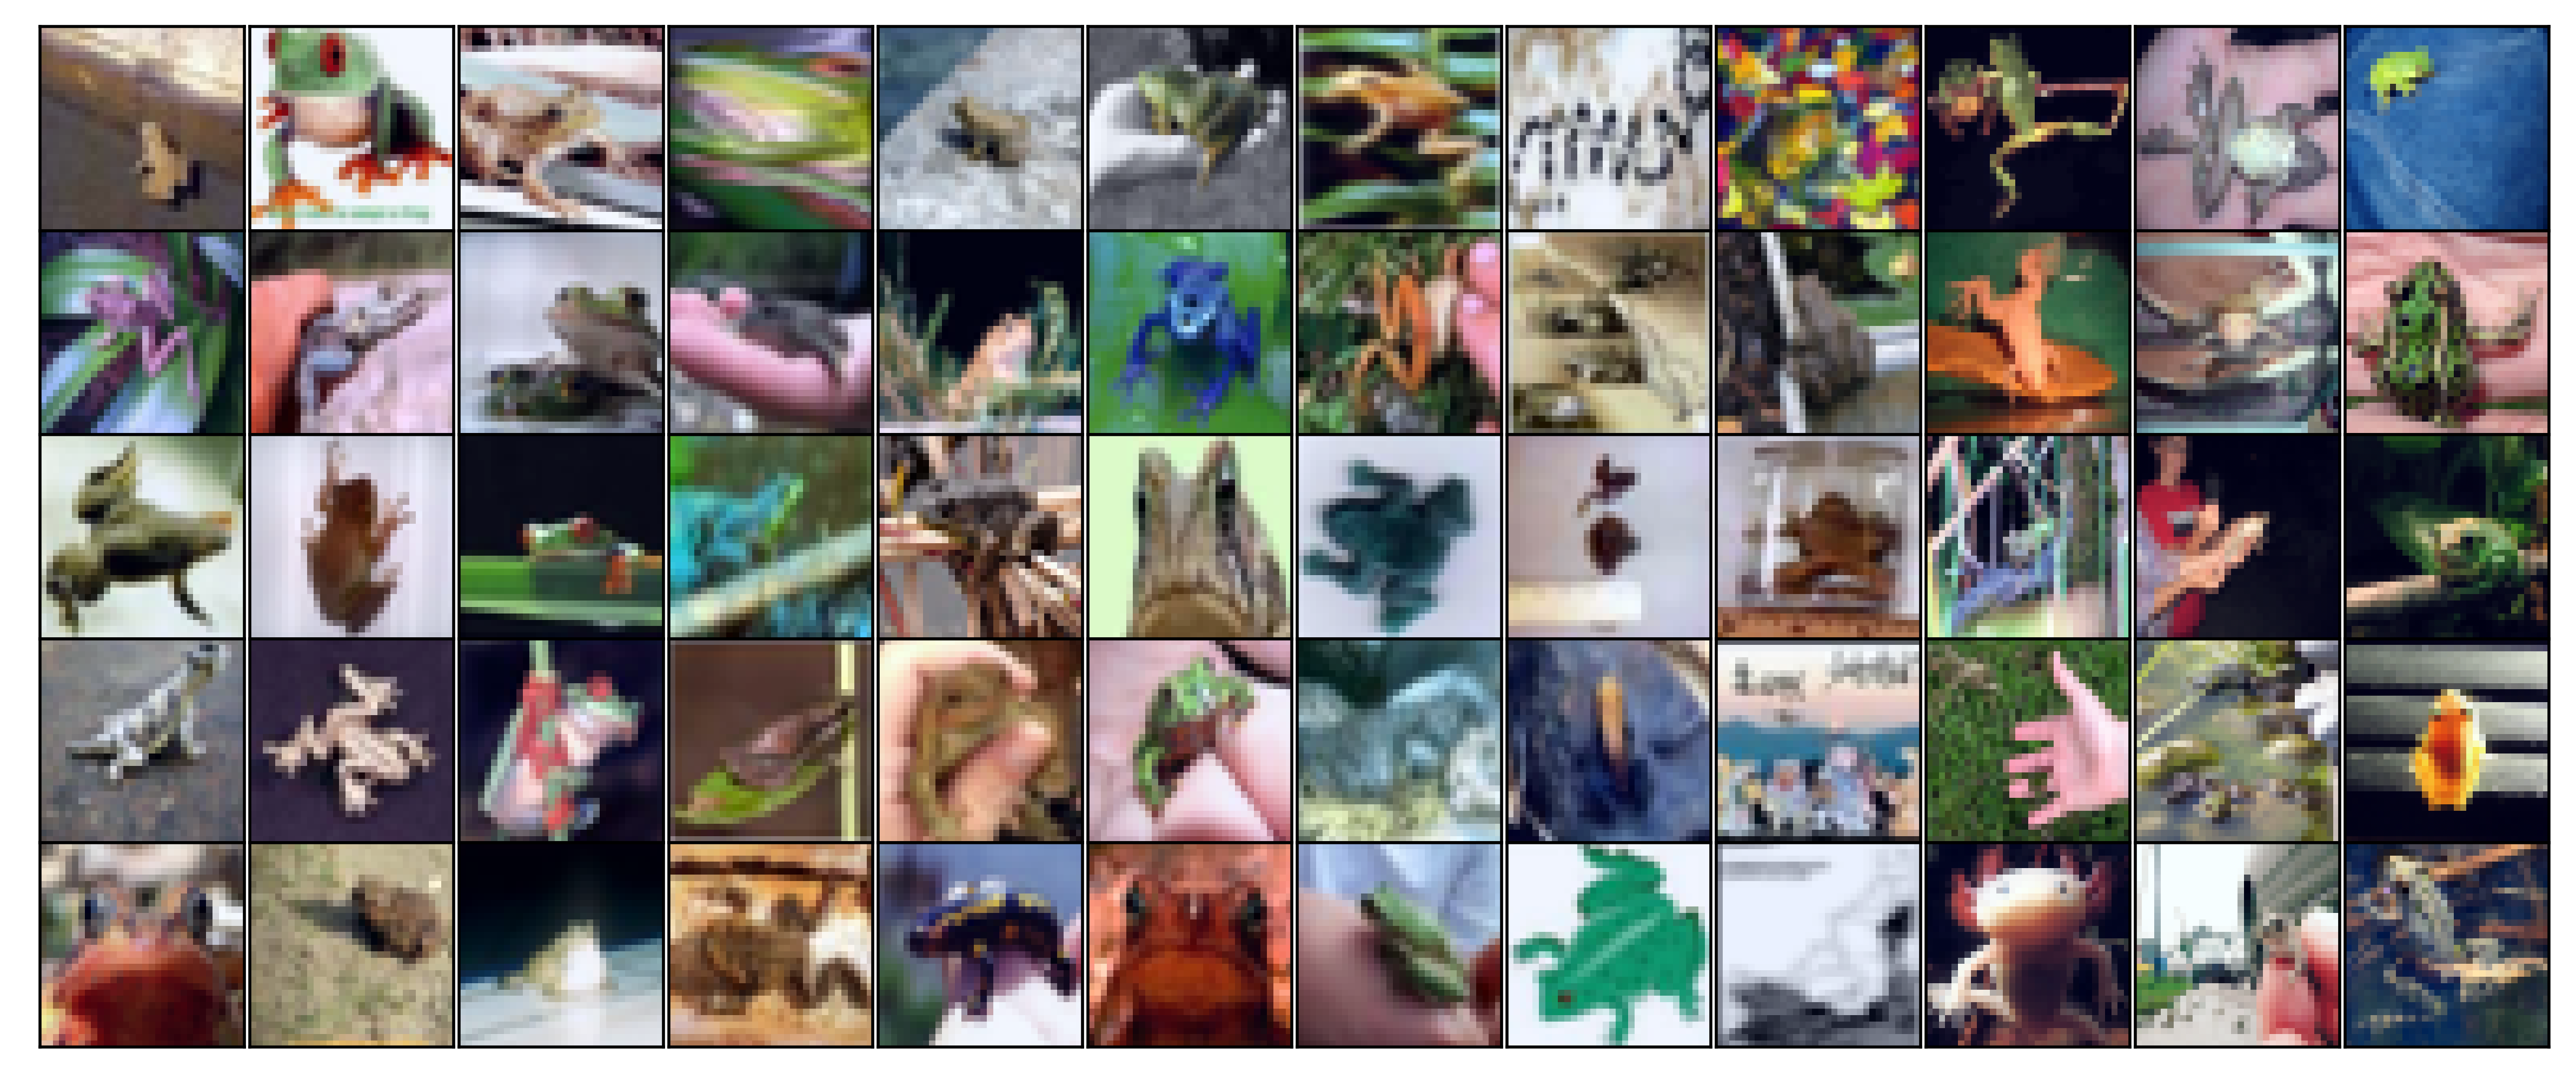}
    \includegraphics[width=0.48\textwidth]{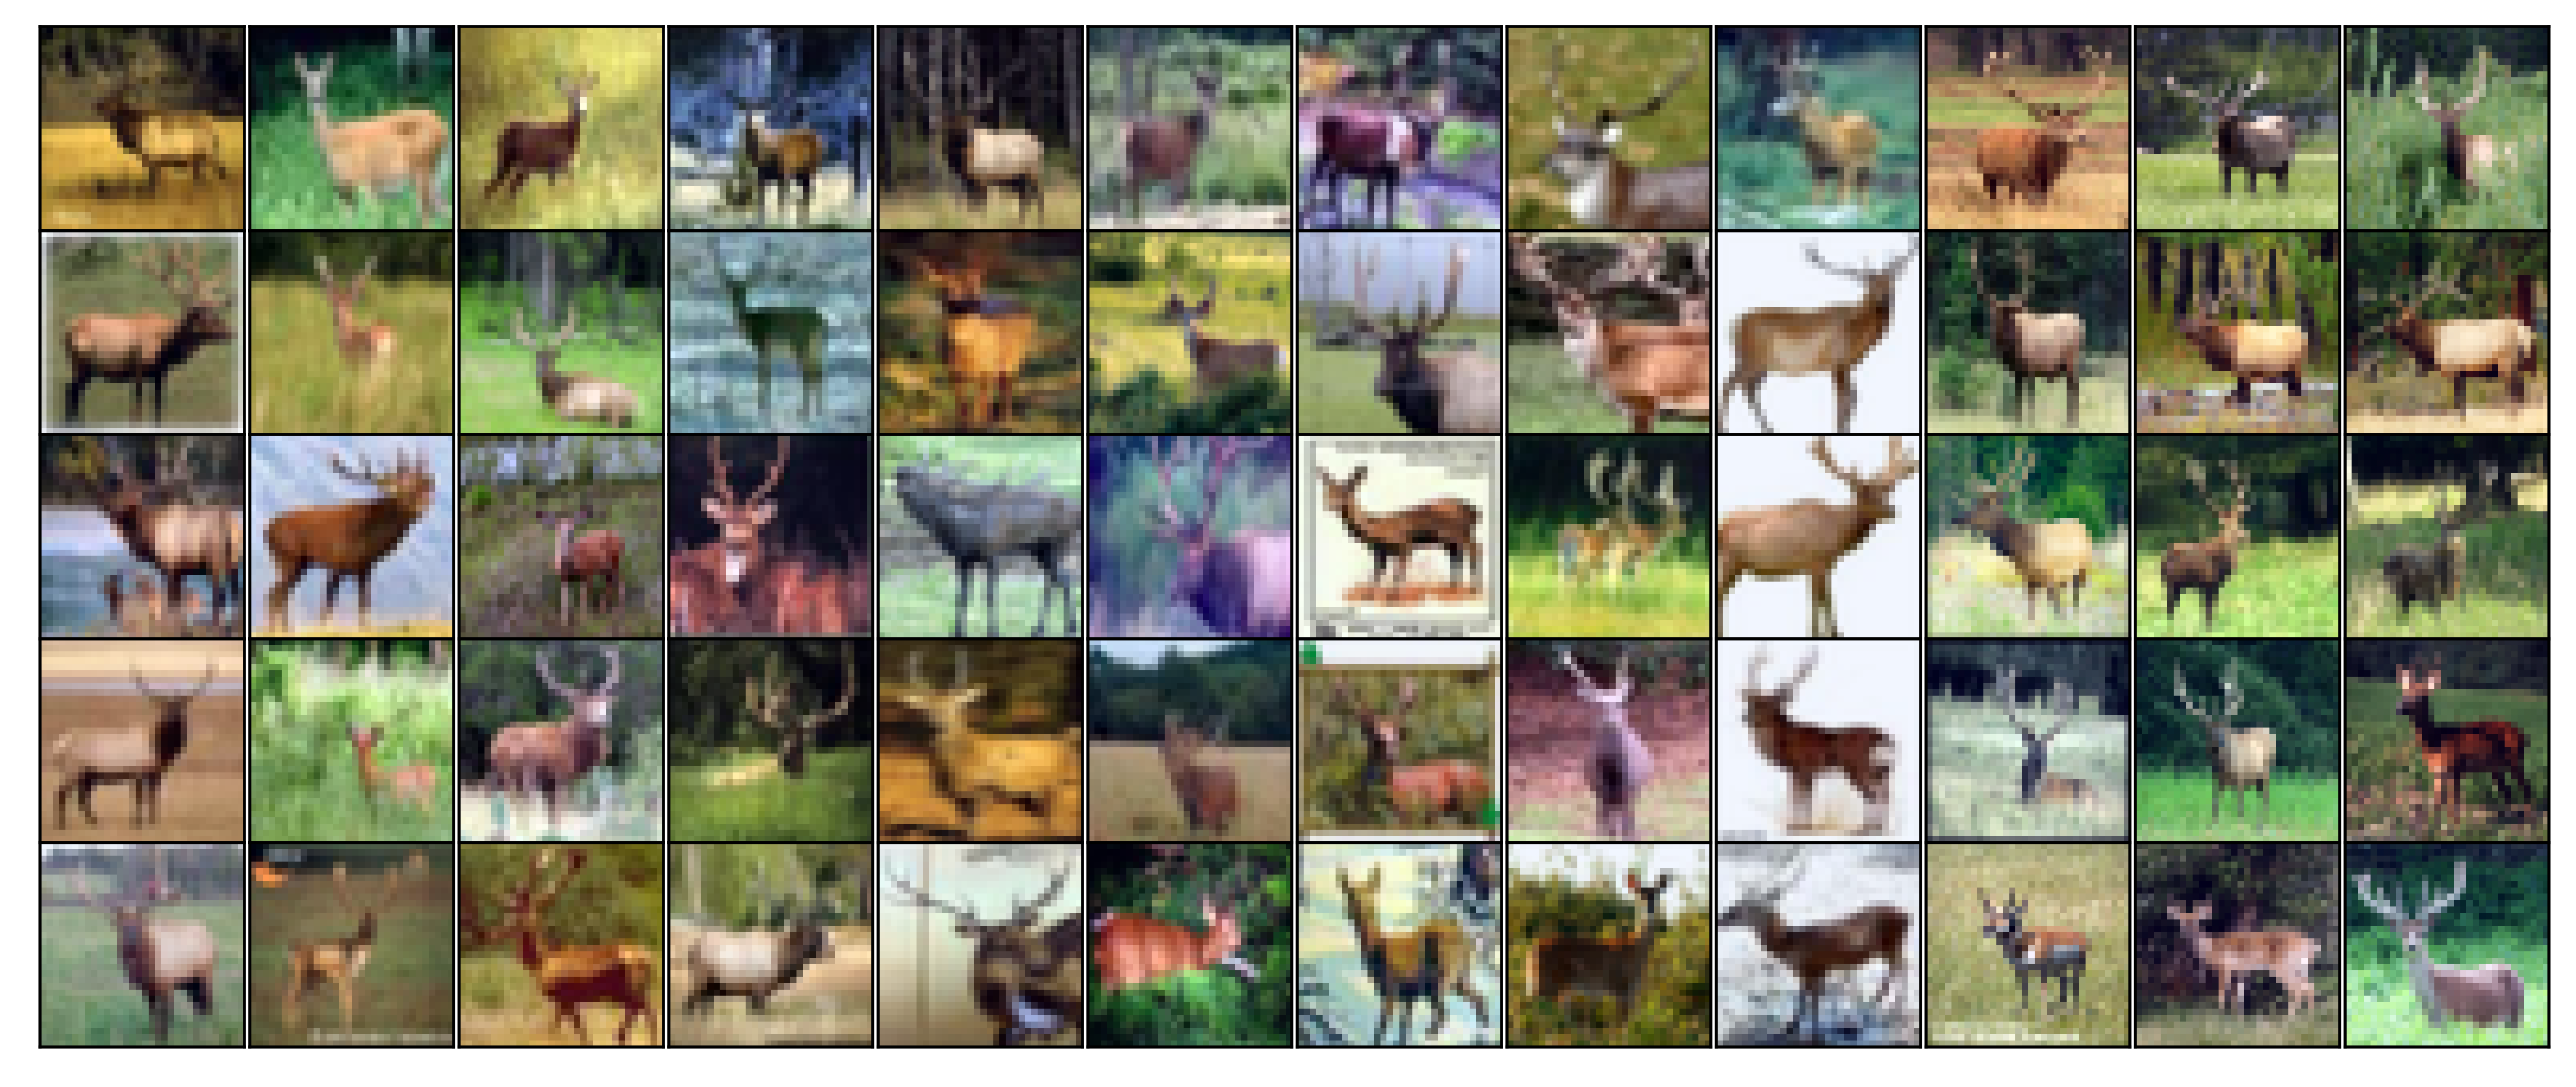} \hspace{3mm}
    \includegraphics[width=0.48\textwidth]{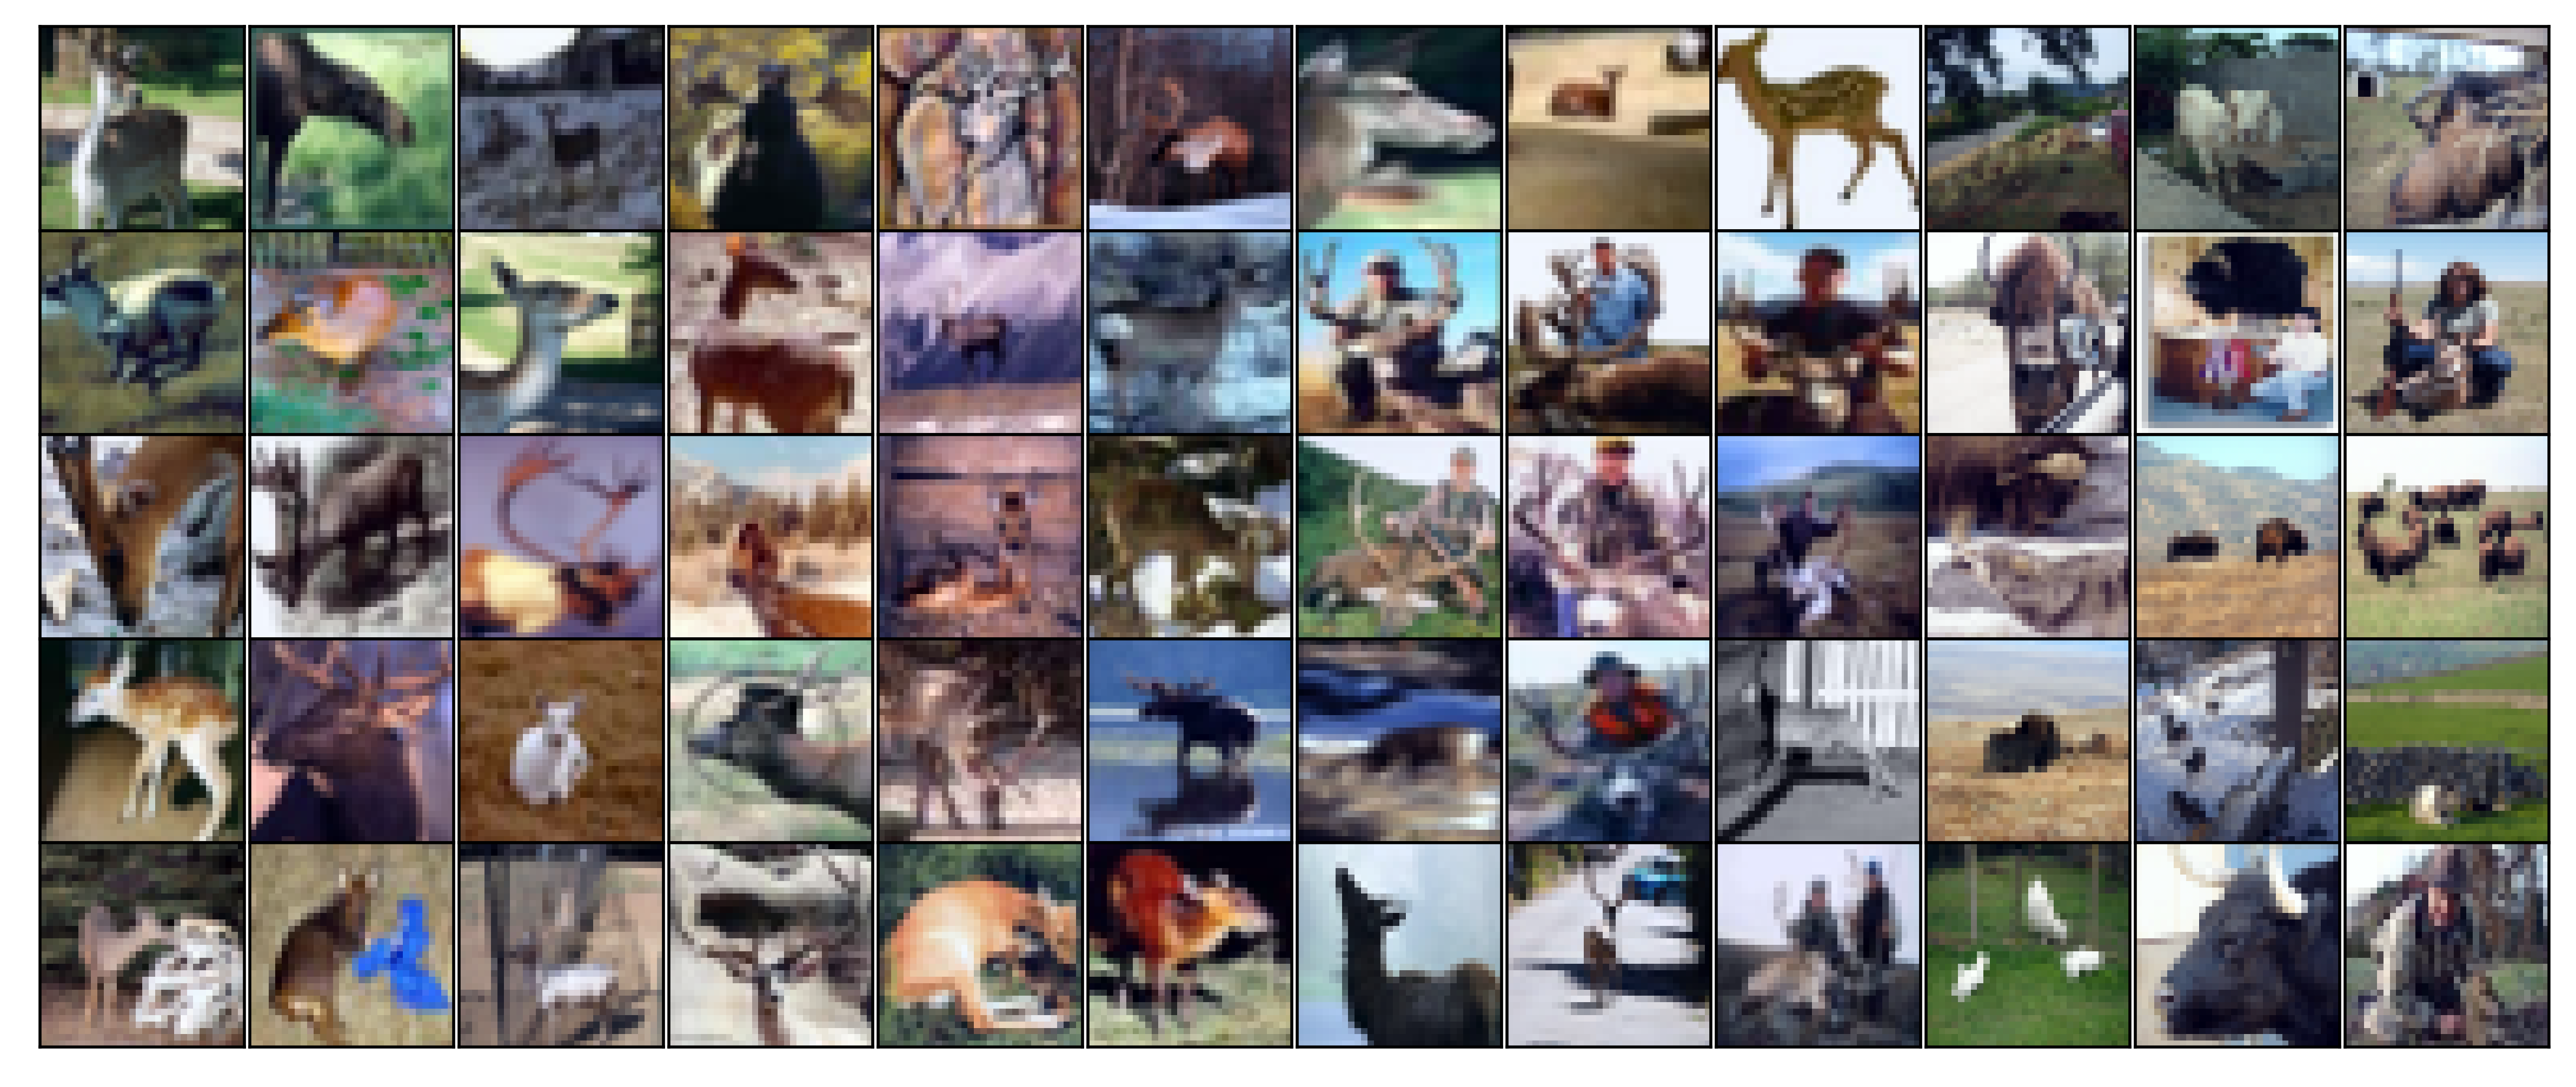}
    \includegraphics[width=0.48\textwidth]{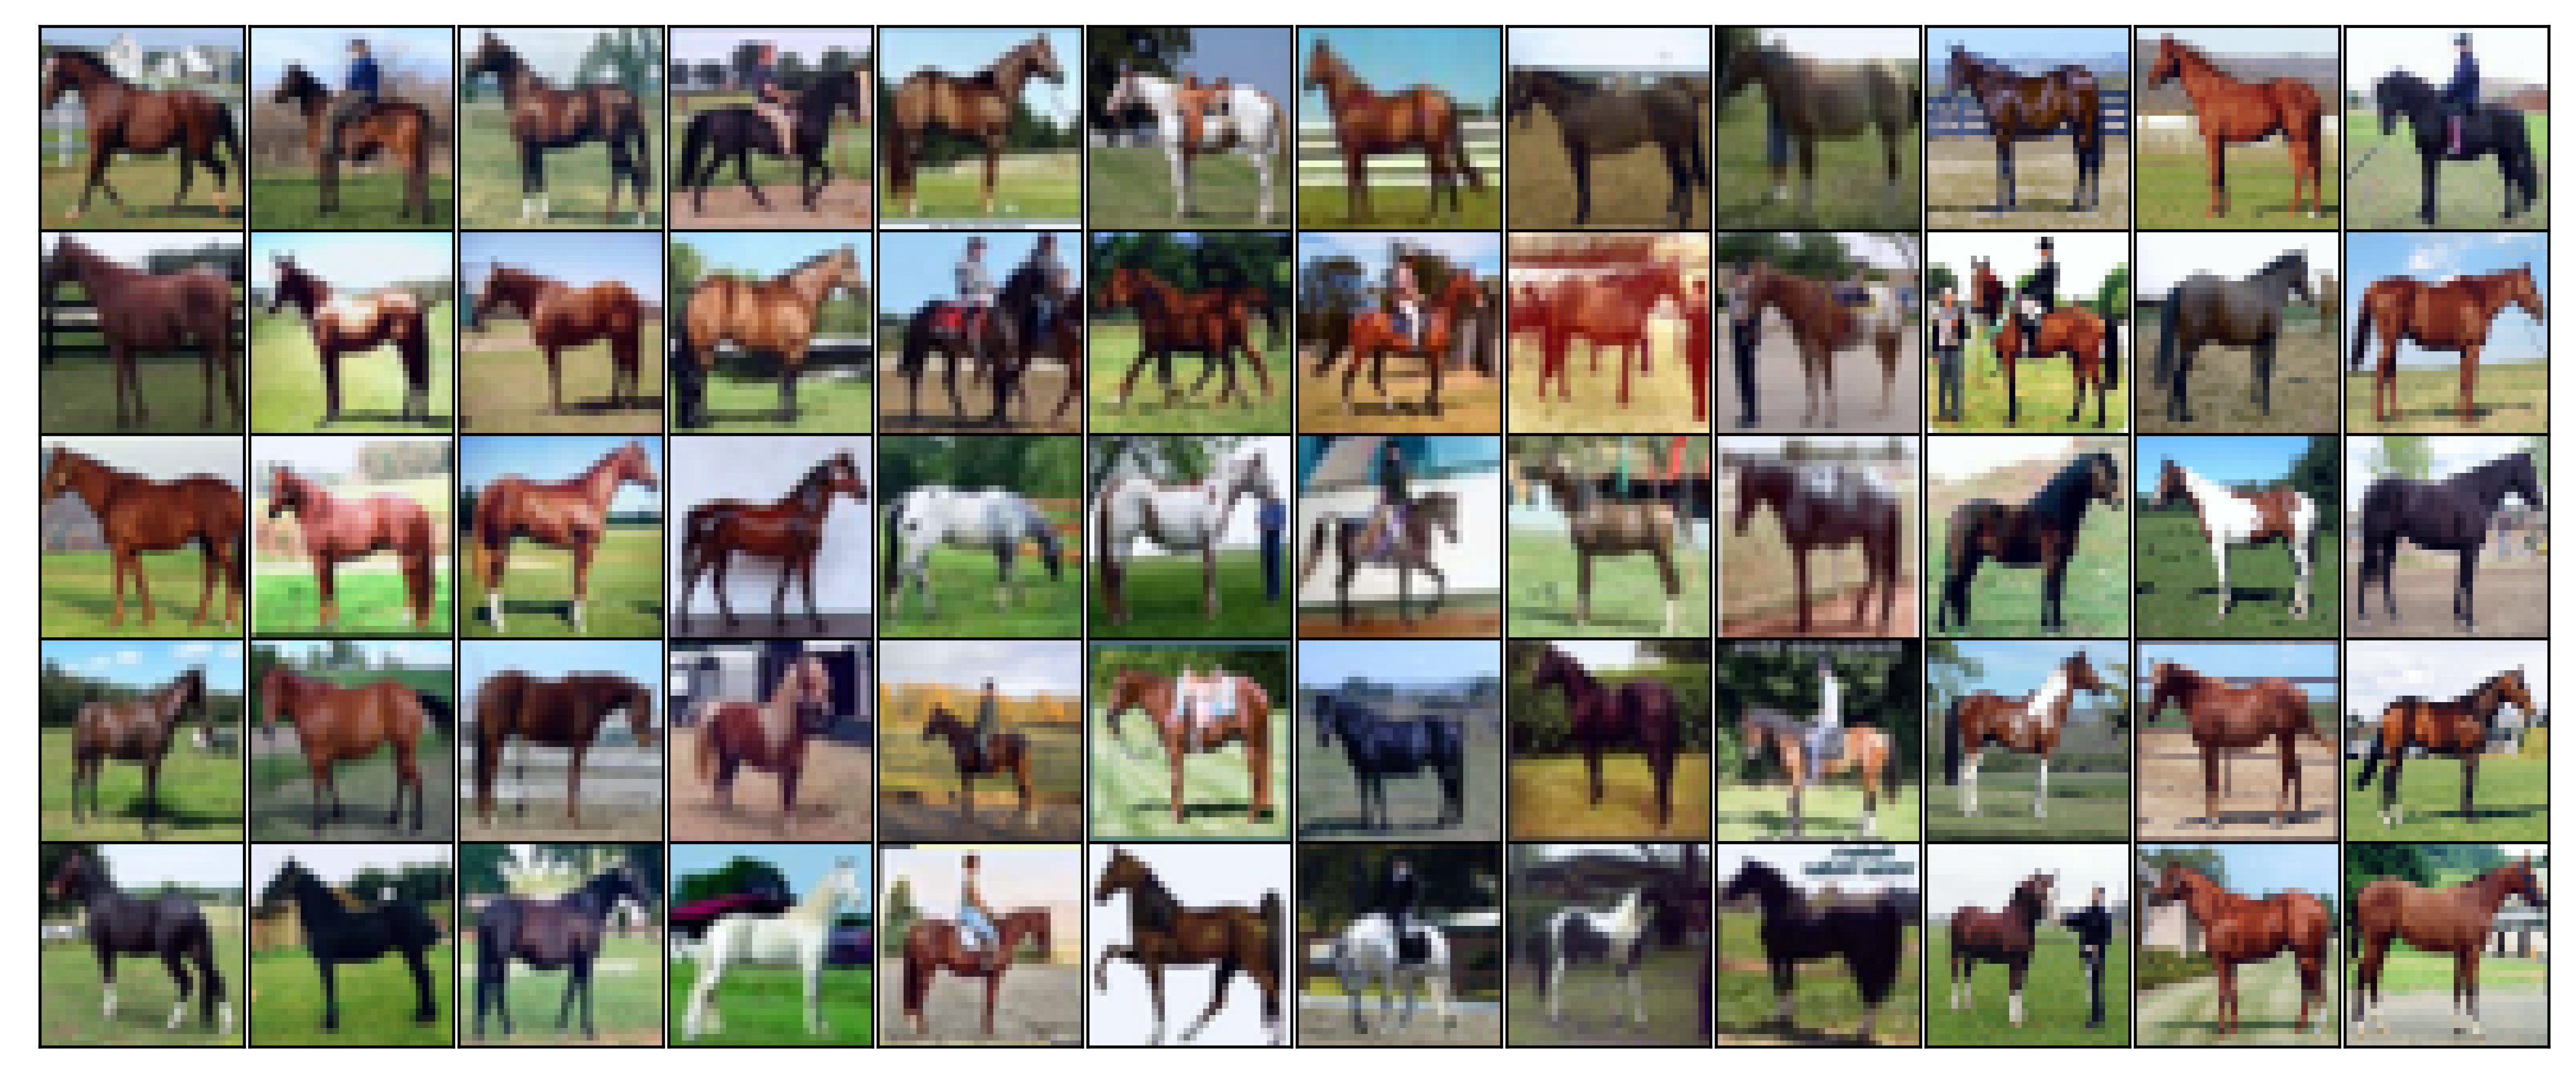} \hspace{3mm}
    \includegraphics[width=0.48\textwidth]{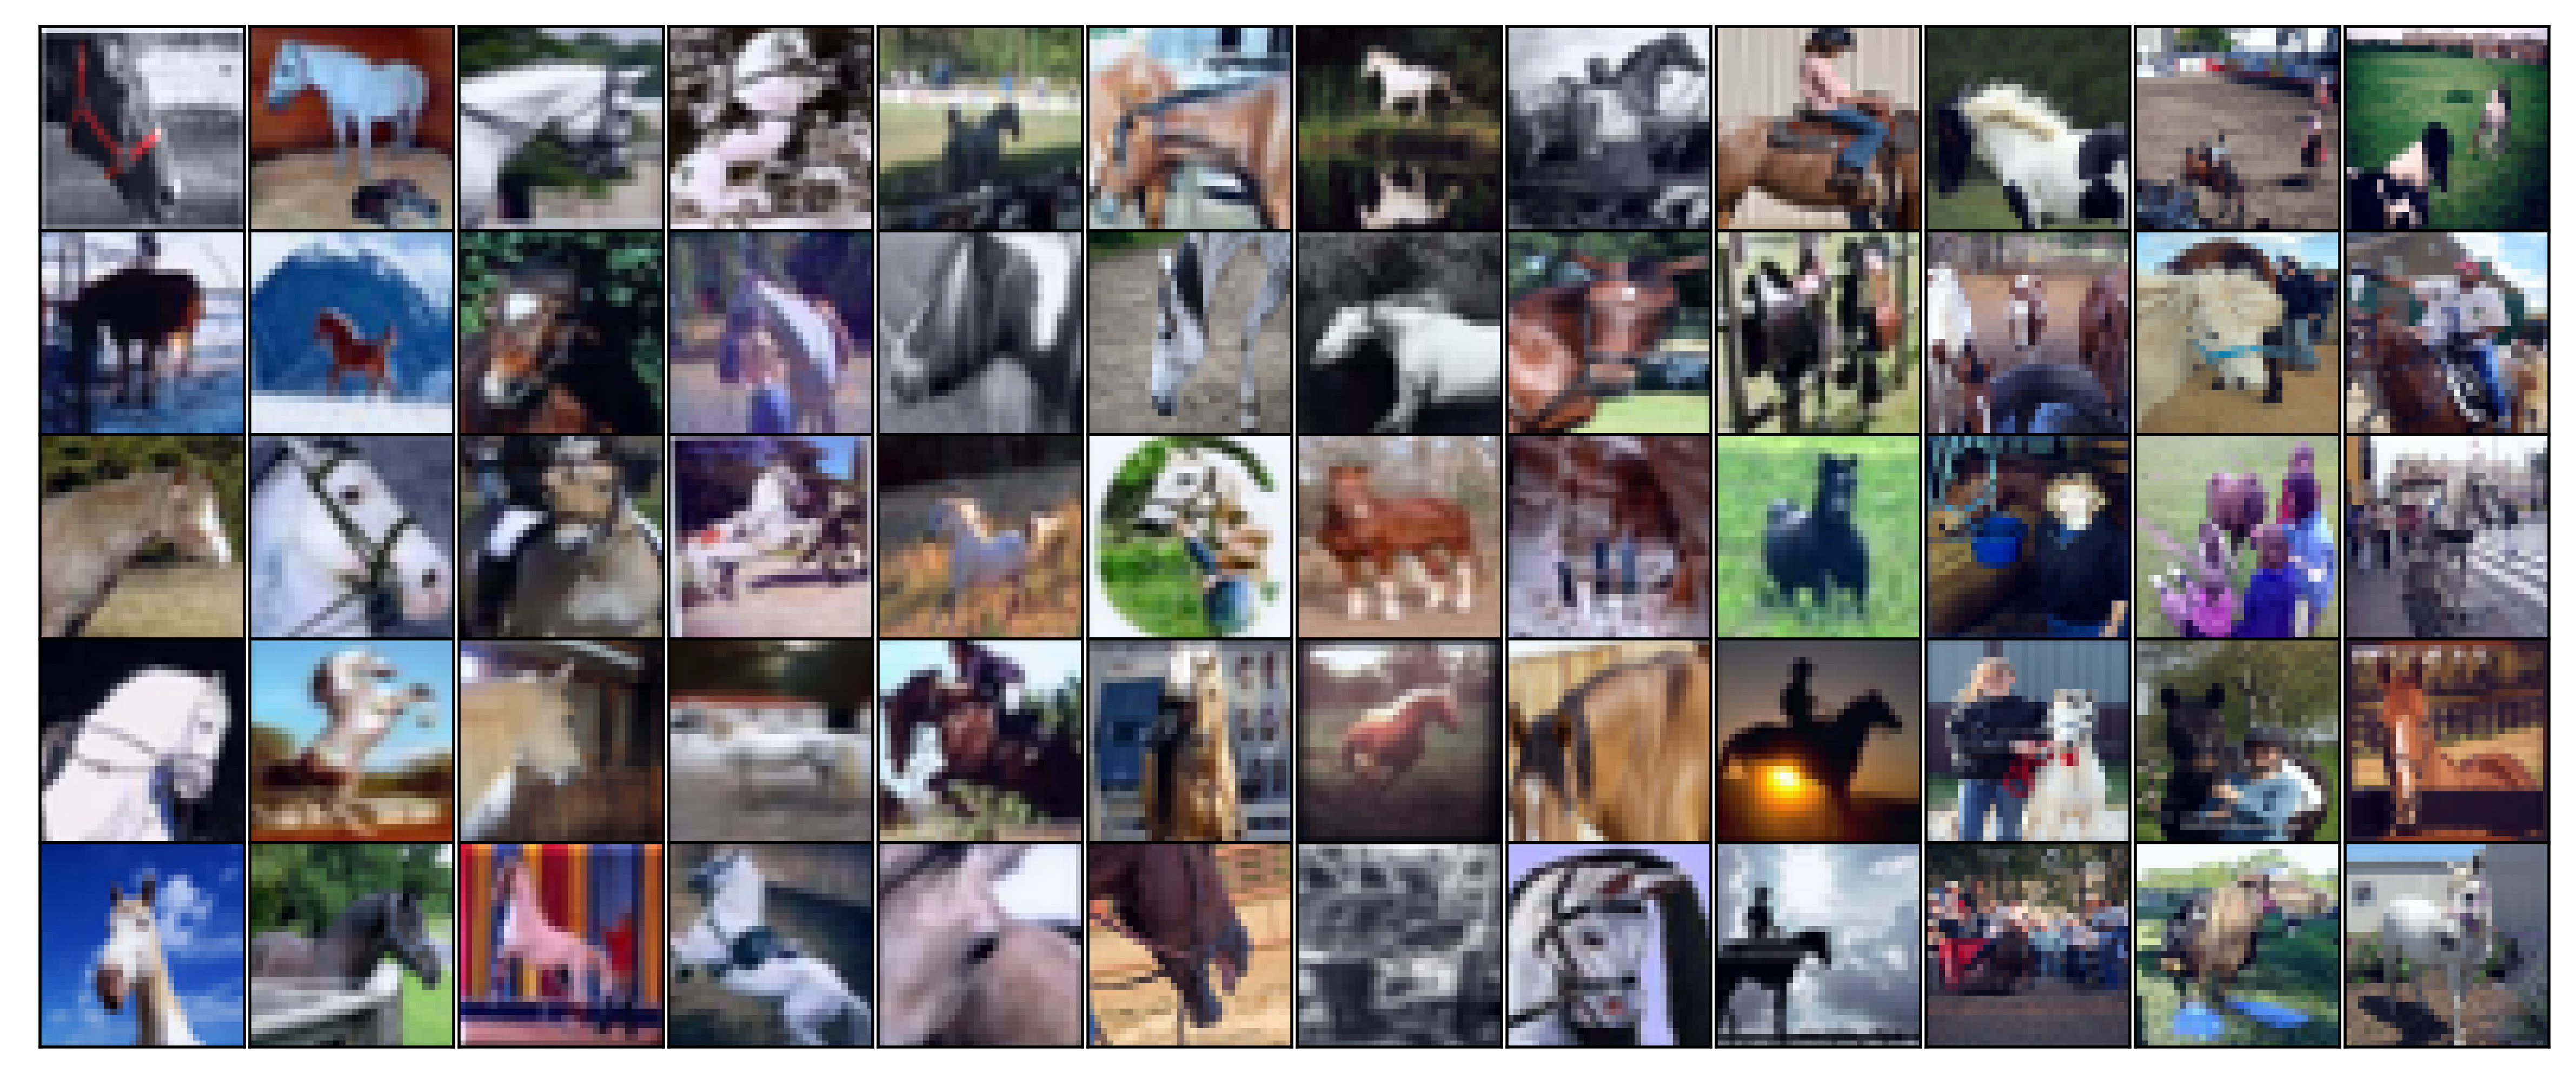}
    \includegraphics[width=0.48\textwidth]{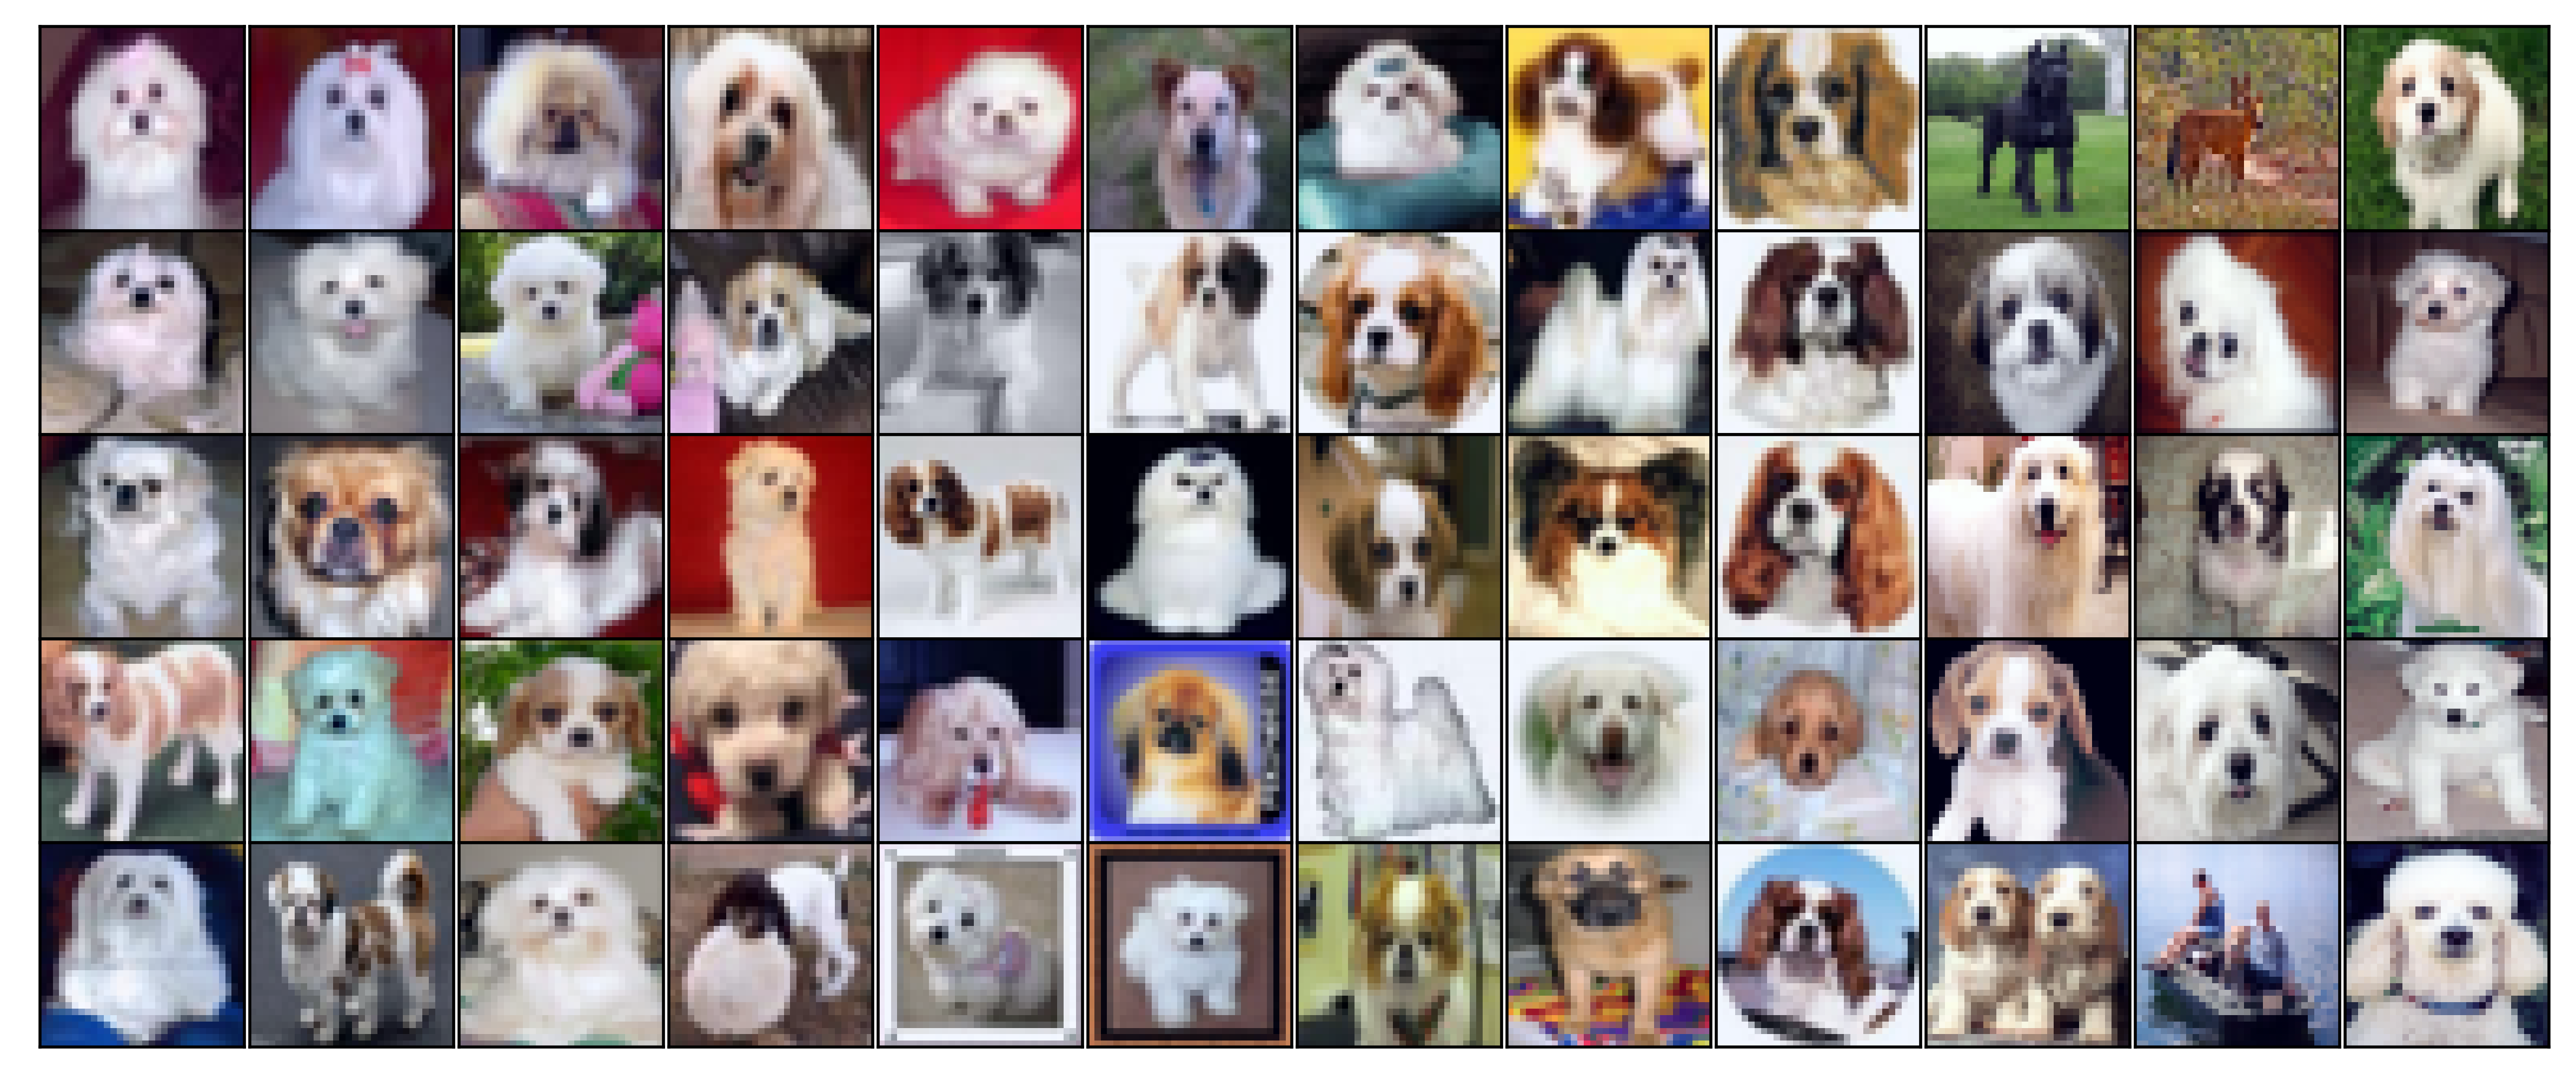} \hspace{3mm}
    \includegraphics[width=0.48\textwidth]{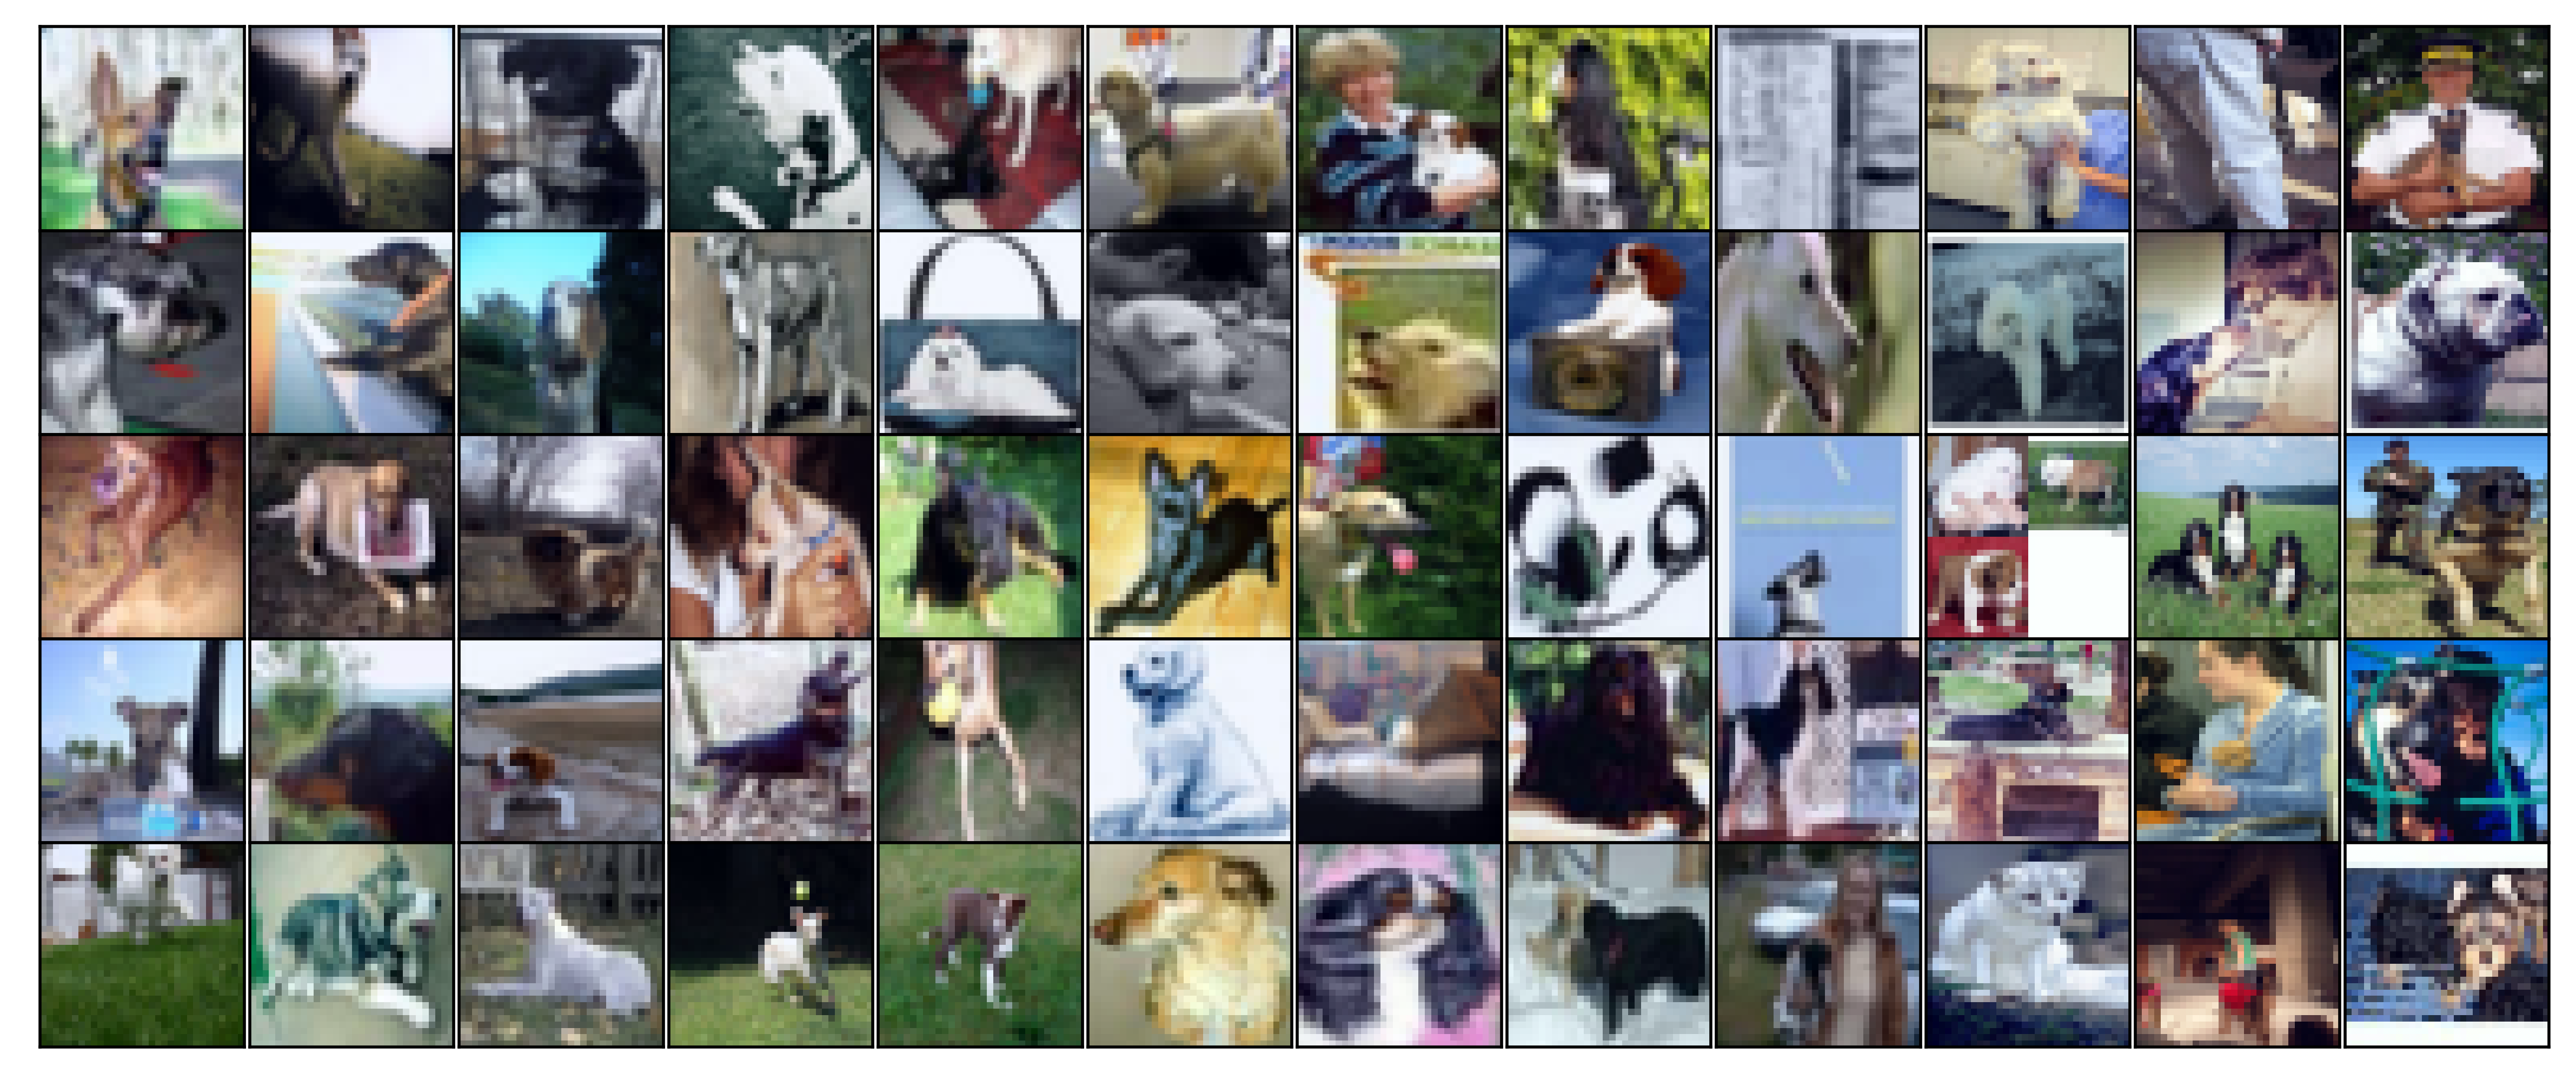}
    \includegraphics[width=0.48\textwidth]{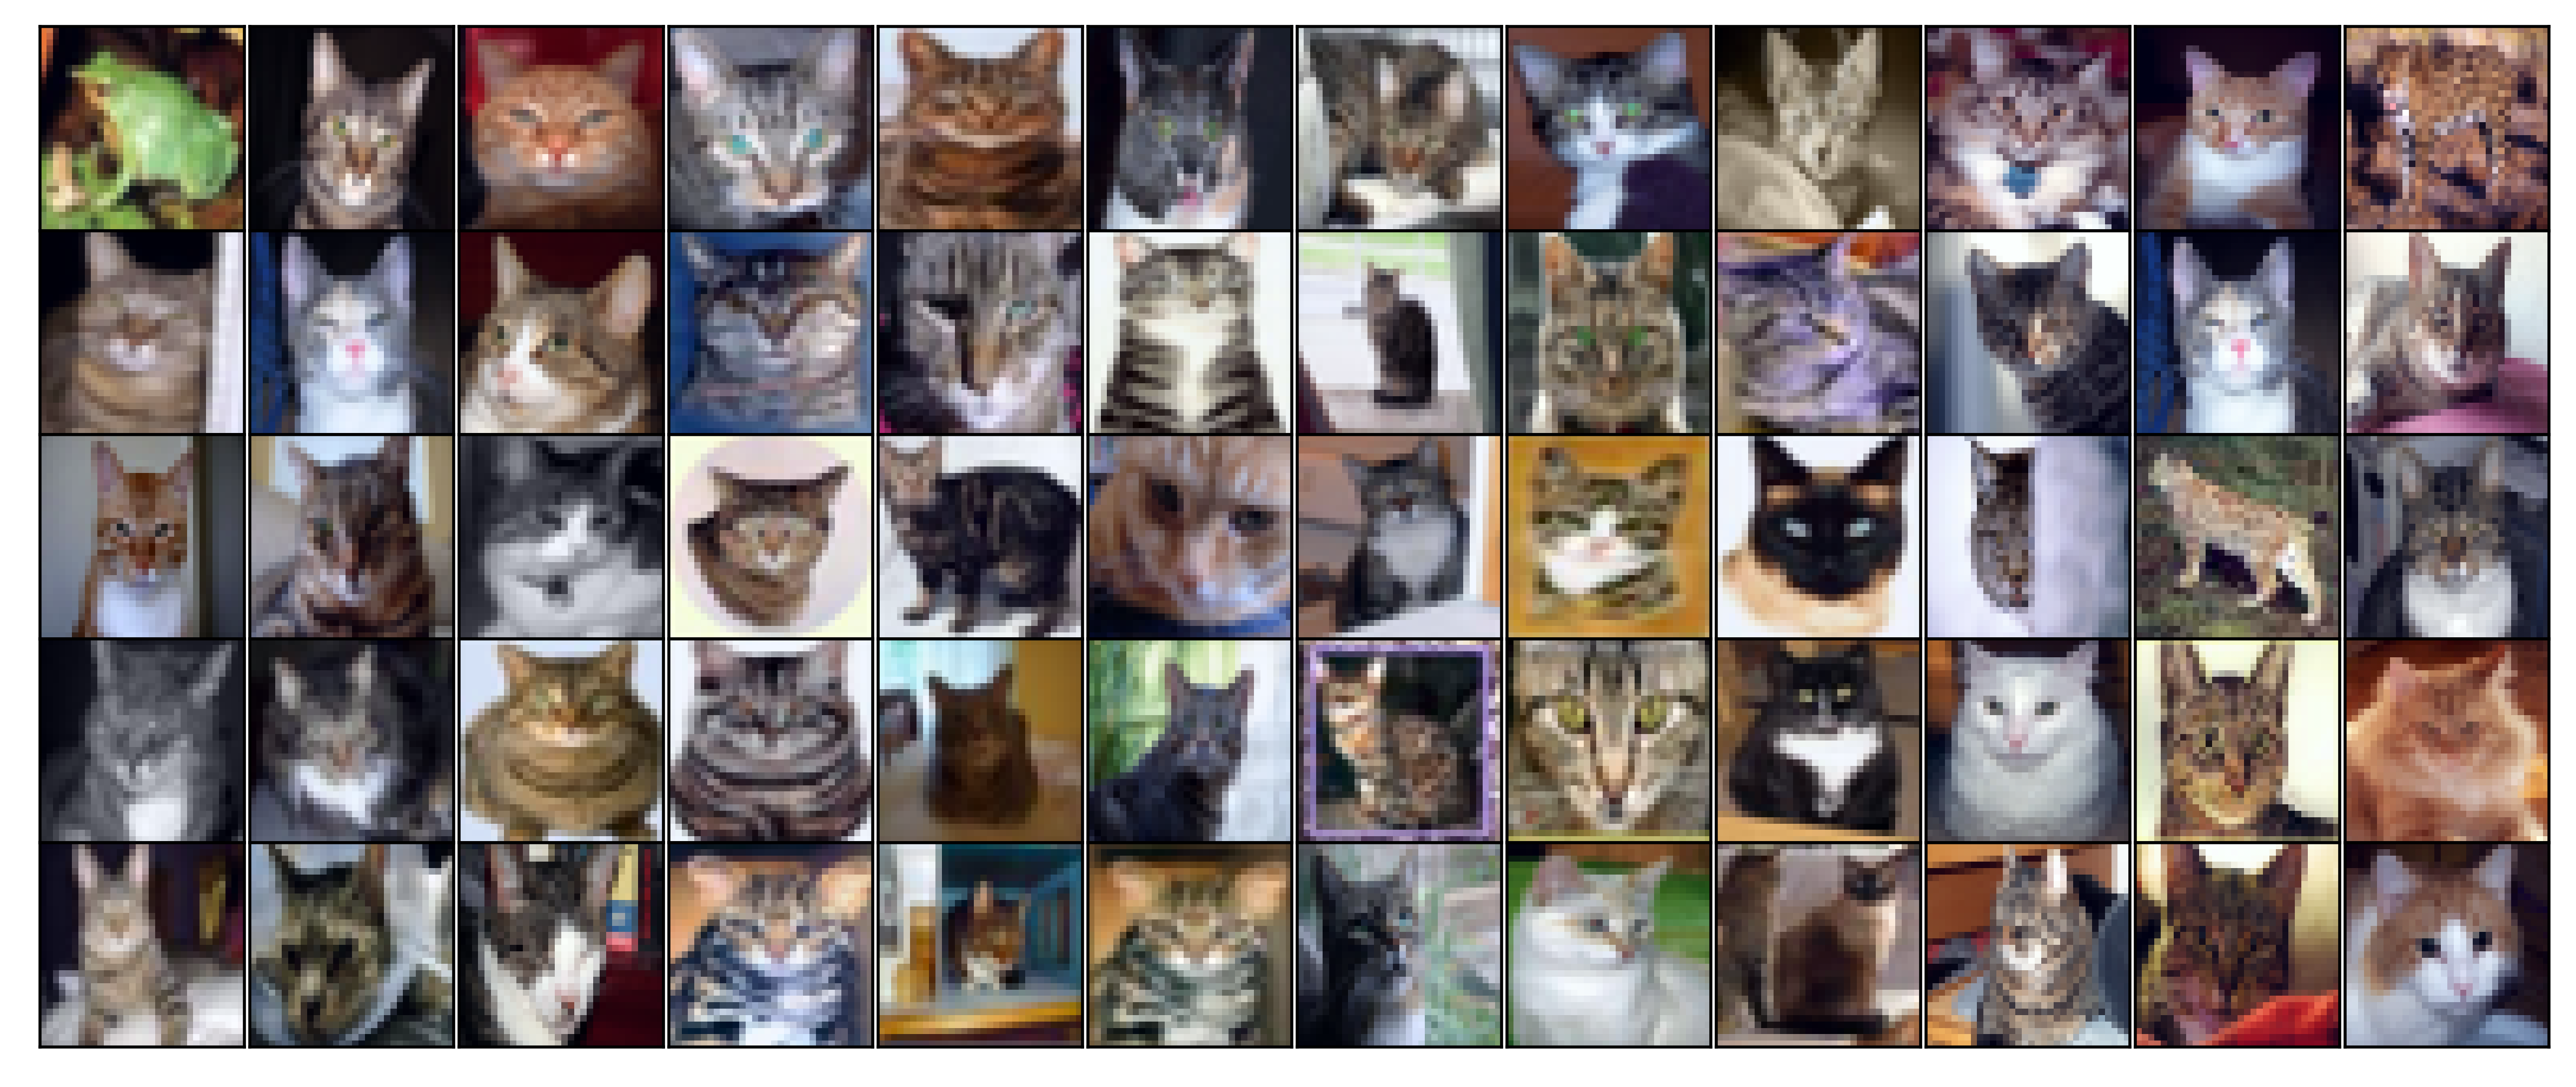} \hspace{3mm}
    \includegraphics[width=0.48\textwidth]{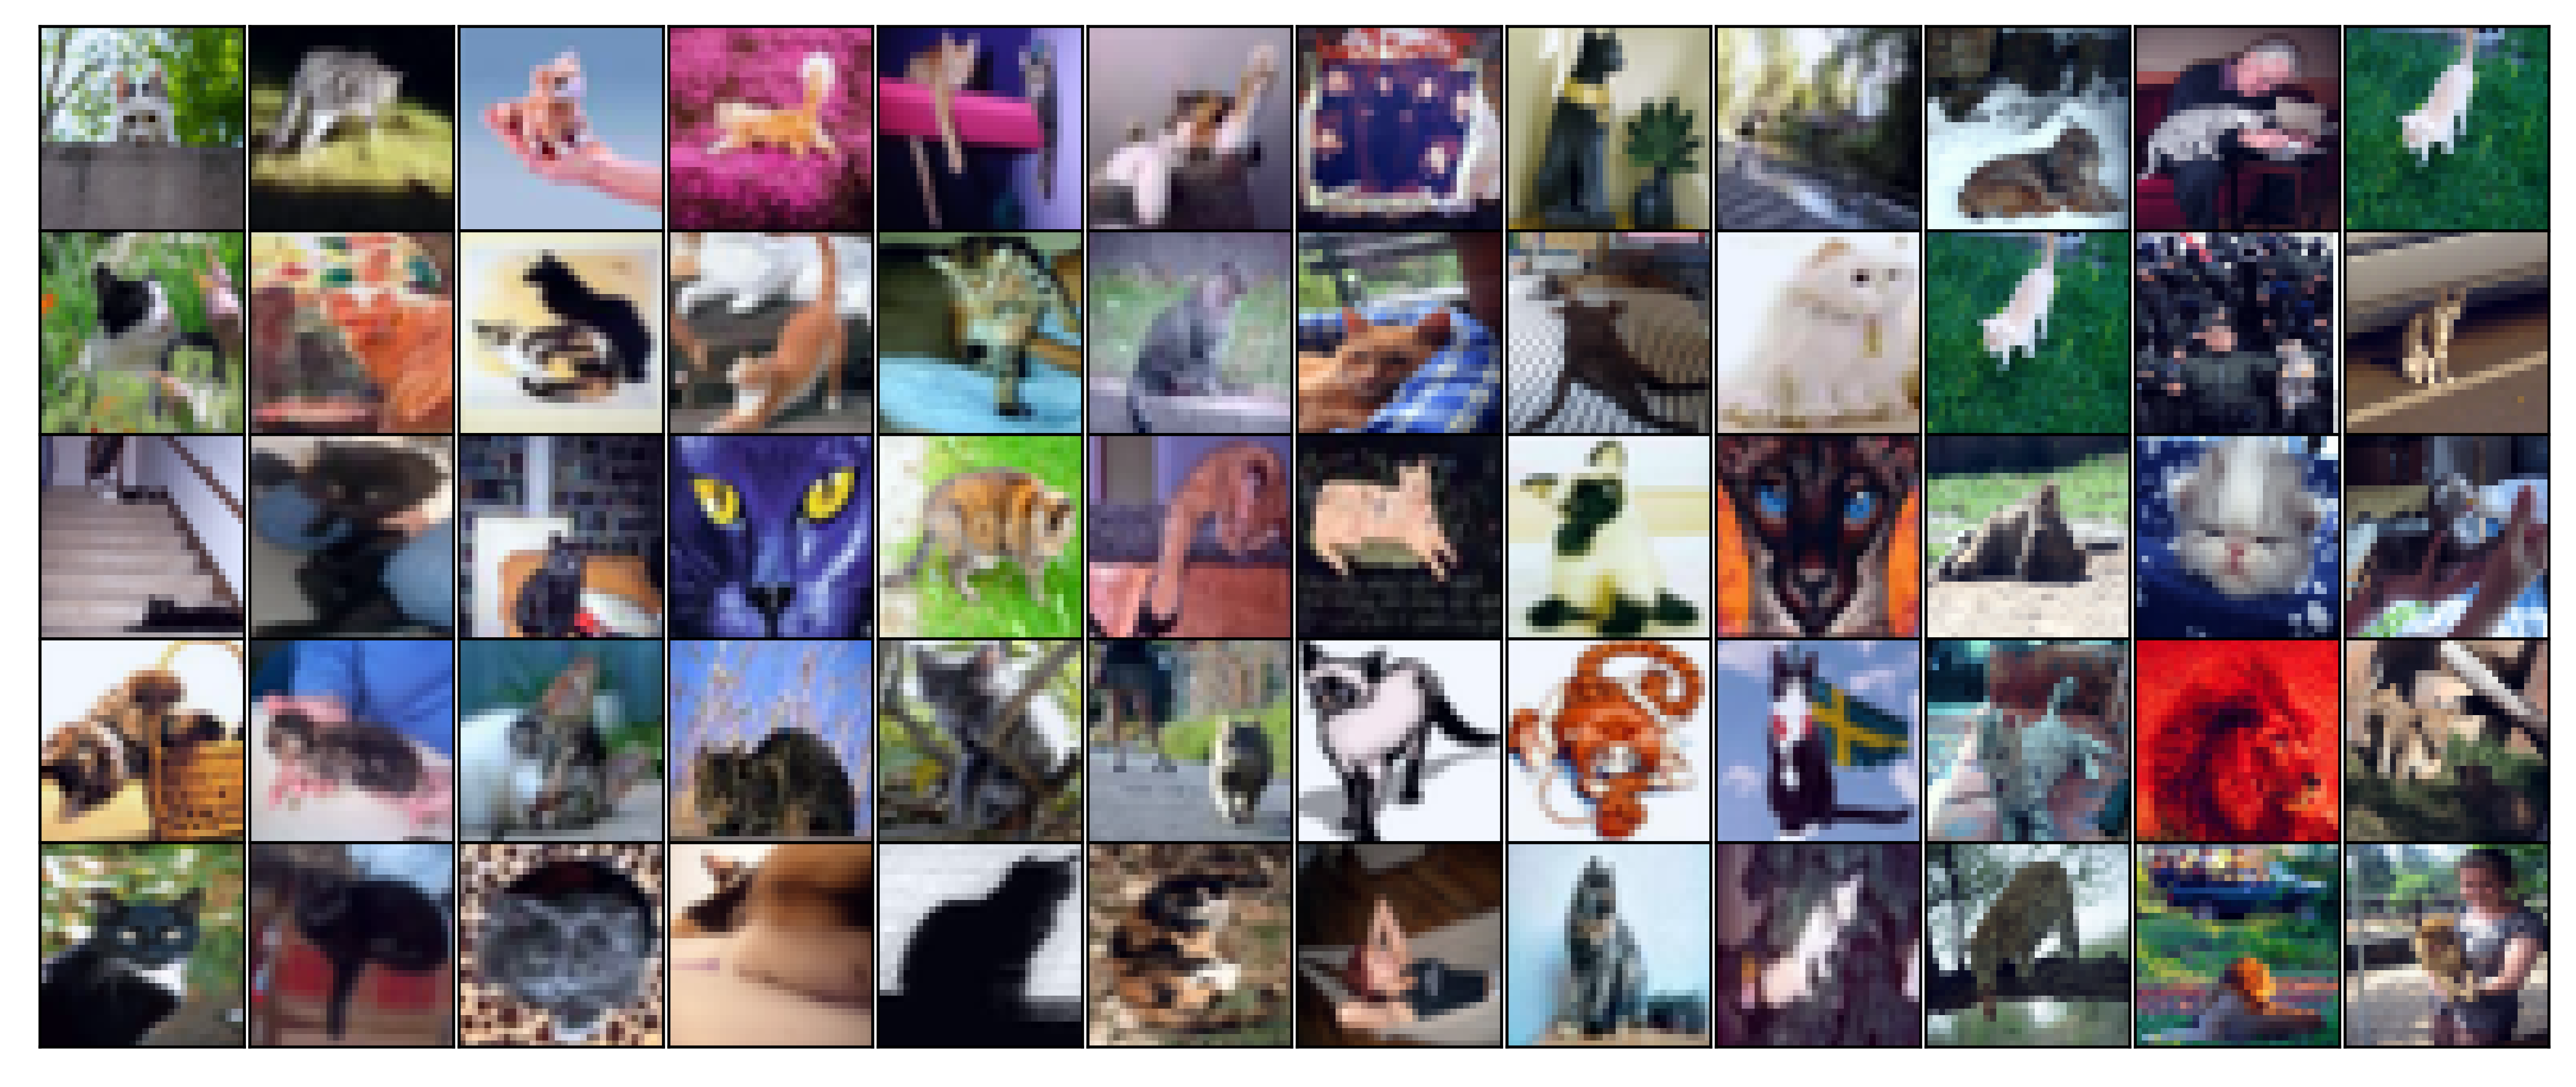} 
   \end{center}
  \vspace{-0.3cm}
  \caption{\label{fig:low-high-entropy-app2} \textbf{Left: lowest entropy images; Right: highest entropy images from the CIFAR-10 test dataset (ID) and three OOD datasets (CIFAR-10.1, CIFAR-10.2, and CINIC-10)}} 
\end{figure}

\subsection{Low entropy images with spurious correlations}

\begin{figure}[t!]
   \begin{center}
    \includegraphics[width=0.24\textwidth]{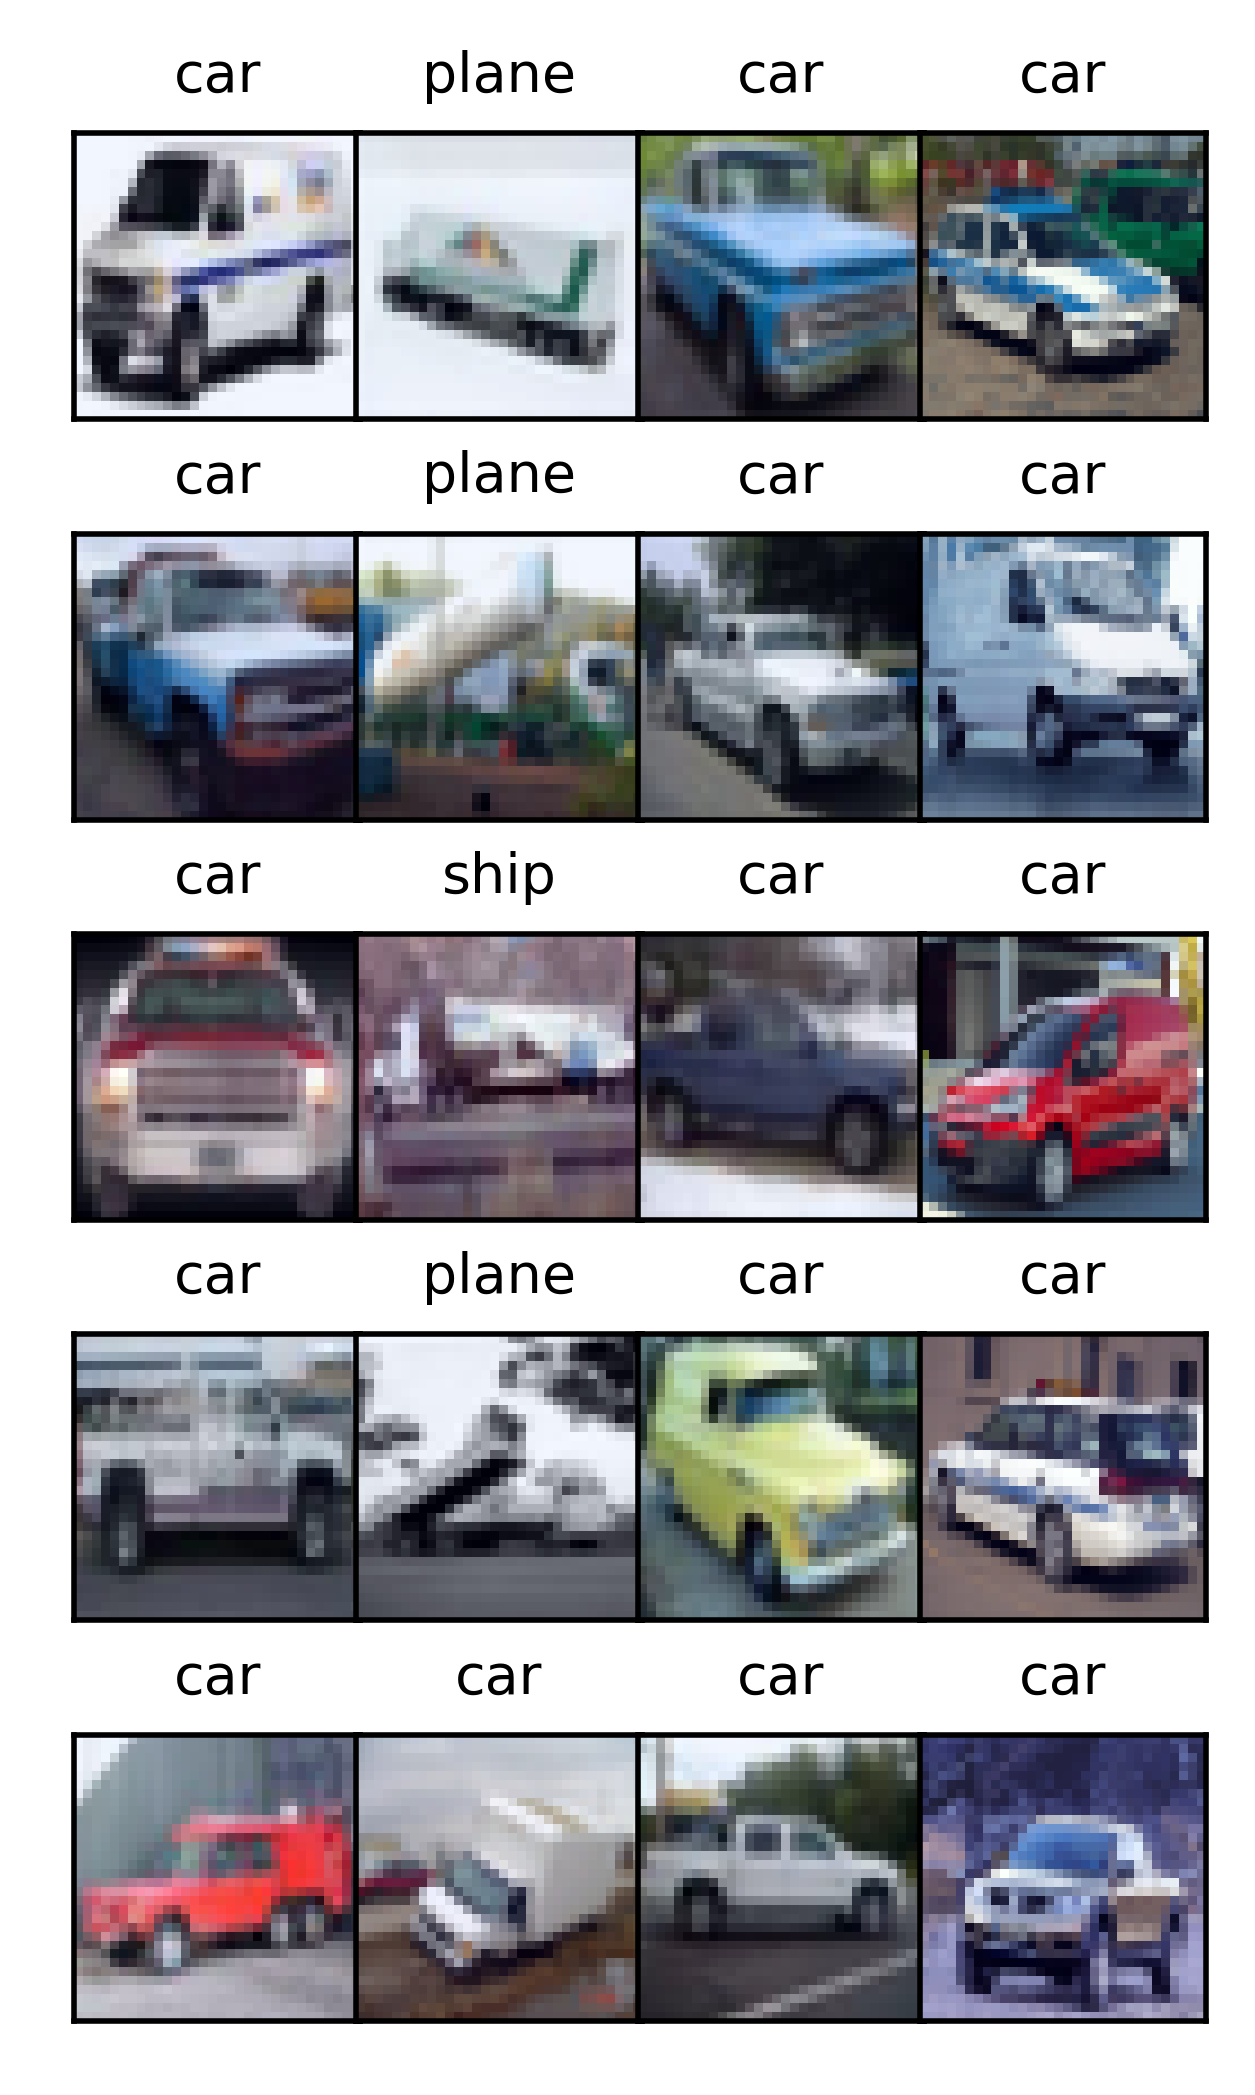}
    \includegraphics[width=0.24\textwidth]{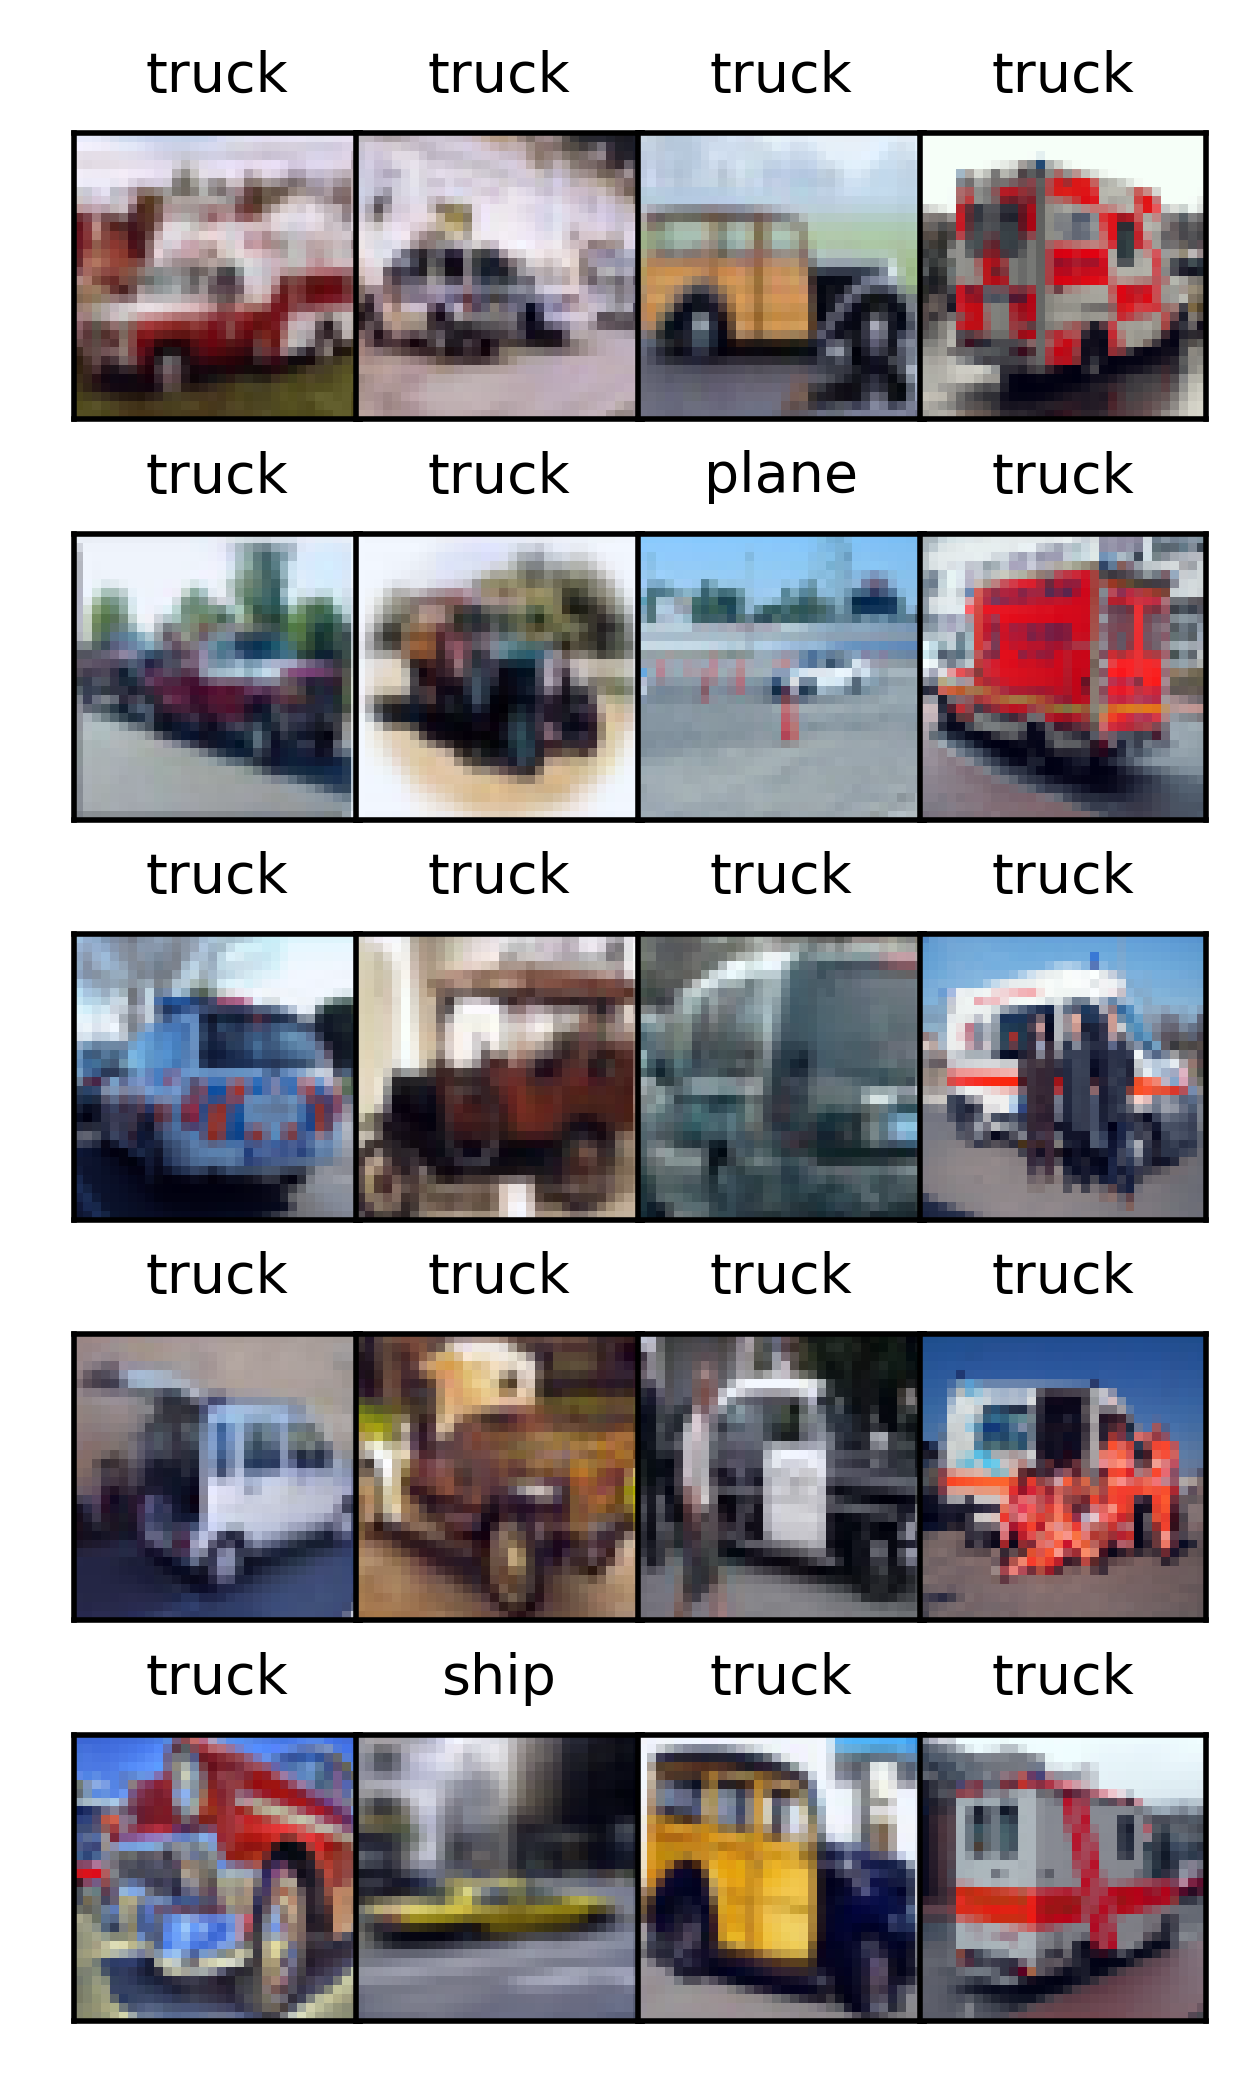} 
    \includegraphics[width=0.24\textwidth]{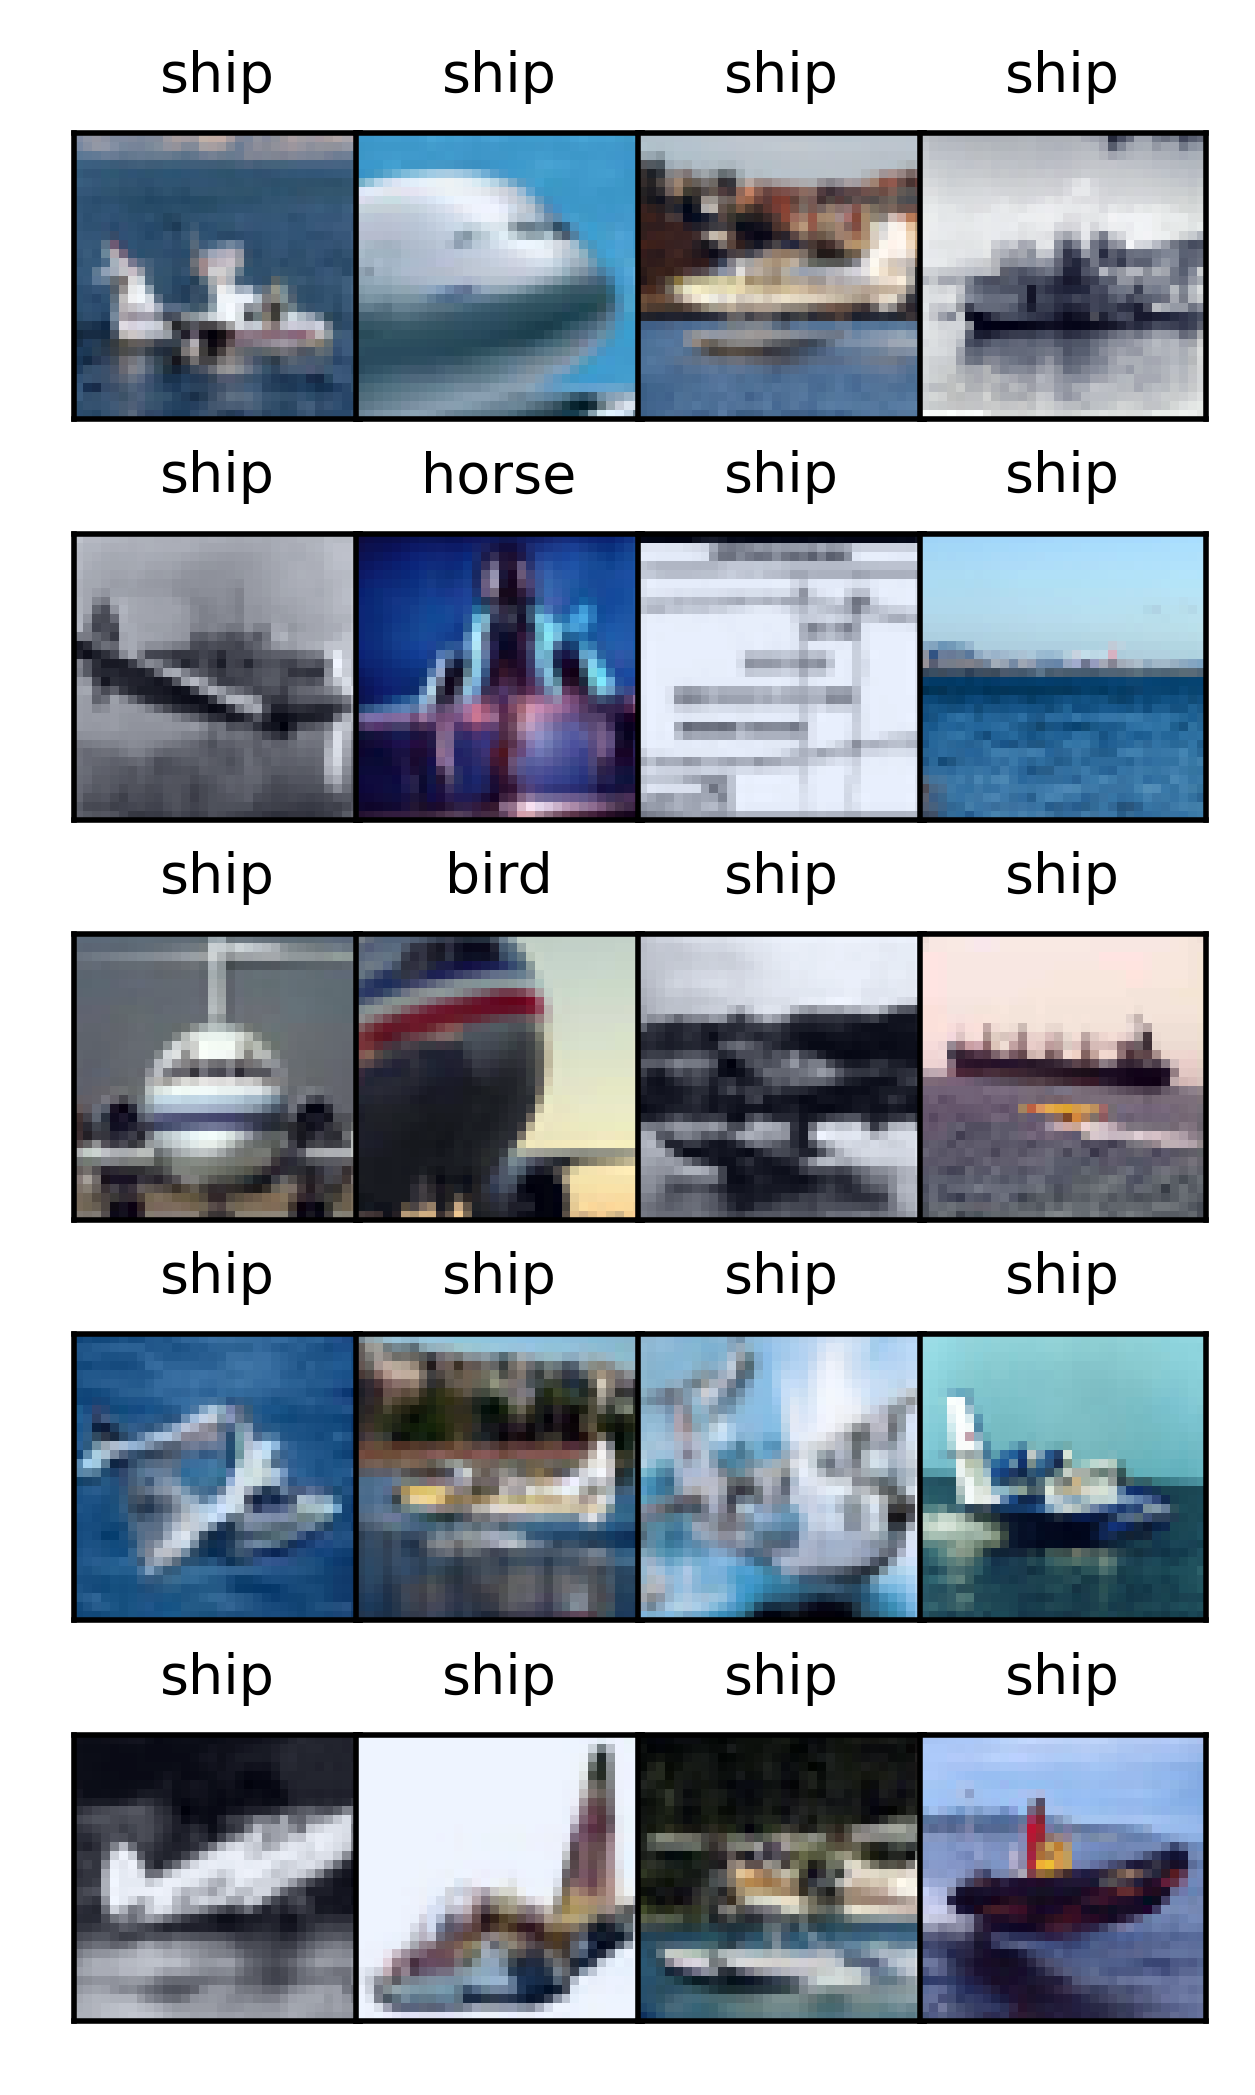} 
    \includegraphics[width=0.24\textwidth]{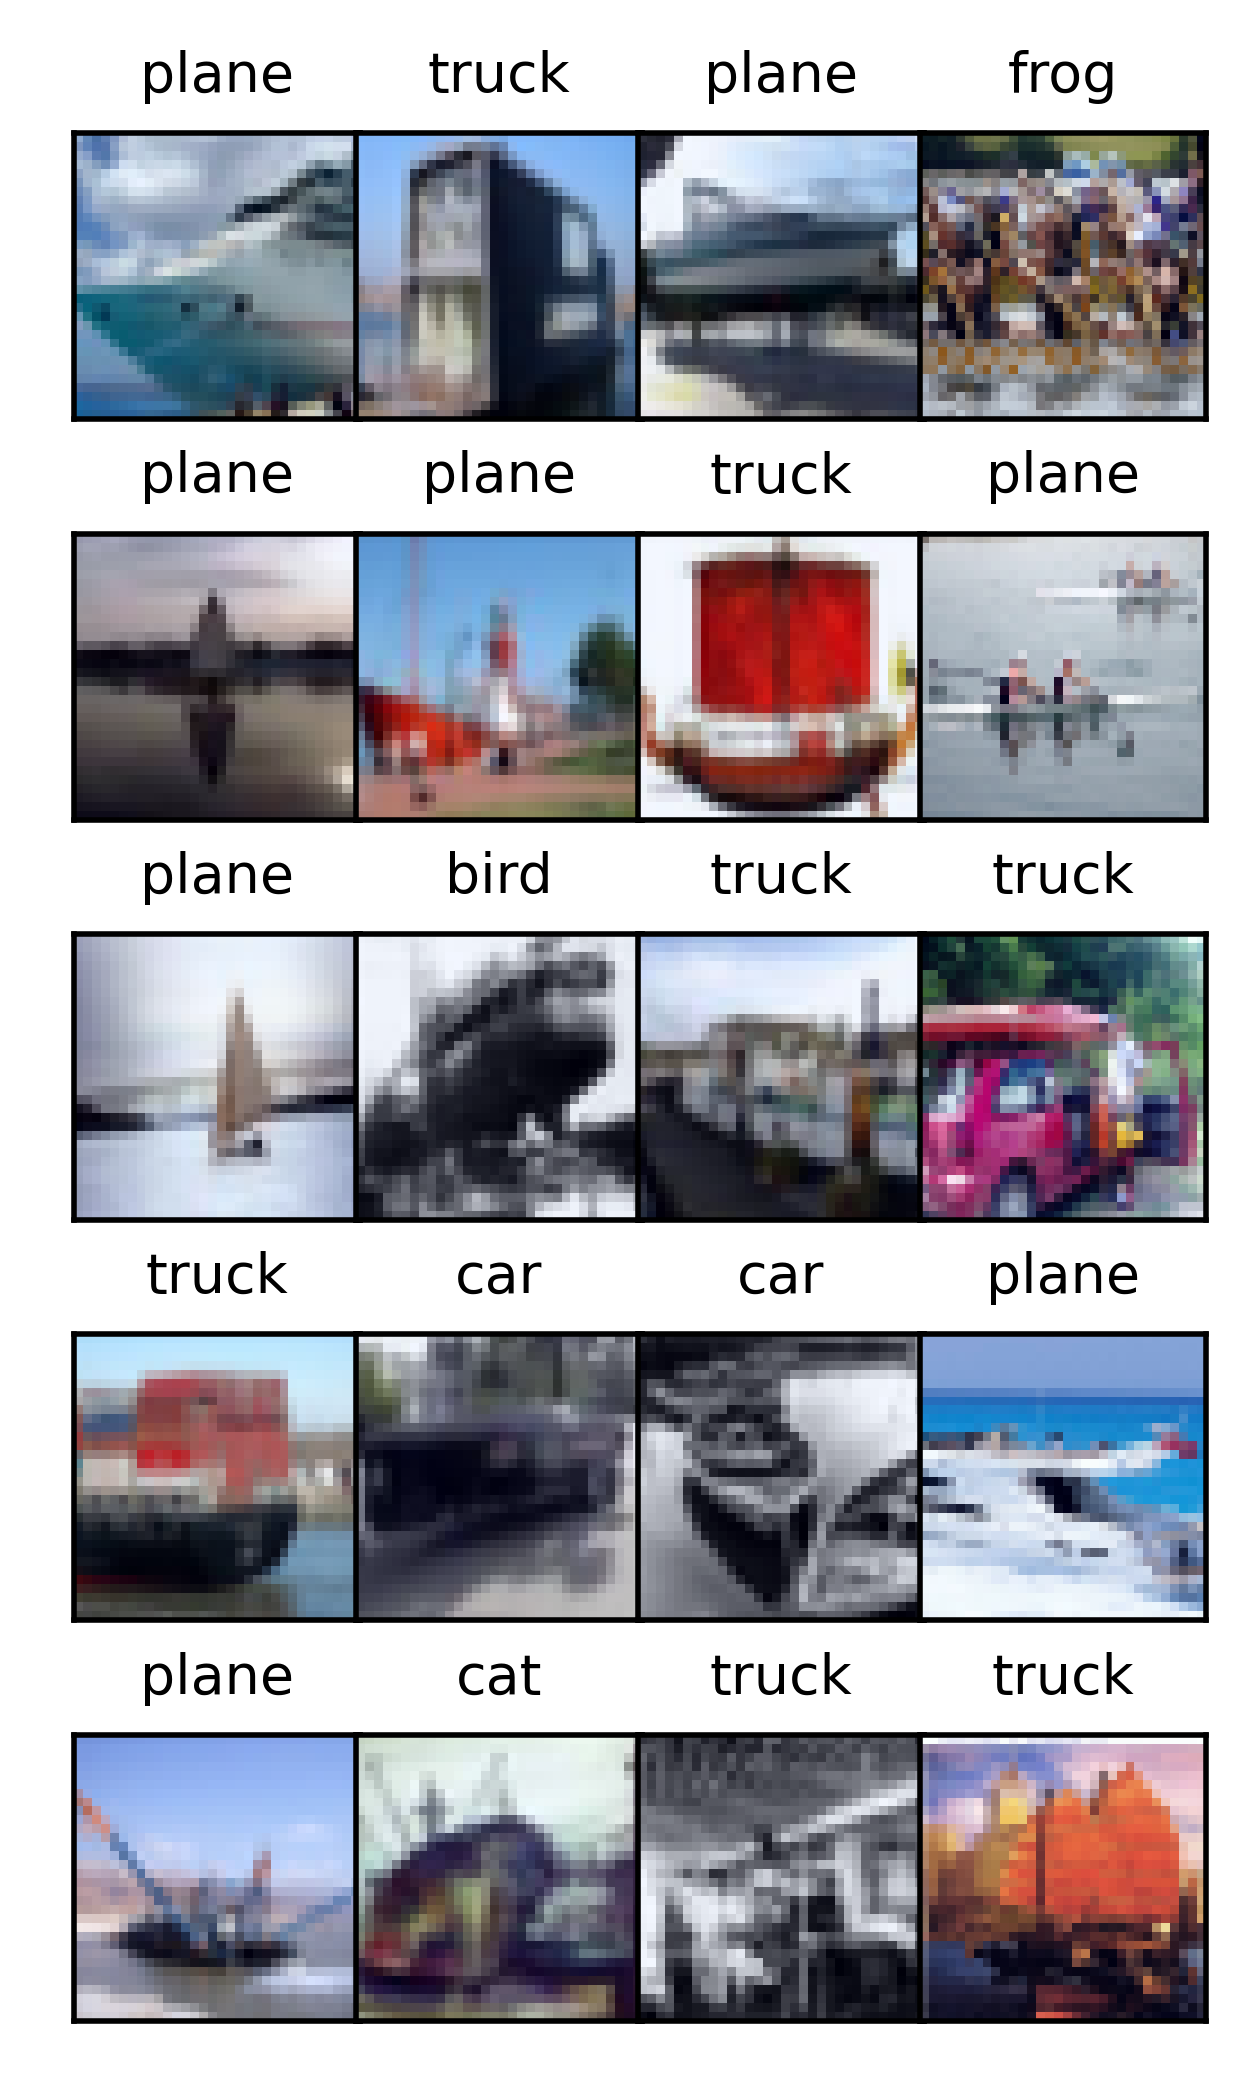} \\
    \textbf{ {\scriptsize Truck \hspace{3cm} Car \hspace{2.5cm} Plane \hspace{3cm} Ship}} \\ \vspace{0.25cm}
    \includegraphics[width=0.24\textwidth]{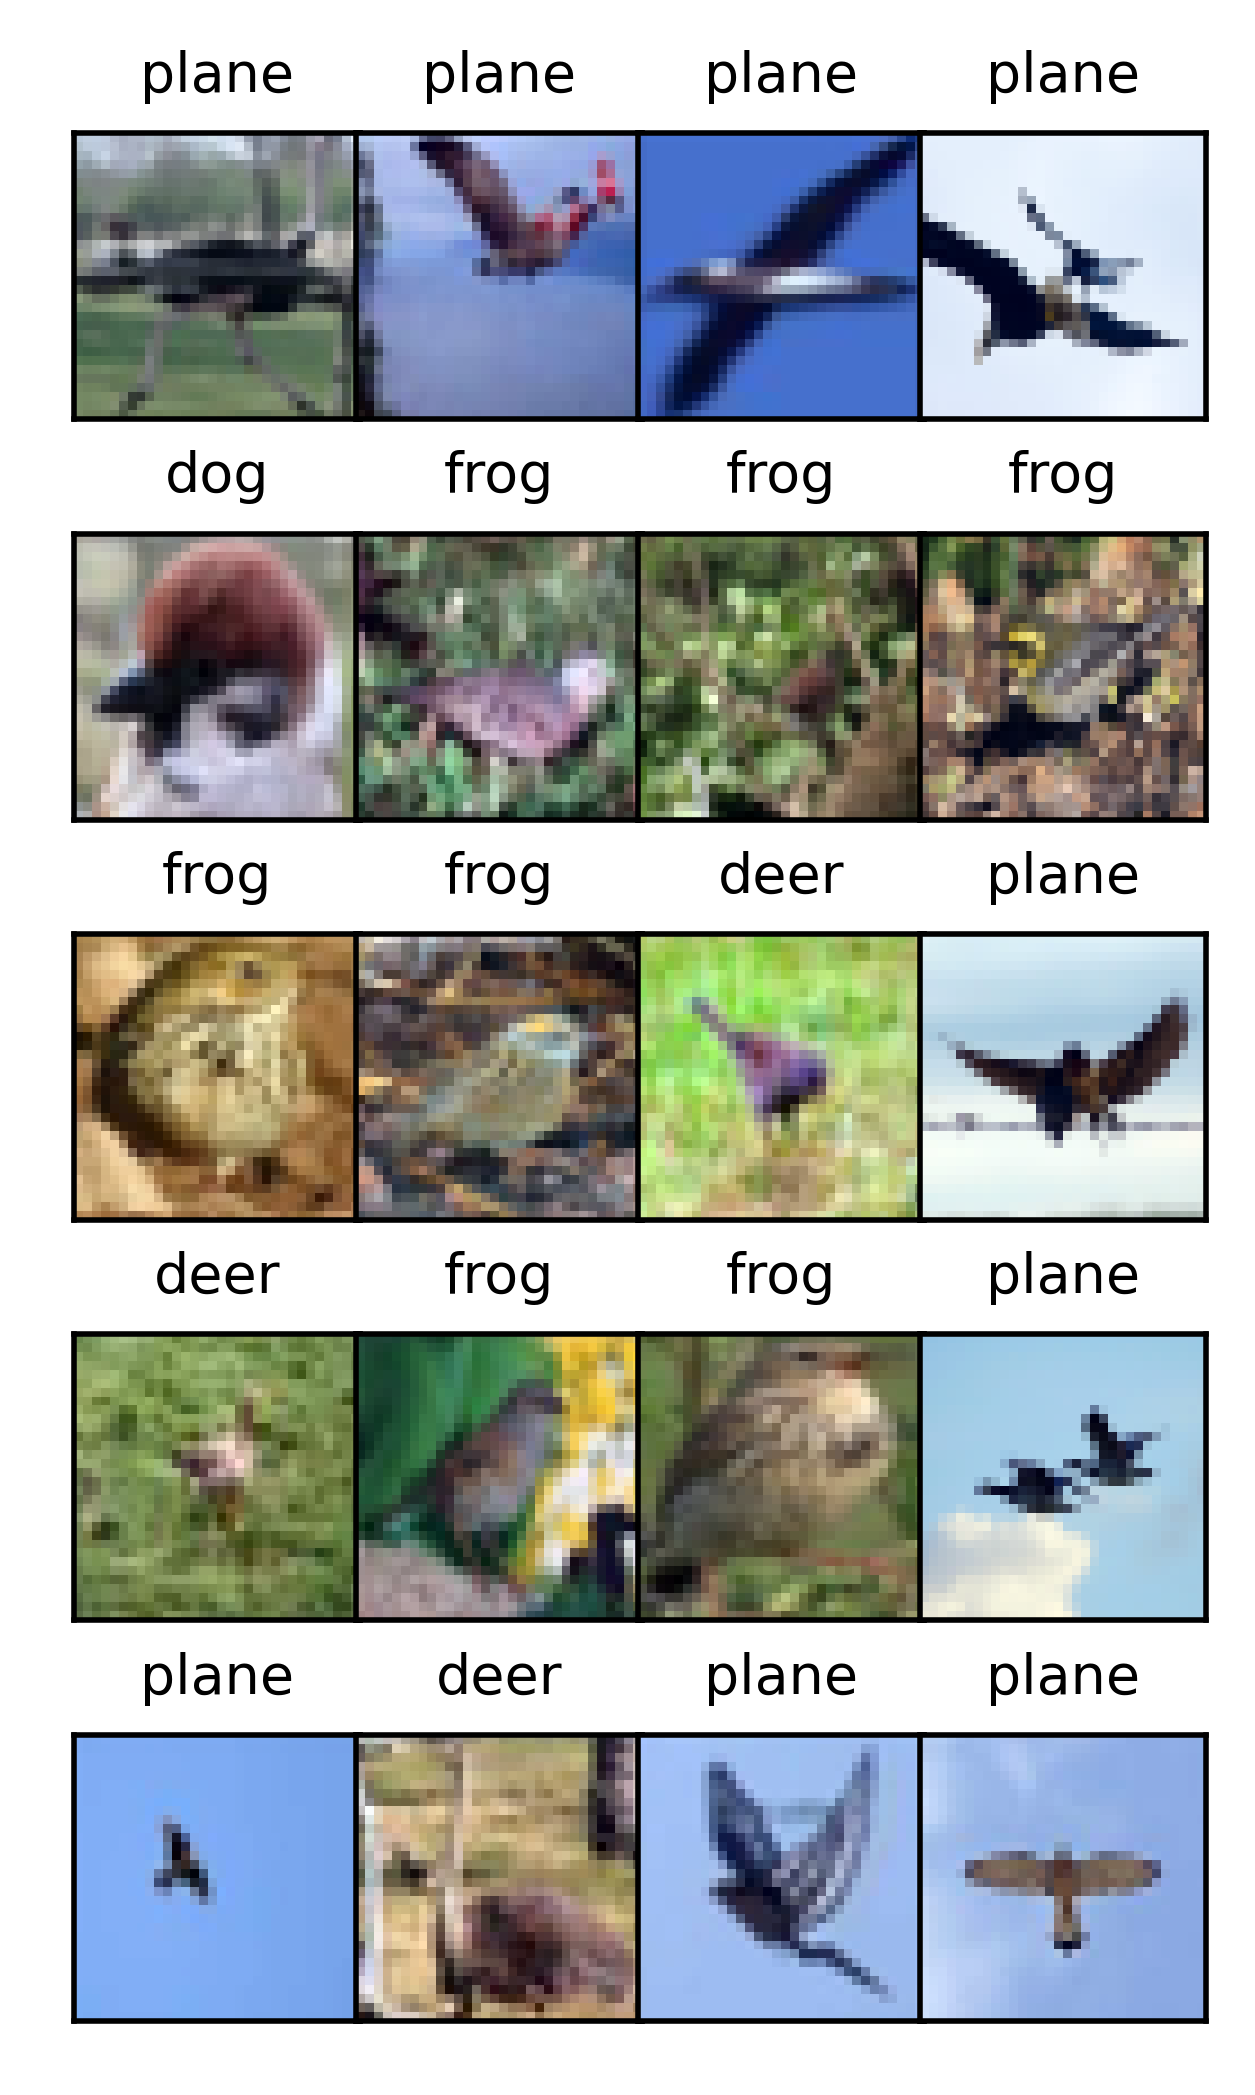}
    \includegraphics[width=0.24\textwidth]{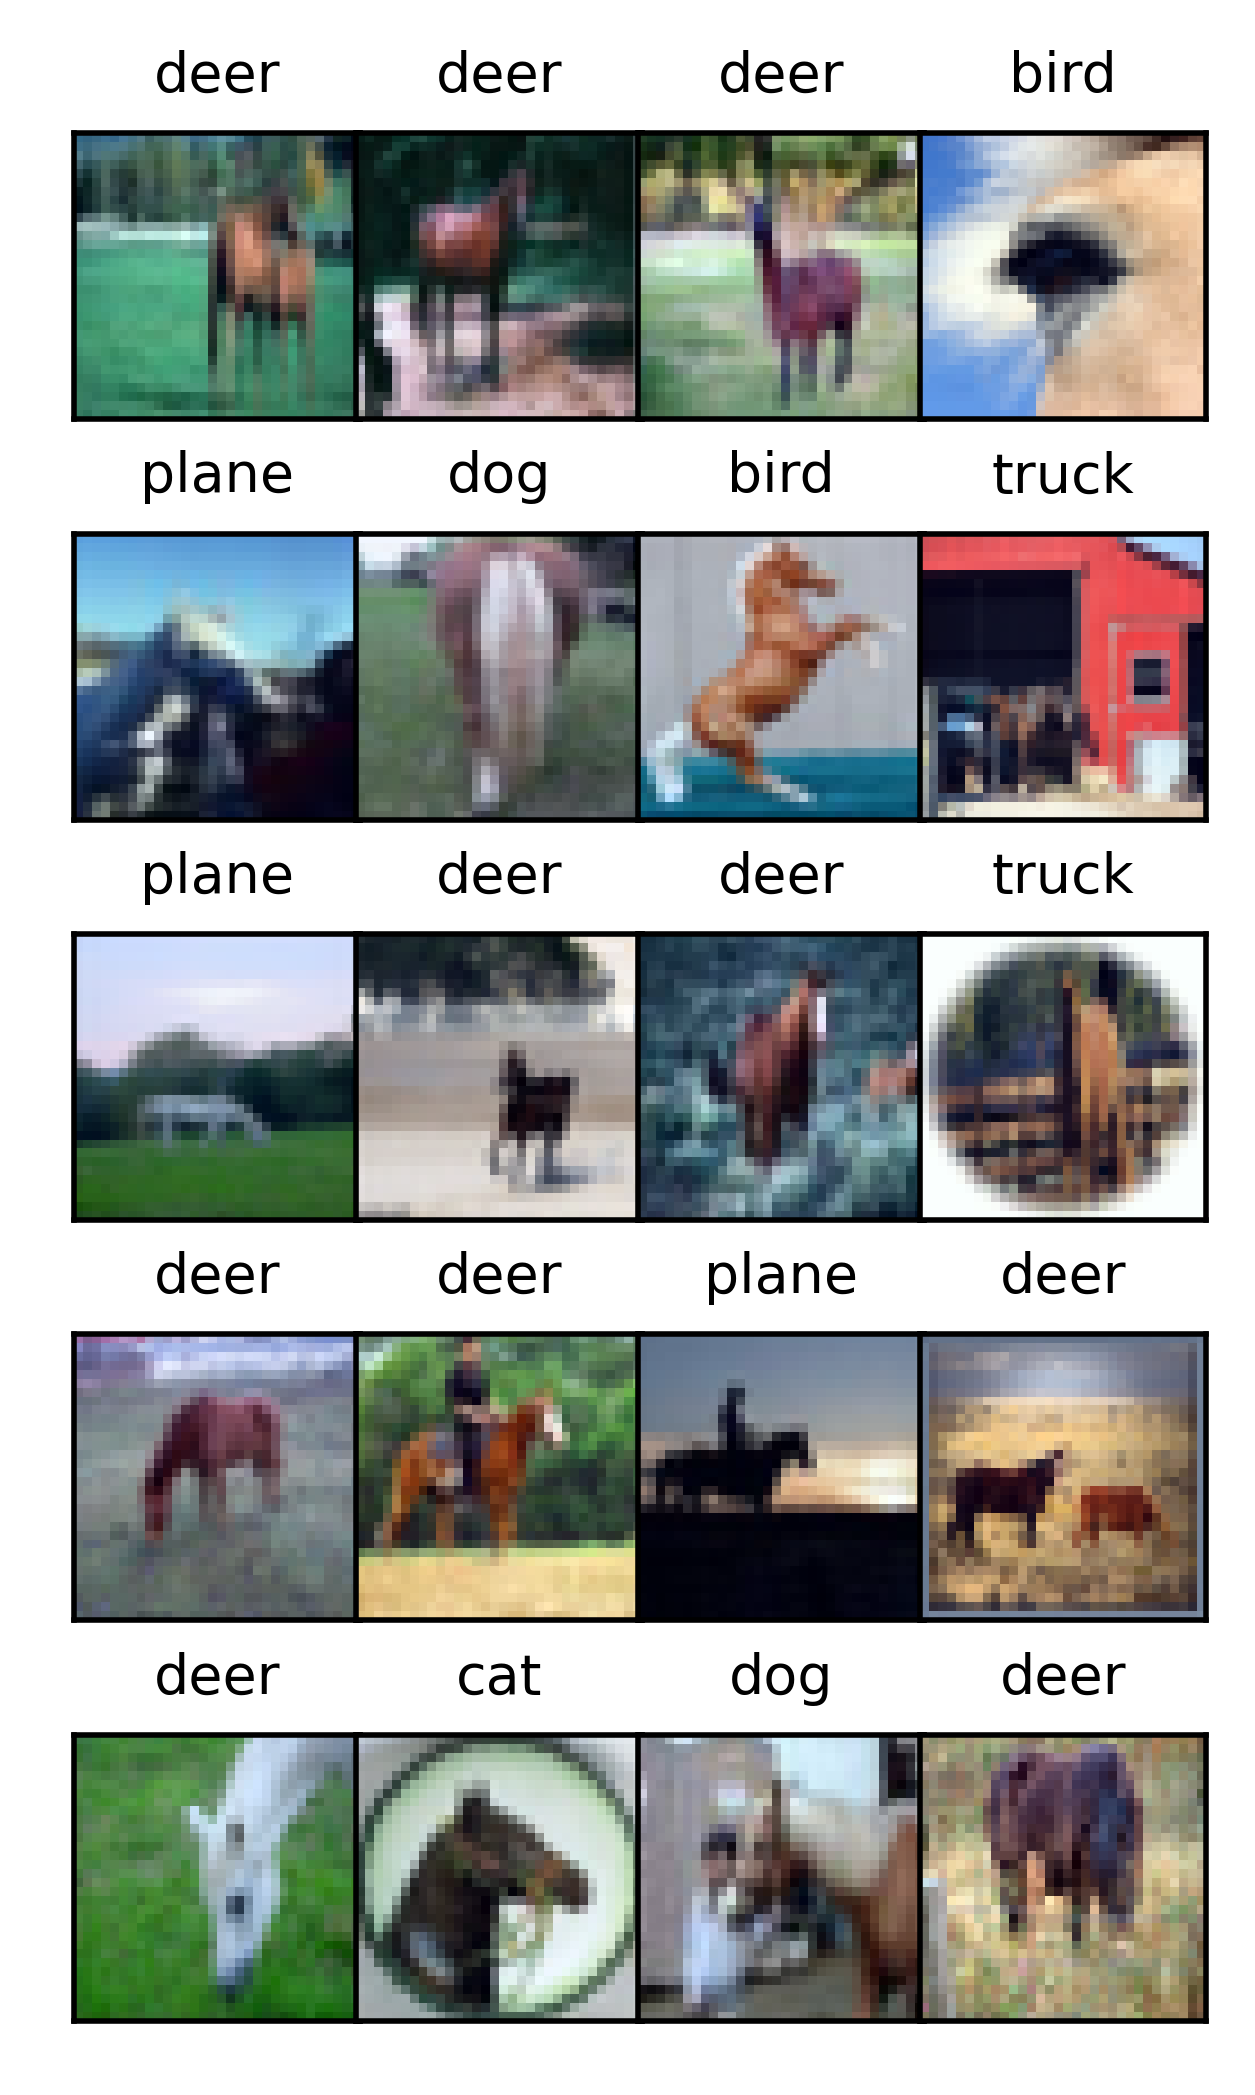} 
    \includegraphics[width=0.24\textwidth]{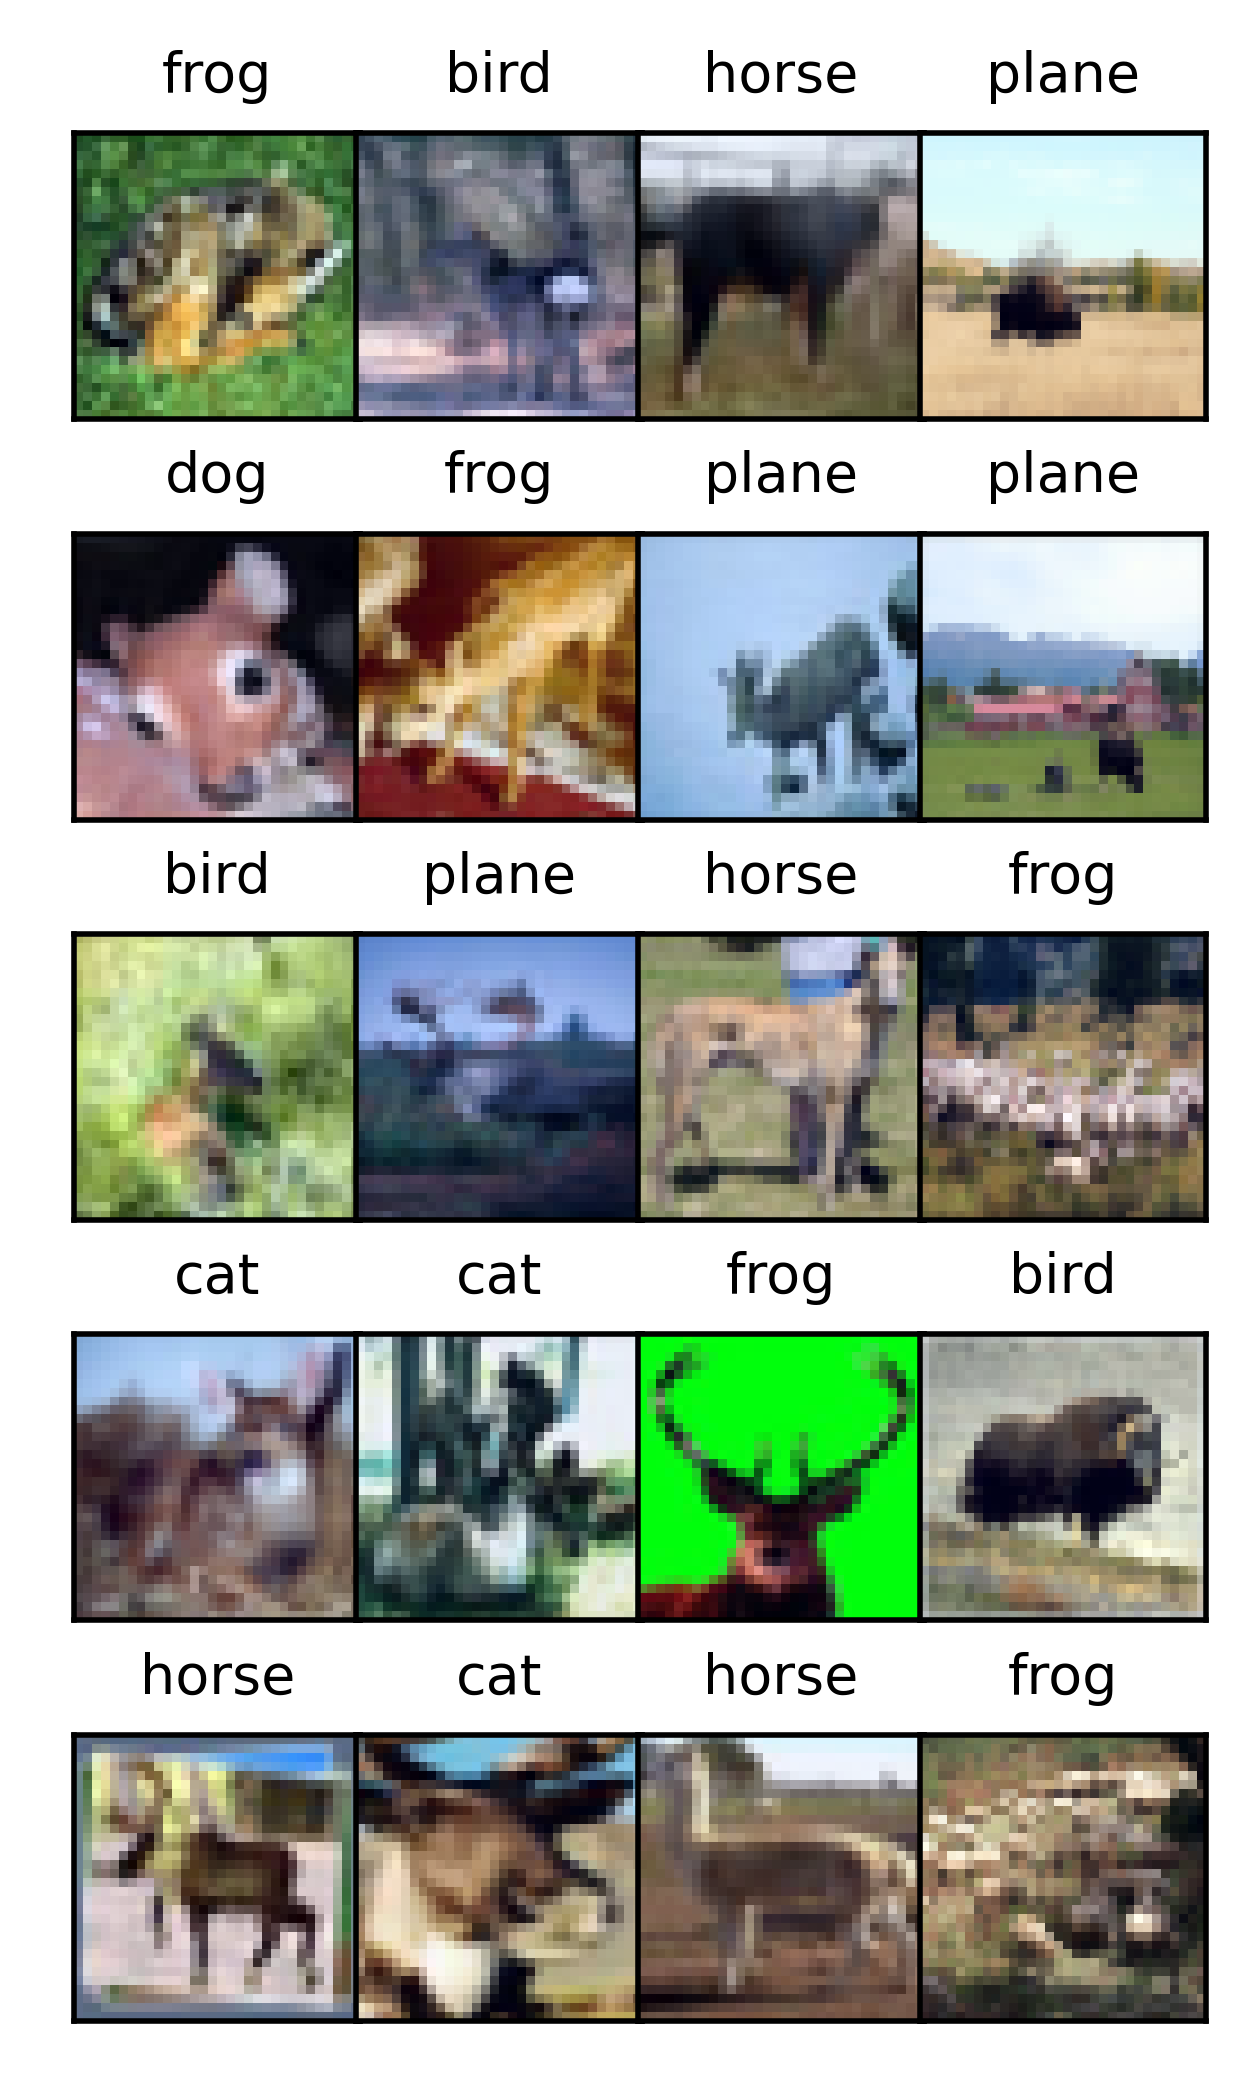} 
    \includegraphics[width=0.24\textwidth]{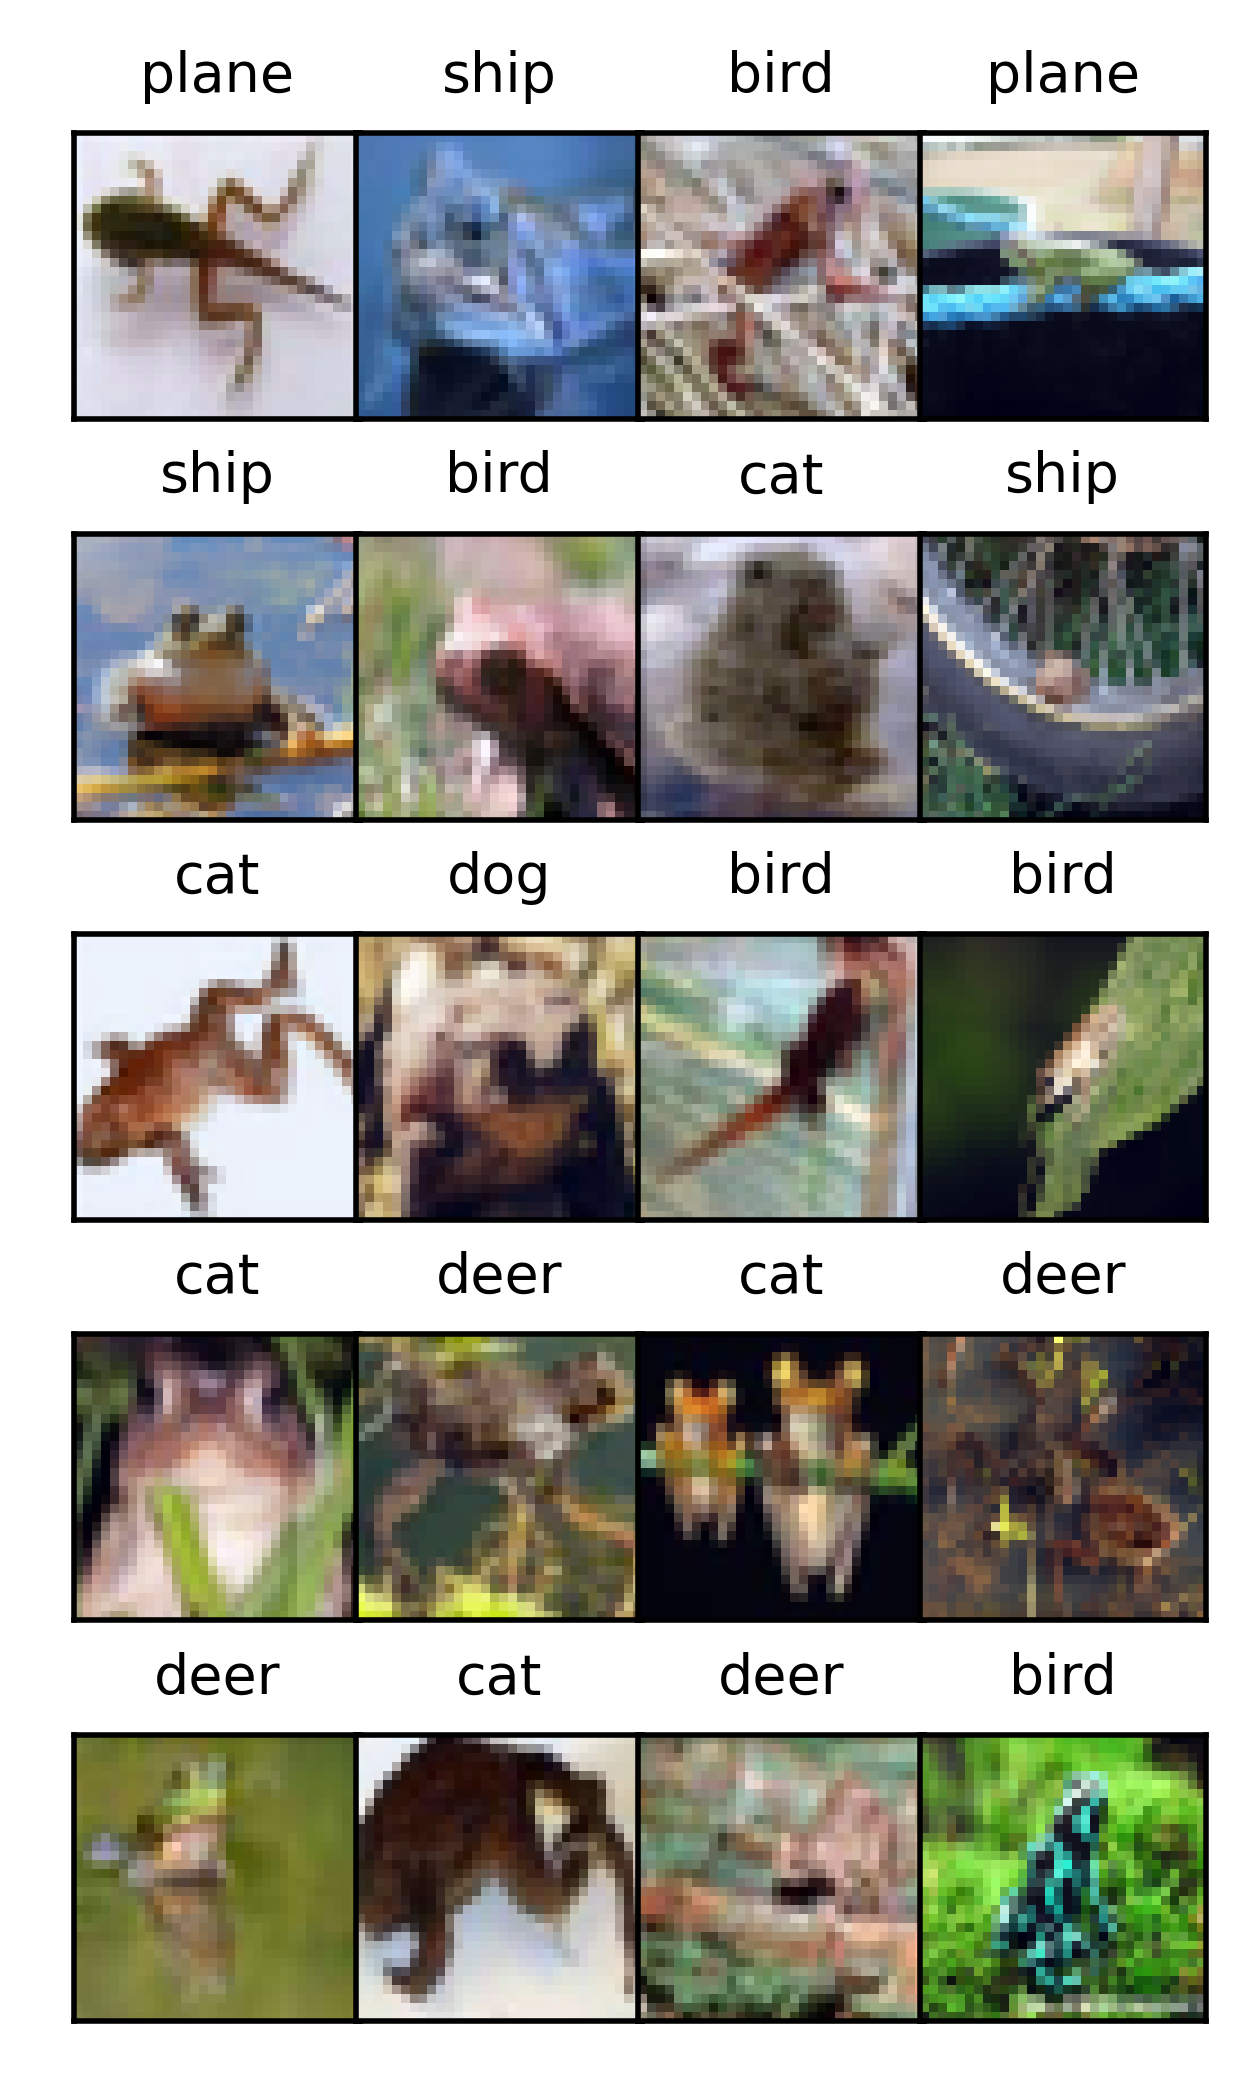} \\
    \textbf{ {\scriptsize Bird \hspace{3cm} Horse \hspace{2.5cm} Deer \hspace{3cm} Frog}} \\ \vspace{0.25cm}
    \includegraphics[width=0.24\textwidth]{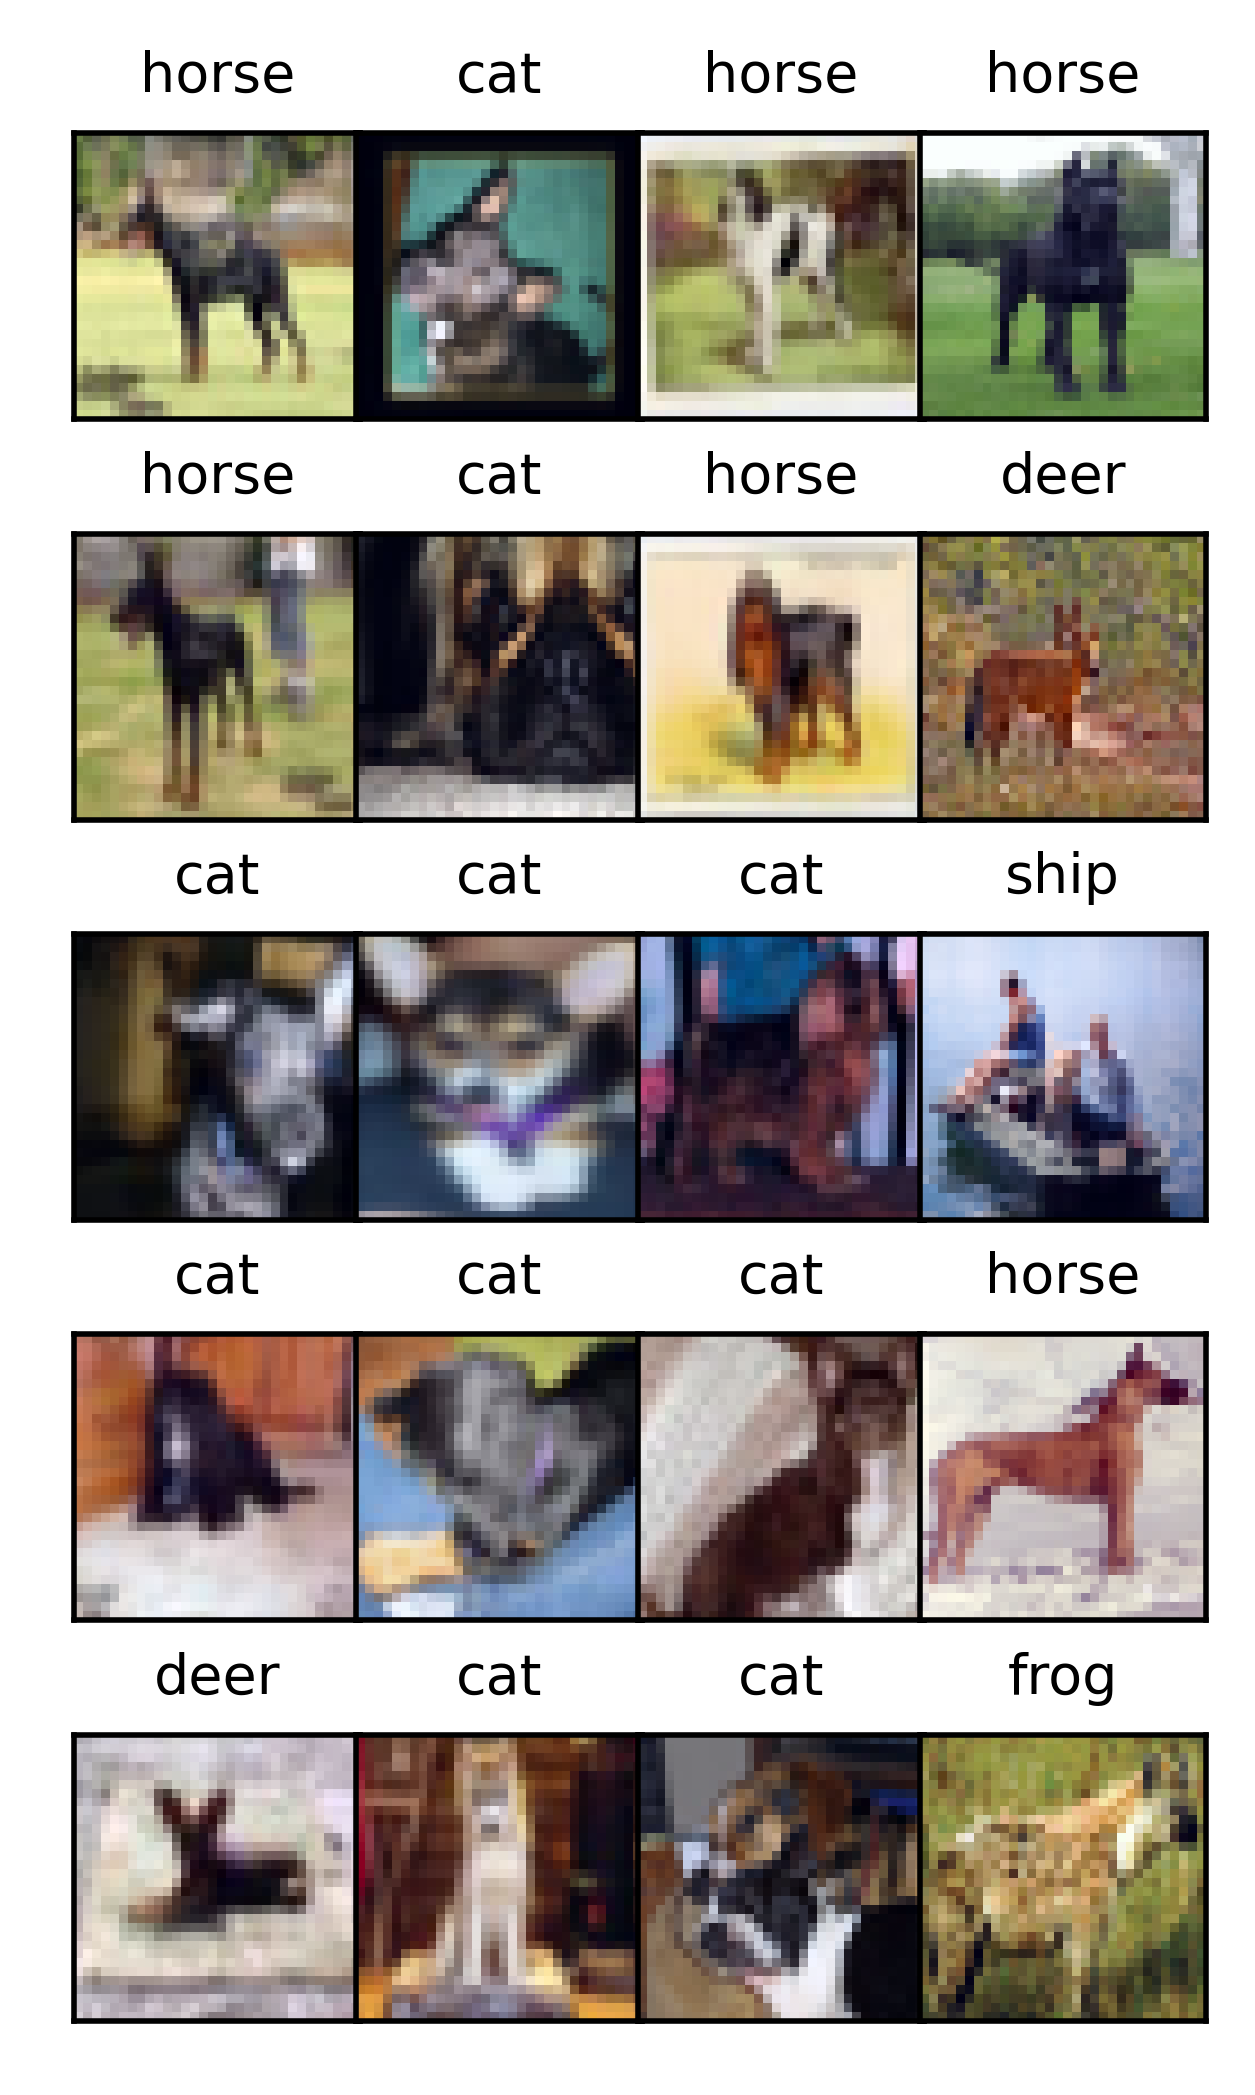} 
    \includegraphics[width=0.24\textwidth]{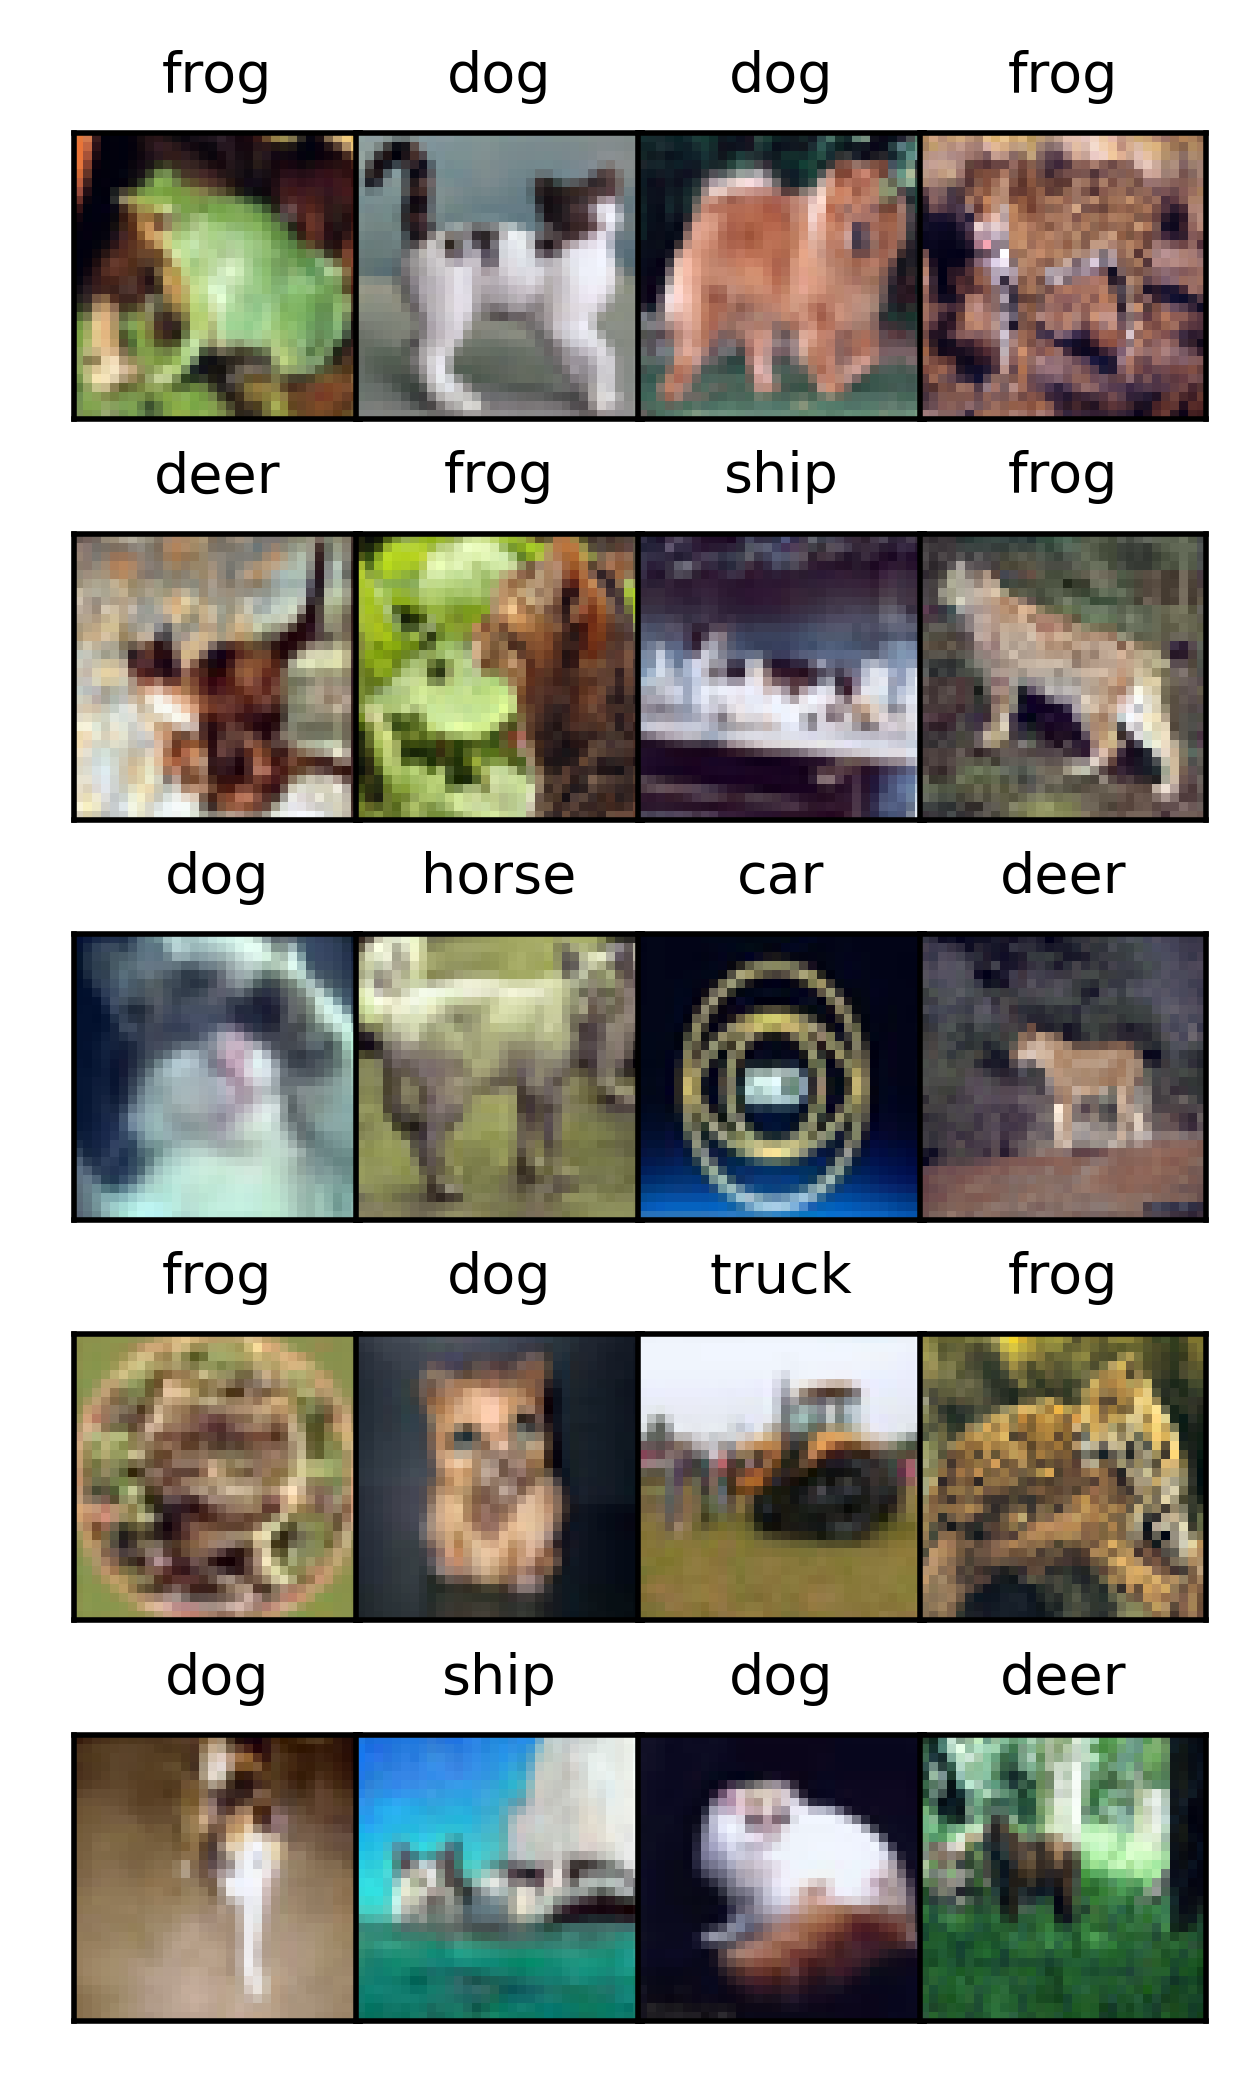} \\
    \textbf{{\scriptsize Dog \hspace{2.5cm} Cat}}
   \end{center}
  \vspace{-0.3cm}
  \caption{\label{fig:sp-corr-app} Spurious correlations per image.}
\end{figure}

\section{Colored MNIST experiments}

We have corrupted $\%10$ of the training labels. 
We then colored $\%80$ of the class $0$ in red and $\%80$ of the class $1$ in green thus introduced spurious correlation between the class labels and the color following \cite{arjovsky2019invariant}. 
We first trained $40$ networks similar to LeNets with two convolutional layers and one following feedforward layer where we have $ w \in \{8,16,32,64\}$ filters in the first layer, $2w$ filters in the second layer, and a feedforward layer that maps to class probabilities at the end ($10$ seed for each architecture). 
We calculated the entropy scores using the average of the first 100 epochs for one in-distribution and two OOD datasets. 
Calculating the confusion score distributions based on these networks, we find:

\begin{figure}[t!]
   \begin{center}
    \includegraphics[width=0.9\textwidth]{figs/01-cmnist-entrop-splits.png} 
   \end{center}
  \vspace{-0.3cm}
  \caption{\label{fig:cmnist-entropies}}
 \end{figure}
 
In ood1, all low entropy samples are from class 1 and in ood2, all low entropy samples are from class 0!

tested trained networks on this datasets in two domains: (1) ood1 where all digits are green, and (2) ood2 where all digits are red.

\section{The accuracy line's slope depends the difficulty of the OOD dataset but the confidences do not}

\begin{figure}[t!]
   \begin{center}
    \includegraphics[width=0.7\textwidth]{figs/allnets4-accs.png} 
    \includegraphics[width=0.7\textwidth]{figs/allnets4-conf.png} 
   \end{center}
  \vspace{-0.3cm}
  \caption{\label{fig:no-aug-main} \textbf{ID-OOD accuracies of the feedforward nets (blue) vs. convolutional nets (red)}. Top row: accuracies, bottom row: confidences. Blue dots ($300$) represent feedforward networks with depths $[2,3,4]$, with widths $[2,4,8, \ldots, 1024]$ at each layer, and $ 10 $ random seeds for each architecture. 
  Horizontal and vertical lines represent $\pm2$ standard deviations calculated for the fixed-size model with $10$ runs and dots represent the mean accuracy. 
  Dark blue dots ($30$) represent ensembles over $ 10 $ random seeds for the same architecture. Red dots ($140$) represent convolutional networks with 2 convolutional layers with filter numbers $[2, 4, \ldots, 128]$ in the first layer and doubled number of filters in the second layer, followed by either one or three layers of feedforward connections; each architecture has $ 10 $ seeds. 
  Dark red dots ($14$) represent the ensembles over the same architecture. All networks are trained on normalized CIFAR10 training data without further data augmentation.}%$R^2$ coefficients are: (1) for CIFAR-10.1 feedforward fit:0.975, conv fit: 0.978; (2) for CIFAR-10.2 feedforward fit:0.979, conv fit: 0.980; (3) for CINIC-10 feedforward fit:0.990, conv fit: 0.983. The two lines merge into one line in the probit scale.} 
 \end{figure}
 
 In this section, we evaluate $300$ feedforward networks and $140$ convnets on CIFAR-10, CIFAR-10.1 \citep{recht2019imagenet}, CIFAR-10.2 \citep{lu2020harder}, and CINIC-10 \citep{darlow2018cinic} datasets based on two metrics: accuracy and average confidences (see Fig~\ref{fig:no-aug-main}). In our testbed, we consider the scaling of the same model families and consider a fixed training dataset (w/o data augmentation) to study the effect of overparameterization unlike similar studies in literature where (1) several type of architectures are considered and (2) several training data modalities are considered such as pretraining on ImageNet or on JFT, or simply expanding the training dataset using augmentation.
 
 Strikingly, we observe that two model families follow two separate lines with different slopes when presented in the linear scale. When presented in the logit scale, we lose the fine resolution and the two families fall on the same line. For the CINIC-10 dataset, we observe that the two lines approach each other. Moreover, we observe that the average confidences follow a slope $ 1 $ which suggests that it solely comes from the model complexity rather than an intrinsic data property.

\section{Easy/Medium/Hard subpopulation split}

For the original Lenet family we considered ($70$  networks), we bucket the images into $71$ groups where bucket $ k $ contains the images that are correctly classified by $ k $ networks. Then we combine the images that are correctly classified by less than $1/3$-rd of the networks in the hard subpopulation, the images that are correctly classified by more than $2/3$-rd networks in the easy subpopulation, and the rest in the medium subpopulation. We find that both ID and OOD datasets contain very similar easy/medium/hard subpopulations in the sense that both underparameterized and overparameterized network achieve almost identical accuracies on these subpopulations (see Figure \ref{fig:subpops-OOD}). 

\textbf{A candidate model for the collinearity [incomplete].}
Let $ \acc^{(i)}(\alpha) \in (0,1)$ be the accuracy on a test dataset (ID or OOD) where $ \alpha \in [0,1]$ denote the model complexity, i.e. $0$ represents the worst model and $1$ represents the best; and $i \in \{0,1,2,3\}$ denotes the test dataset index (CIFAR-10, CIFAR-10.1, CIFAR-10.2, CINIC-10 respectively). 
Let $\min\acc_{\easy}$ be the minimum accuracy achieved by the model family considered (i.e. LeNets) and let $  s_{\easy} $ be the constant that modulates the accuracy depending on the model complexity such that the accuracy of the model with complexity $ \alpha $ on the easy subpopulation is $\min\acc_{\easy} + \alpha s_{\easy}  $. Same for the medium subpopulation, i.e. the accuracy of the model with complexity $ \alpha$ is given by $\min\acc_{\med} + \alpha s_{\med} $. Finally we posit that the models make random guesses on the hard population.

\begin{figure}[t!]
    \centering
    \subfloat[Majority/Easy subpopulation]{
        \includegraphics[width=0.8\textwidth]{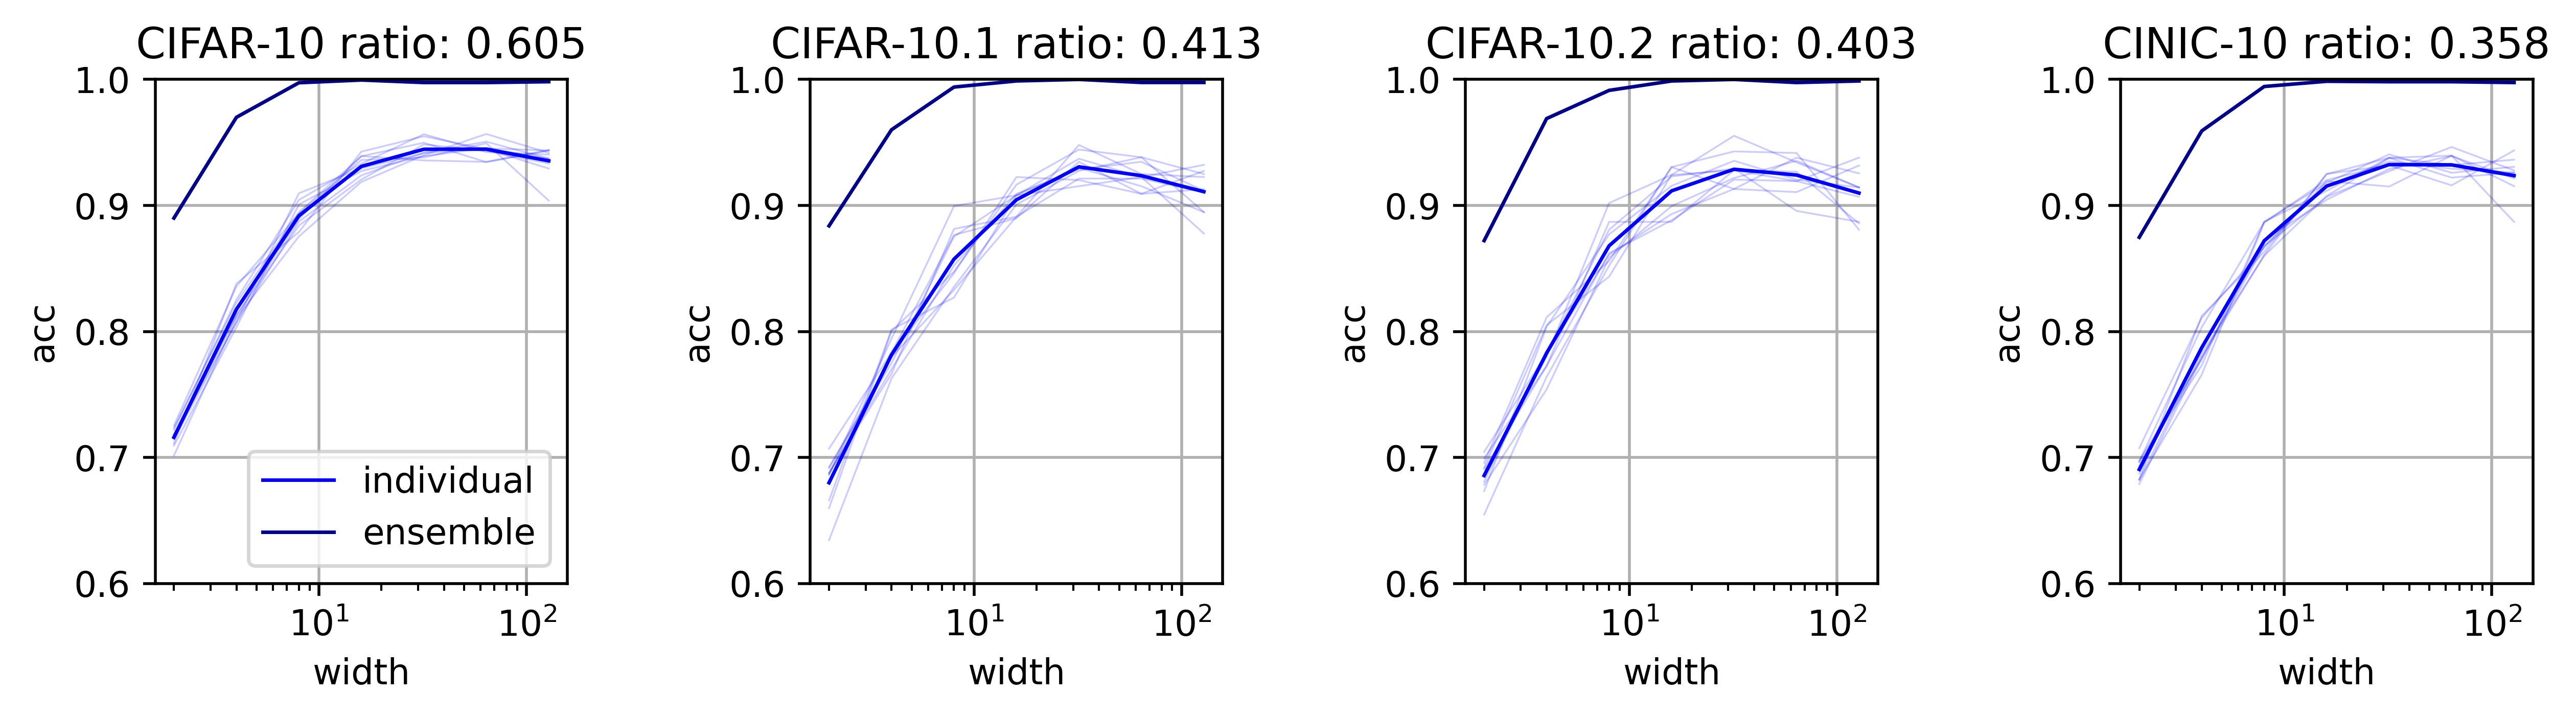}
        } \hfill
    \subfloat[Medium subpopulation]{
        \includegraphics[width=0.8\textwidth]{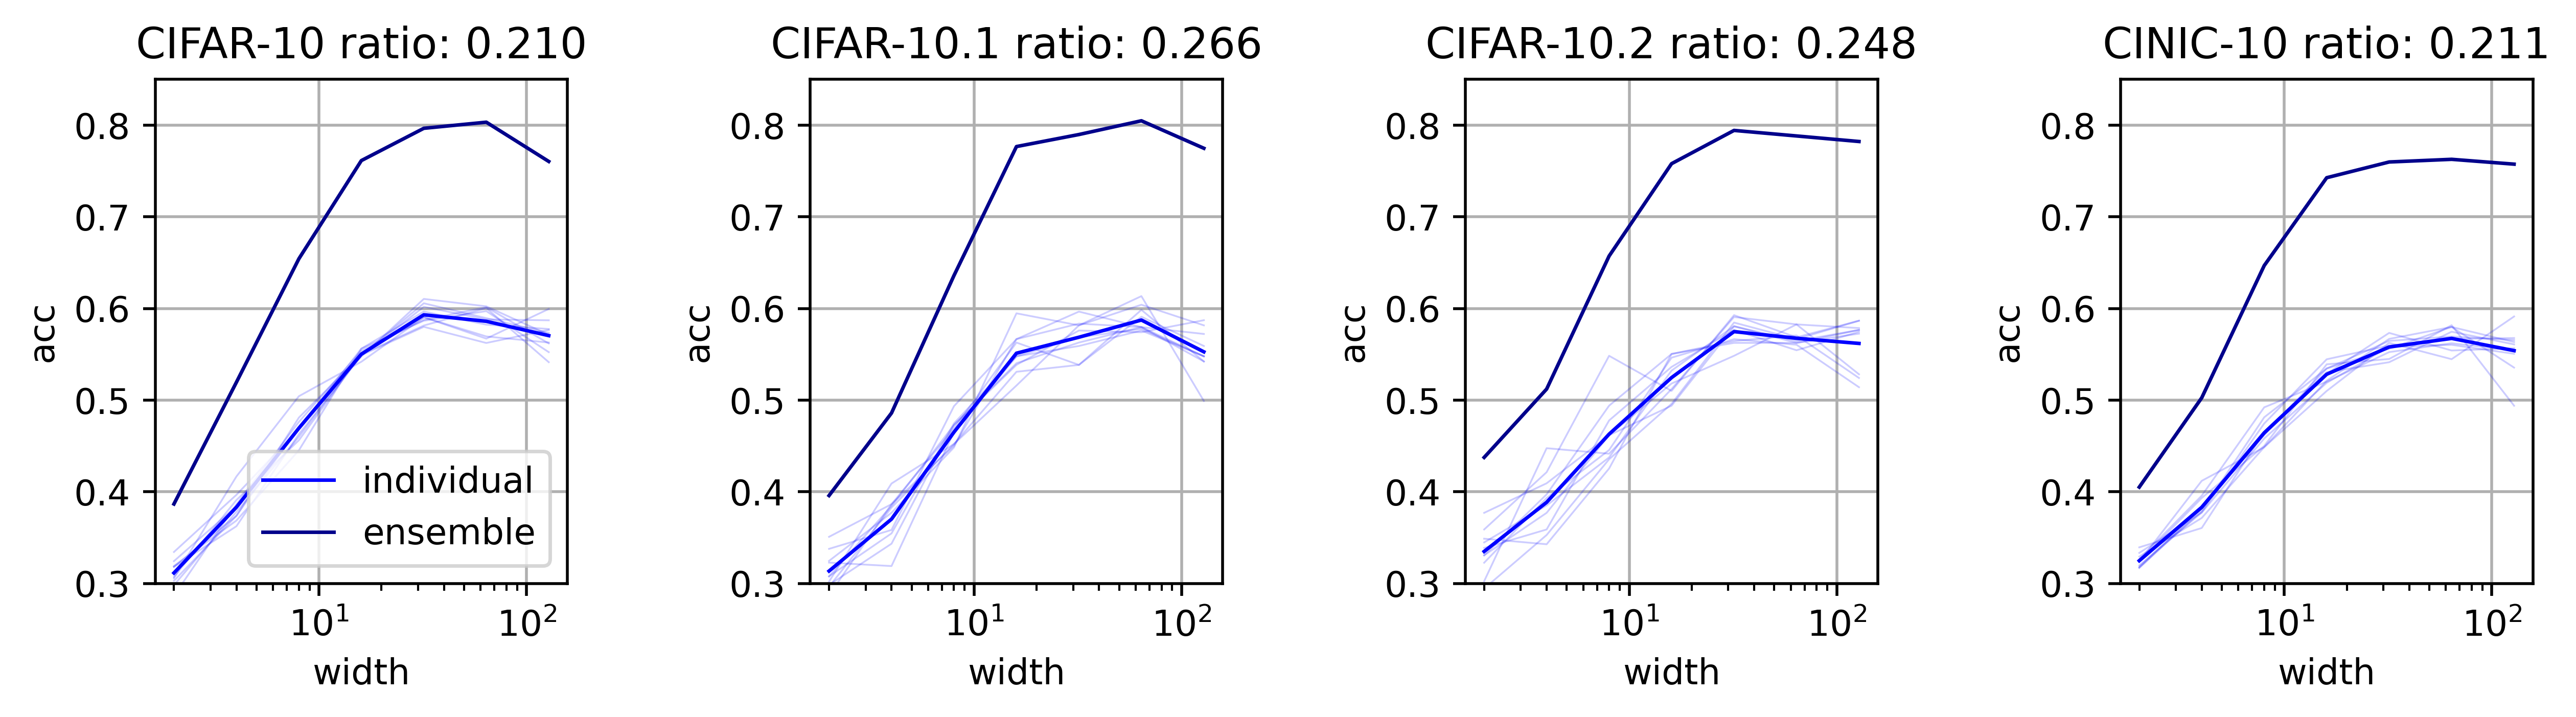}
        } \hfill
    \subfloat[Hard/Ambigious subpopulation]{
        \includegraphics[width=0.8\textwidth]{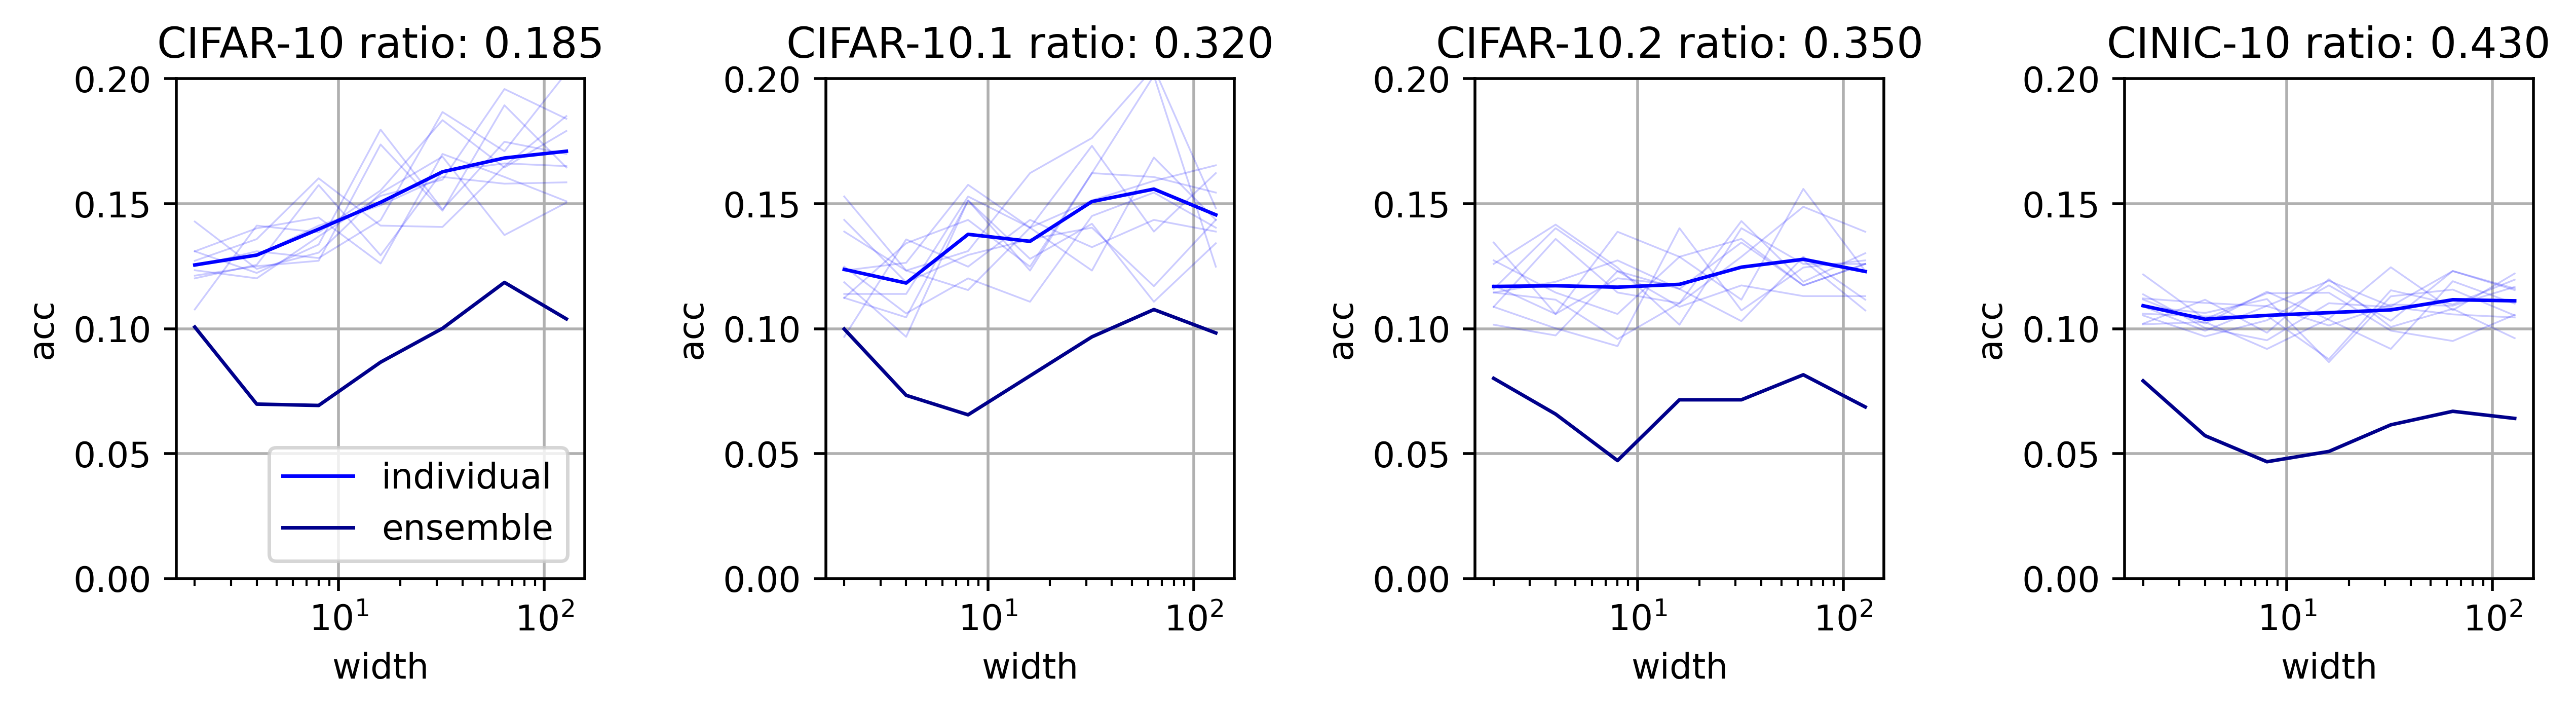}
        }
    \caption{\label{fig:subpops-OOD} \textbf{LeNet performances across subpopoulations of CIFAR-10 type ID and OOD datasets.} (split 1/3-1/3-1/3 by all LeNets with widths $2-128$). We observe that in each subpopulation, the networks achieve very similar accuracies. \textbf{First-row:} Typically the easy subpopulation makes up the biggest portion of the dataset (see the subpopulation ratios) therefore dominates the overall accuracy. \textbf{Second-row:} Underparameterized networks exhibit gradual improvement in medium subpopulation but overparameterized networks exhibit a drop in the accuracy. \textbf{Third-row:} In the hard subpopulation, the networks exhibit random guessing behavior (around $\%10$) and the networks perform pretty much the same independent of the network complexity.
    }
\end{figure}

%Ensembling seems to decrease the average confidence except for the peculiar super overfitting feedforward networks -- which exhibit average confidence $1$.

These assumptions can be combined in the following equation:

\begin{align}
    \acc^{(i)}(\alpha) = \min\acc^{(i)} + \alpha s^{(i)} =  \rho_{\easy}^{(i)} (\min\acc_{\easy}+ \alpha s_{\easy}) + \rho_{\med}^{(i)}  (\min\acc_{\med} + \alpha s_{\med}) + \rho_{\hard}^{(i)} 0.1
\end{align}

Therefore for all datasets $ i \in \{0,1,2,3\} $, we have 
\begin{align}
    \min\acc^{(i)} &= \rho_{\easy}^{(i)} \min\acc_{\easy} + \rho_{\med}^{(i)} \min\acc_{\med} + \rho_{\hard}^{(i)} 0.1 \\
    s^{(i)} &= \rho_{\easy}^{(i)}  s_{\easy} +  \rho_{\med}^{(i)}  s_{\med}.
\end{align}

\section{An alternative way of splitting}

\begin{figure}[ht!]
    \centering
    \subfloat[Majority/Easy subpopulation]{
        \includegraphics[width=0.8\textwidth]{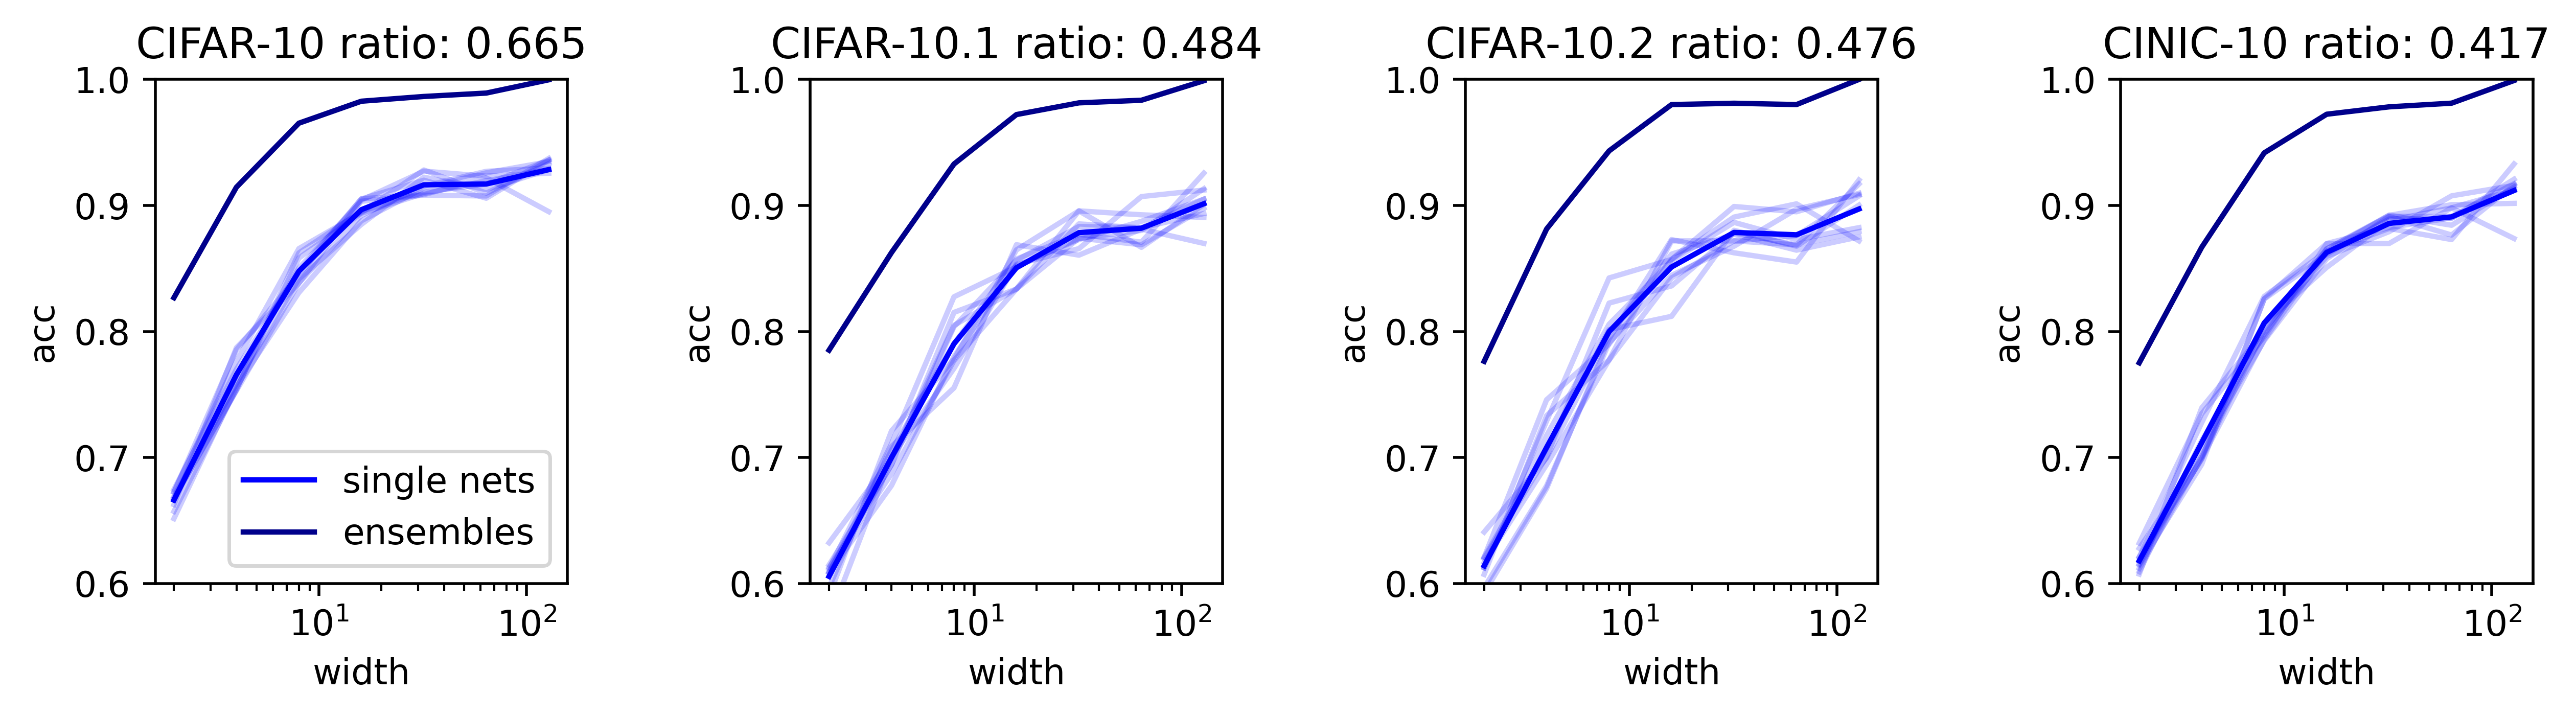}
        } \hfill
    \subfloat[Hard subpopulation]{
        \includegraphics[width=0.8\textwidth]{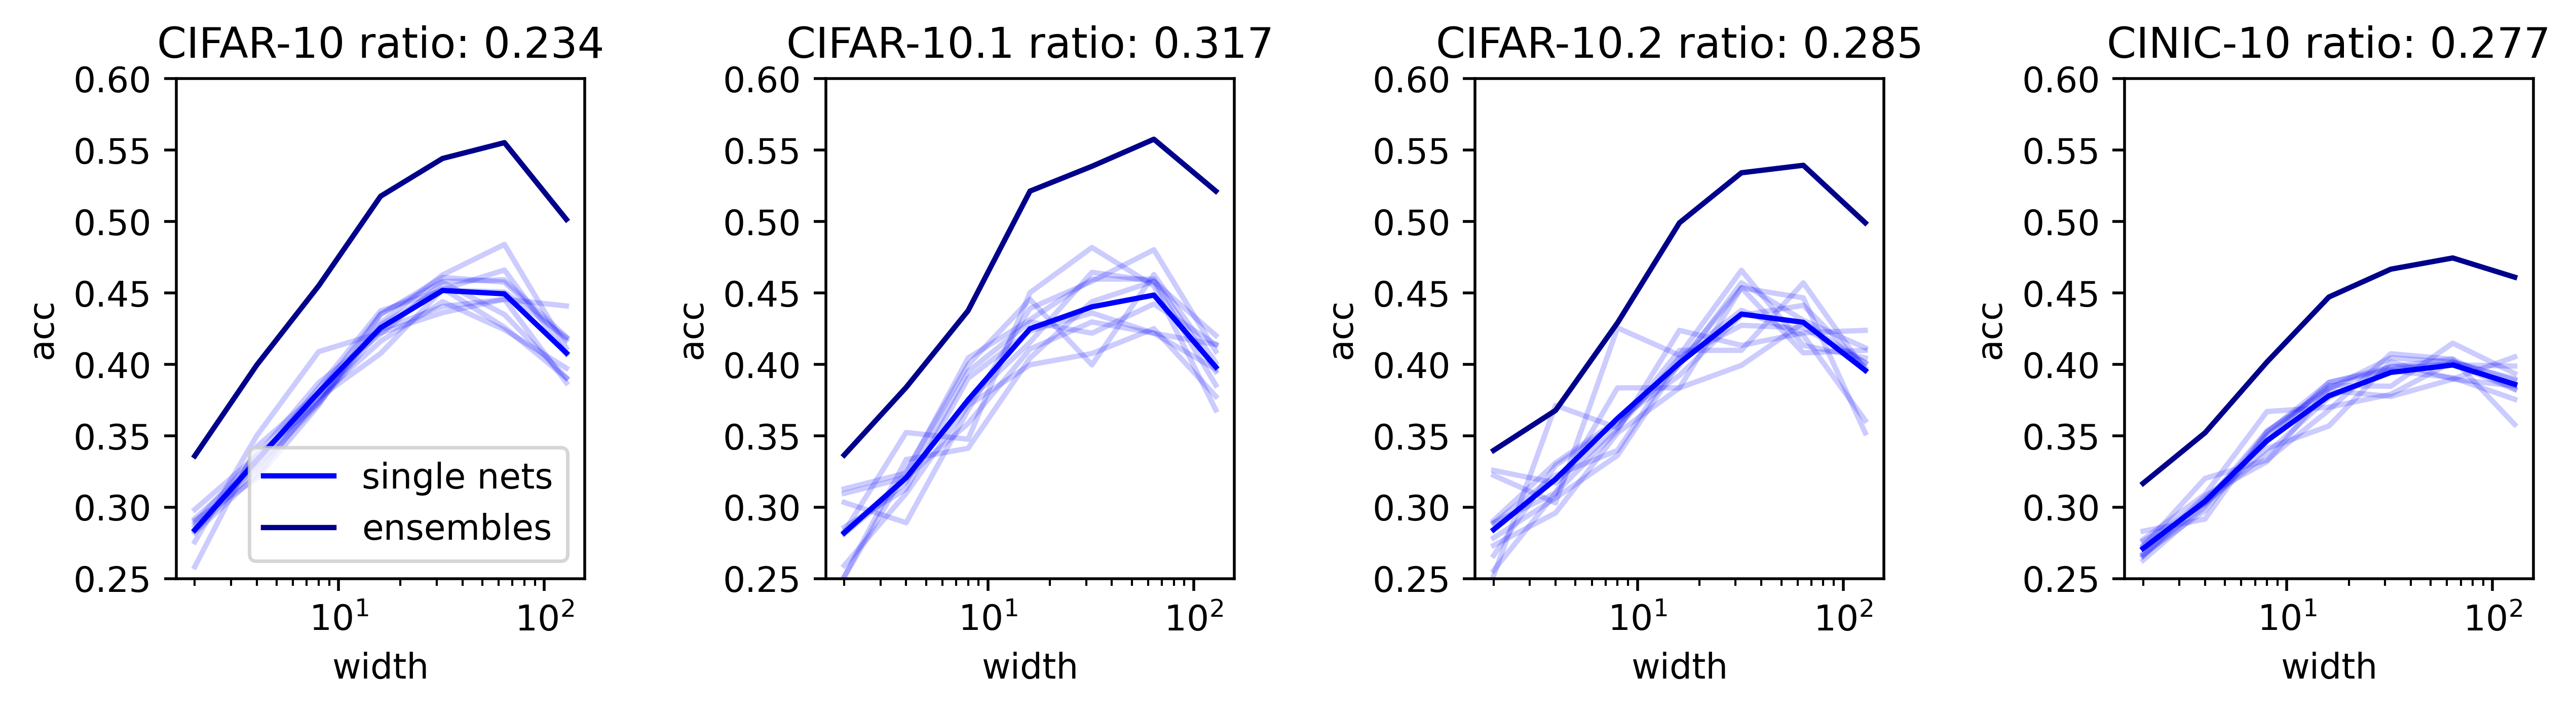}
        } \hfill
    \subfloat[Minority/Ambigious subpopulation]{
        \includegraphics[width=0.8\textwidth]{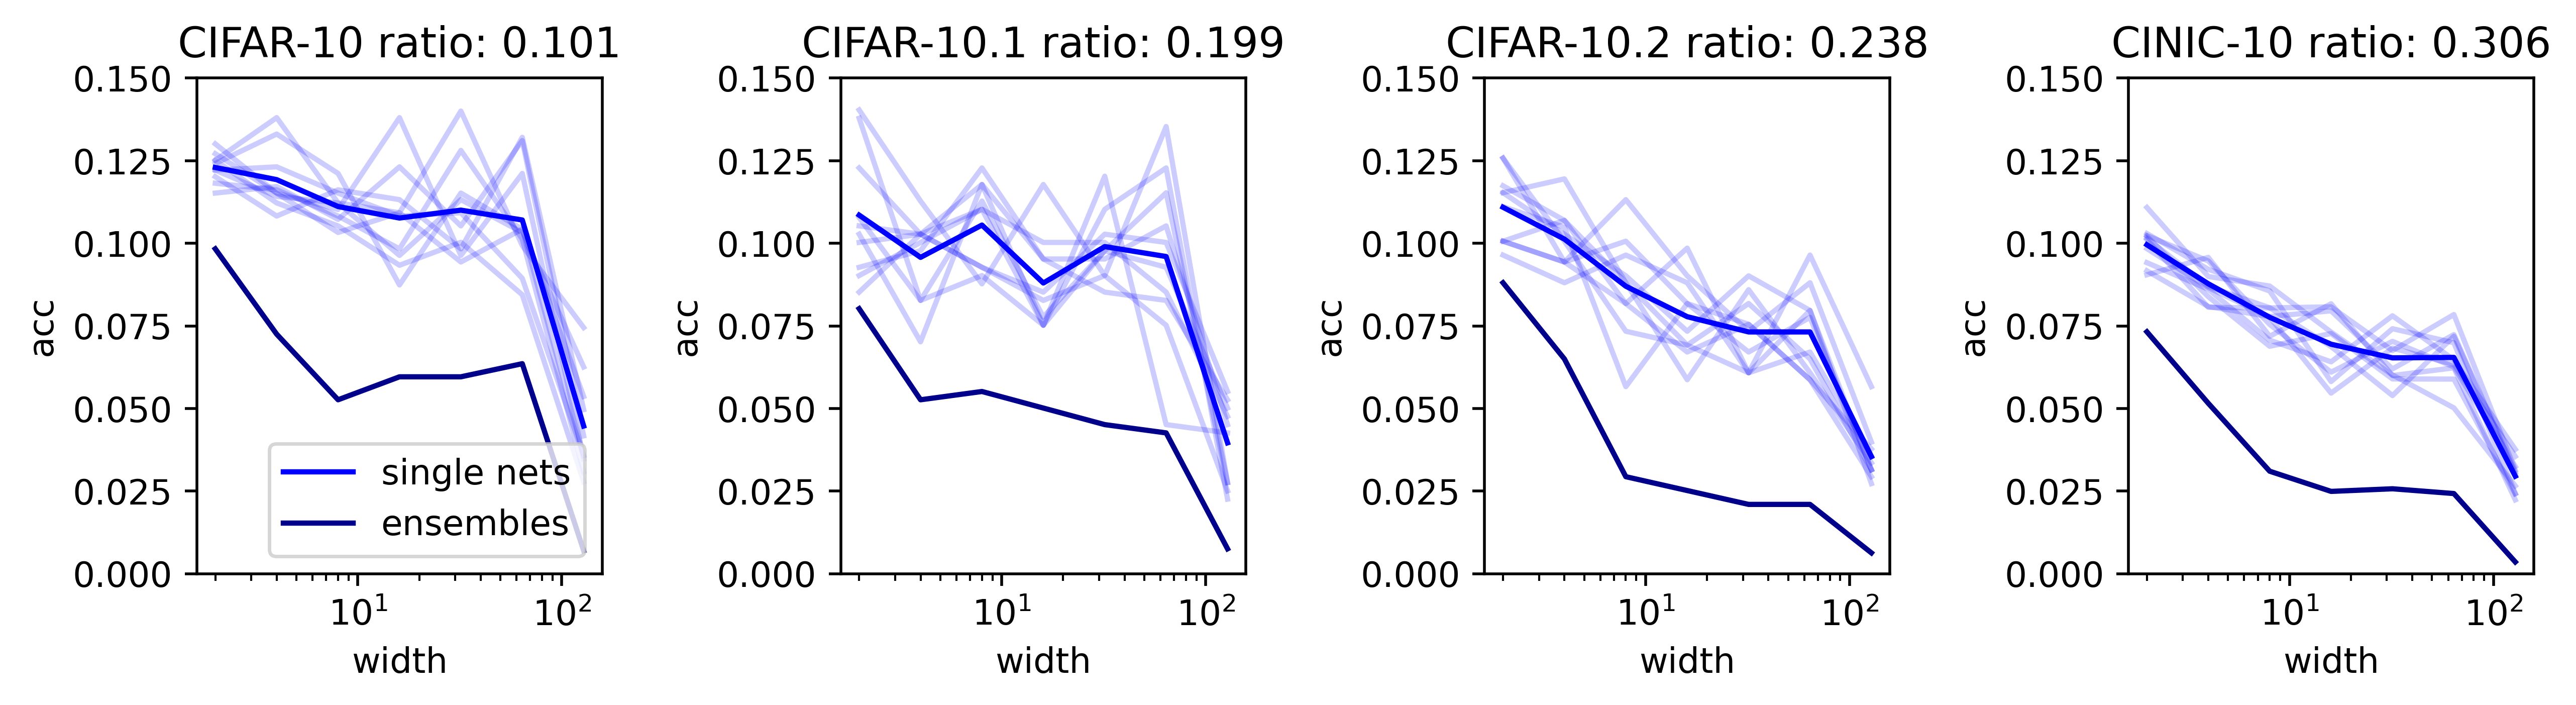}
        }
    \caption{\label{fig:subpops-OOD-2} \textbf{LeNet performances across subpopoulations of CIFAR-10 type ID and OOD datasets.} (split [0,1], [2,3,4,5,6], [7,8,9,10] by LeNet width 128) We observe that in each subpopulation, the networks achieve very similar accuracies. \textbf{First-row:} Typically the easy subpopulation makes up the biggest part of the dataset (see the subpopulation ratios) therefore dominates the overall accuracy too. \textbf{Second-row:} Underparameterized networks exhibit gradual improvement in minority groups but overparameterized networks exhibit a drop in the accuracy. \textbf{Third-row:} In the difficult subpopulation, the smallest networks exhibit random guessing behavior (around $\%10$) whereas overparameterization gradually decreases the accuracy down to $\%0$ in this subpopulation due to memorization/fitting in the spurious features.
    }
\end{figure}

\end{document}
